# Supplementary material for: Constraints on 3- and 4-loop $\beta$-functions in a general four-dimensional Quantum Field Theory
Source: arXiv:1906.04625 ancillary file (2019-08-27)
Supplement: Supplementary file 1 [file Ancillary_5-loops.pdf]

# Constraints on 3- and 4-loop $\beta$ -functions in a general four-dimensional Quantum Field Theory: Ancillary file

---

Colin Poole<sup>1</sup> and Anders Eller Thomsen<sup>2</sup>

CP<sup>3</sup>-Origins, University of Southern Denmark,  
Campusvej 55, DK-5230 Odense M, Denmark

|     |                                                   |    |
|-----|---------------------------------------------------|----|
| 1   | $\beta$ -function basis at 4–3–2 . . . . .        | 1  |
| 1.1 | Gauge $\beta$ -function . . . . .                 | 2  |
| 1.2 | Yukawa $\beta$ -function . . . . .                | 8  |
| 1.3 | Quartic $\beta$ -function . . . . .               | 17 |
| 2   | Consistency conditions at 4–3–2 . . . . .         | 18 |
| 2.1 | List of all CCs . . . . .                         | 18 |
| 2.2 | Extra conditions for symmetric $T_{IJ}$ . . . . . | 37 |
| 2.3 | Consistency conditions for $S$ . . . . .          | 40 |

---

In this ancillary file we provide the full list of 5-loop consistency conditions, save for the  $\gamma_5$  related contributions which are shown in the main paper. First we present the TSs making up the basis of the  $\overline{\text{MS}}$   $\beta$ -functions at order 4–3–2 in the graph notation explained in the paper. In the few places where the notation has a sign ambiguity we write out the contribution explicitly in tensor notation. Afterwards we present the full list of CCs at this order.

## 1 $\beta$ -function basis at 4–3–2

Here we present the TS basis for the  $\beta_{AB}^{(4)}$ ,  $\beta_{aij}^{(3)}$ , and  $\beta_{abcd}^{(2)}$ . The graphical notation is employed for the same reason as in the main article, and the few ambiguities that occur at order 4–3–2 are resolved using regular index notation.

---

<sup>1</sup>cpoole@cp3.sdu.dk

<sup>2</sup>aethomsen@cp3.sdu.dk

1.1 Gauge  $\beta$ -function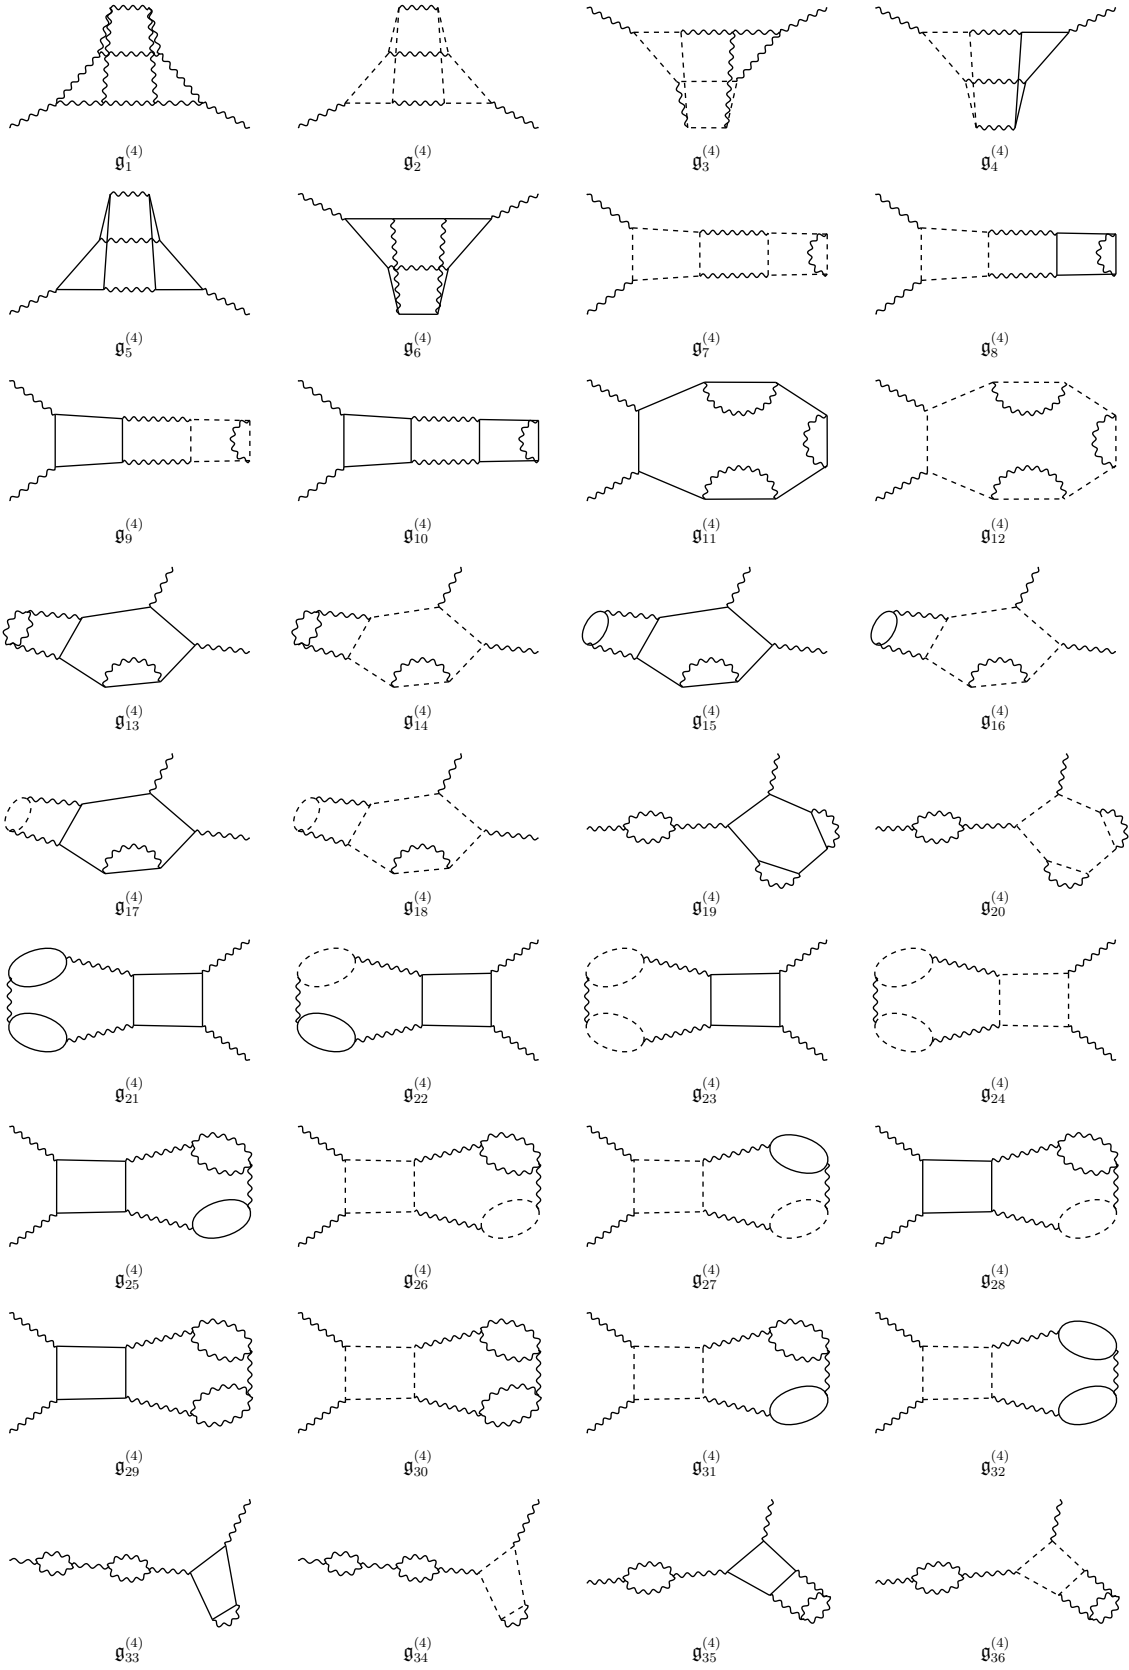

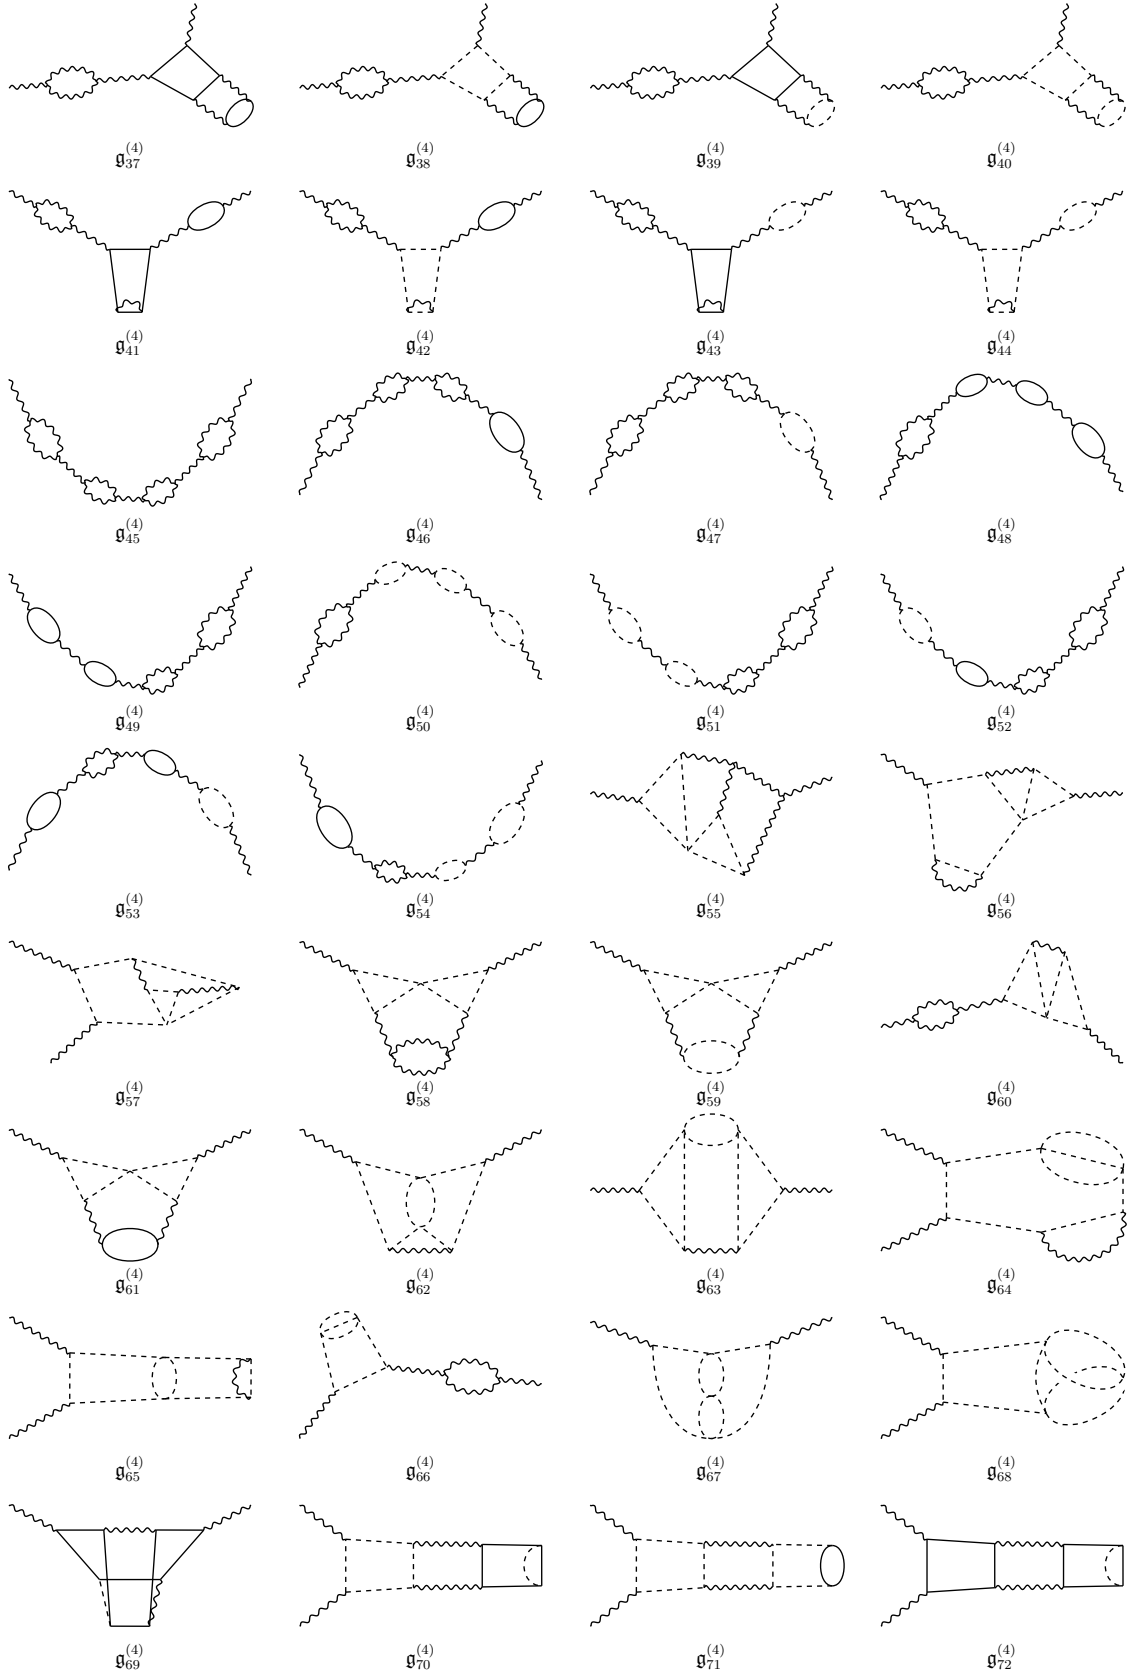

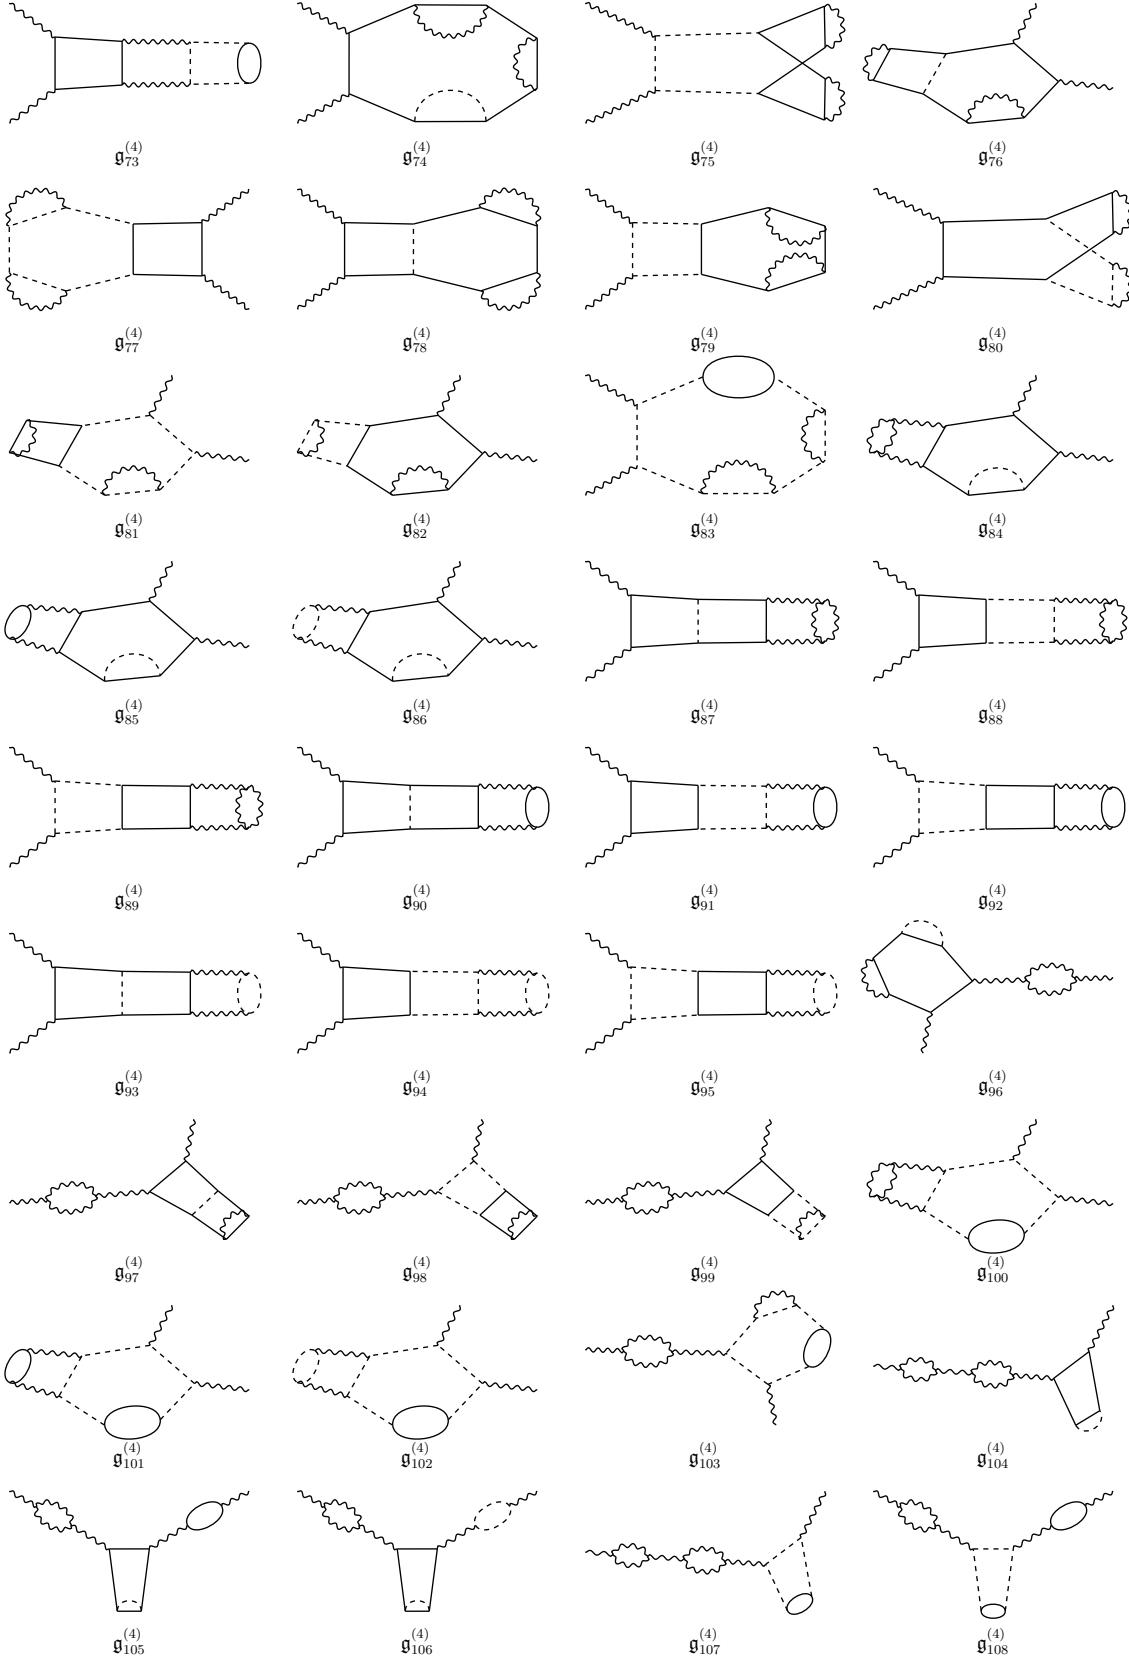

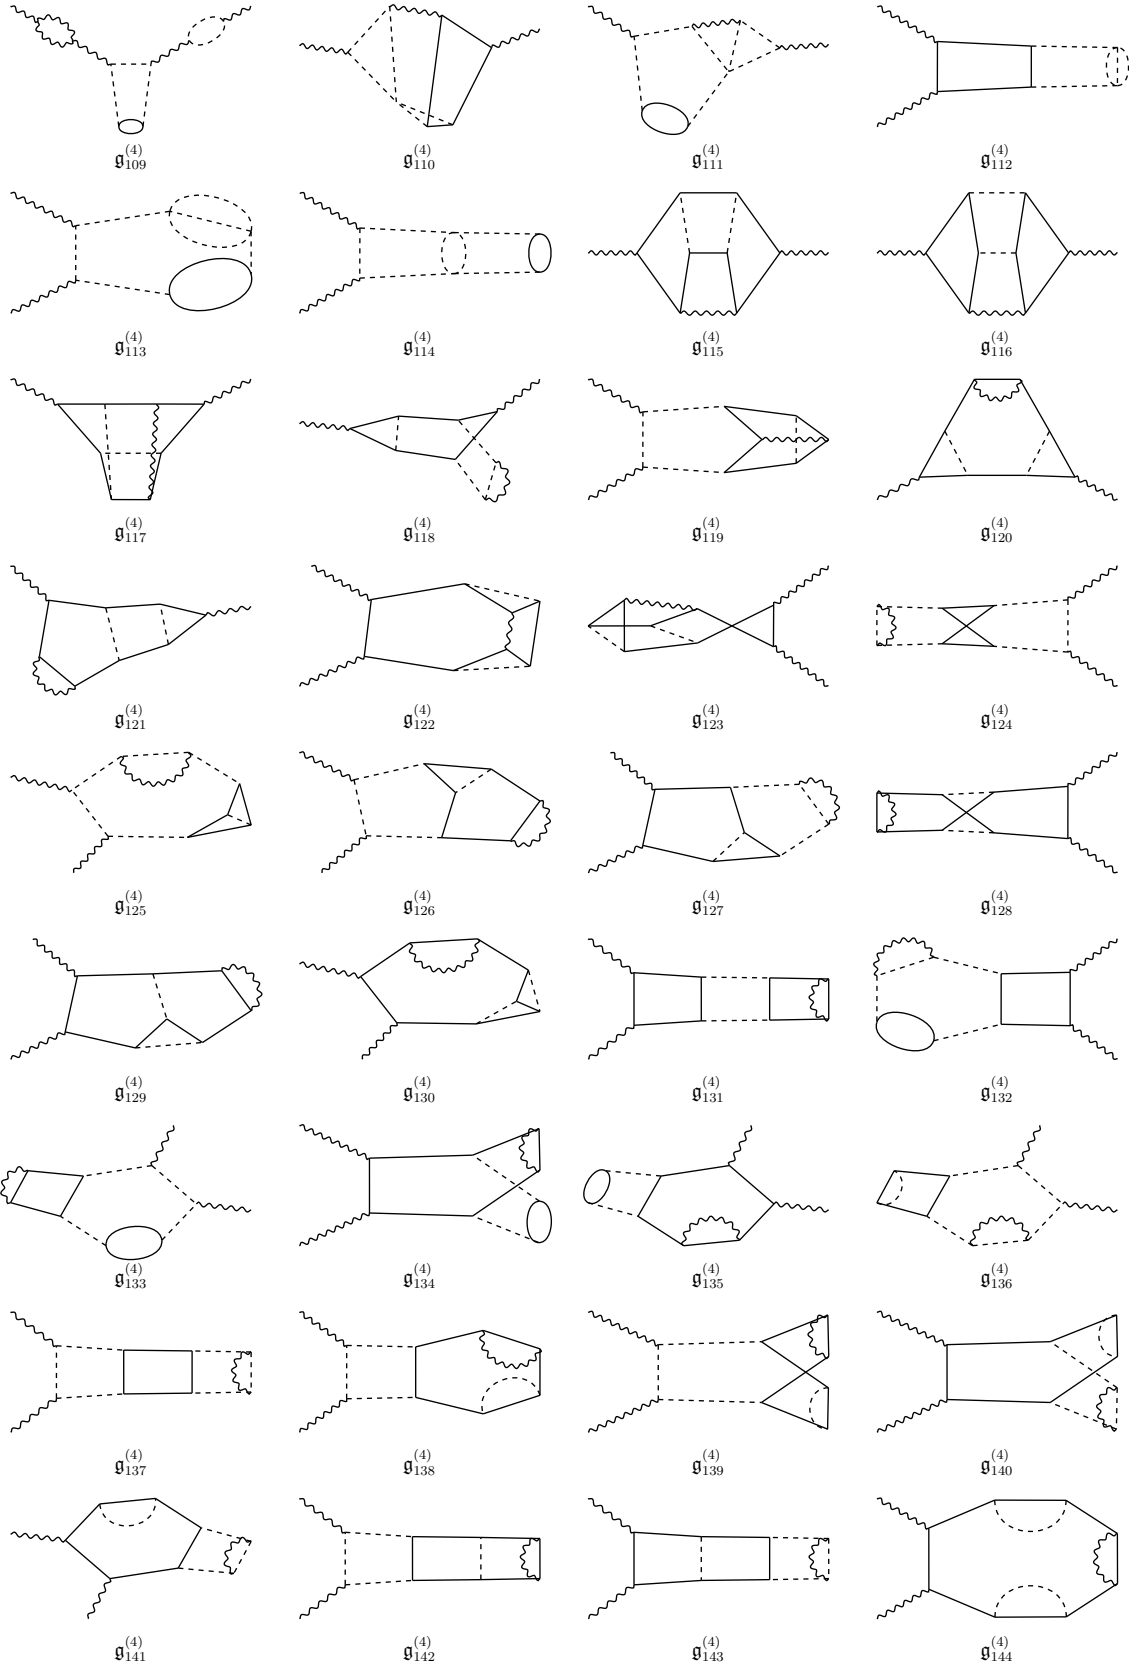

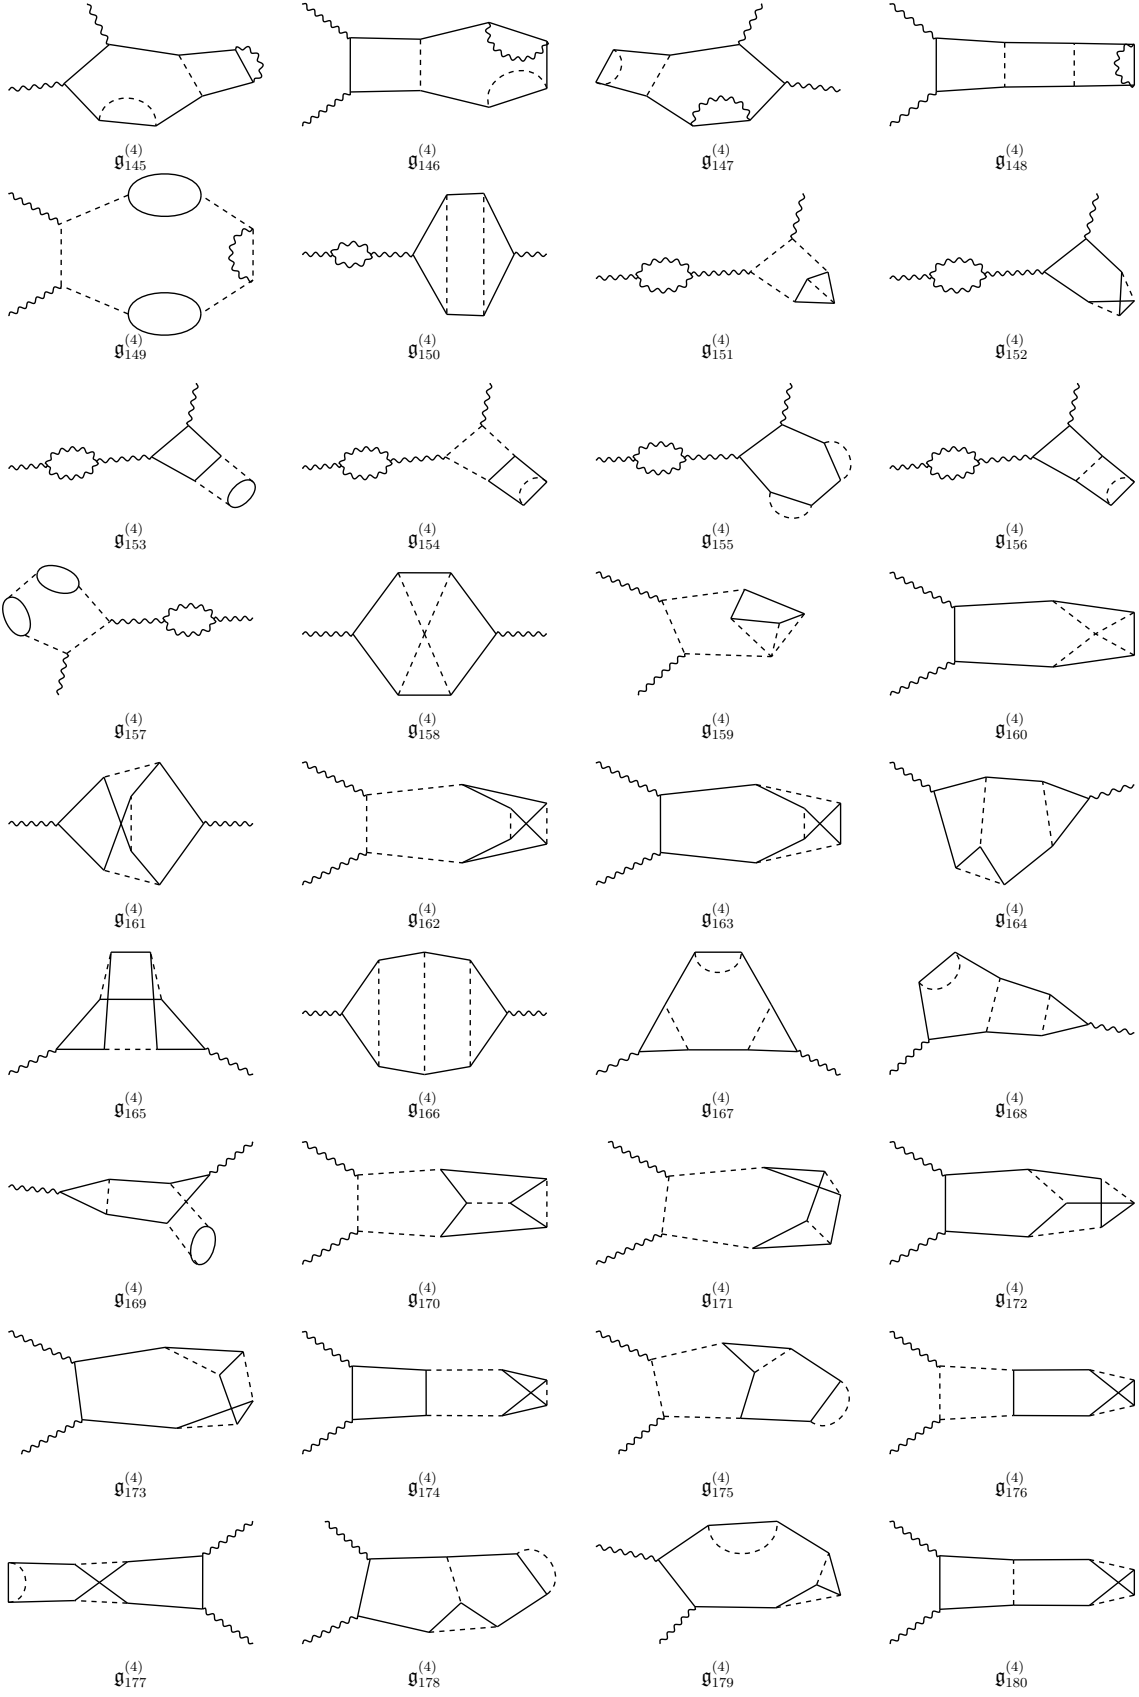

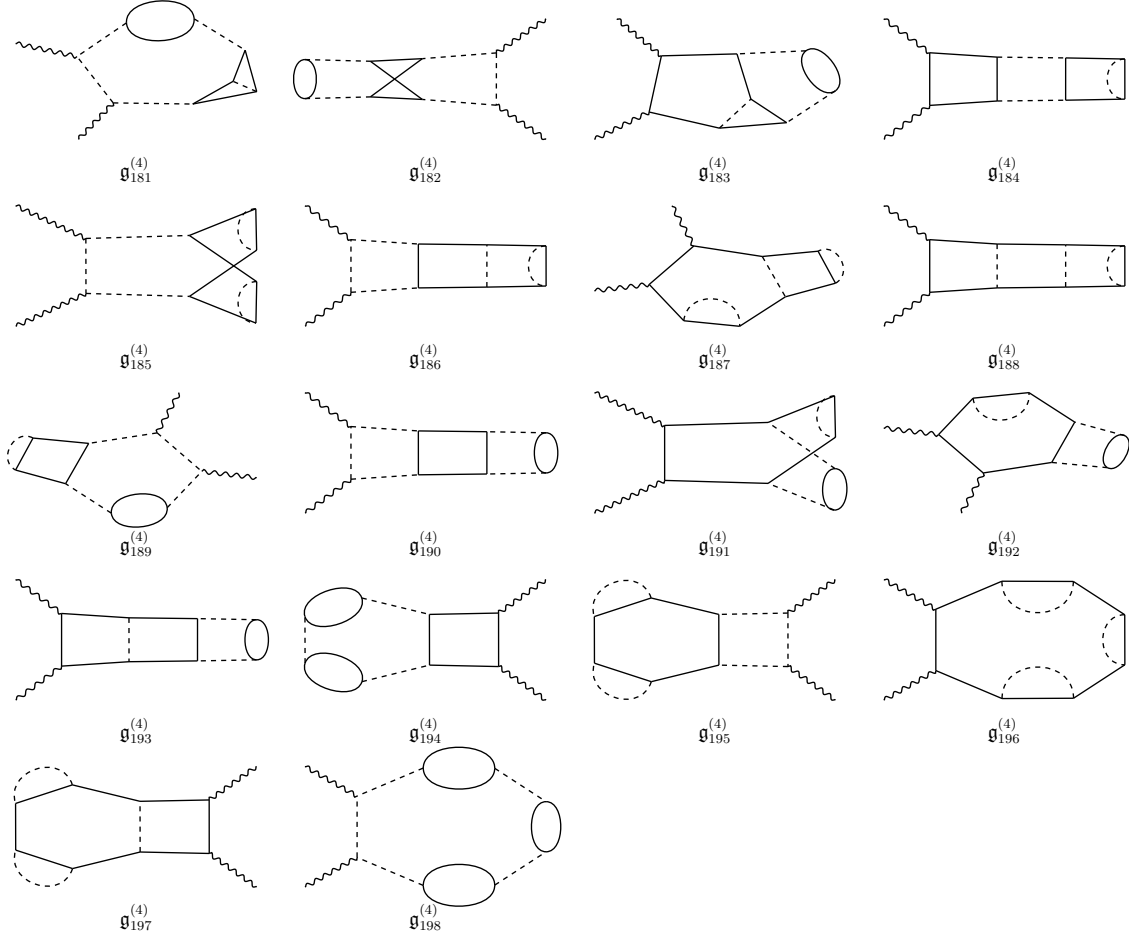

Of the TSs appearing in the 4-loop gauge  $\beta$ -function, there is a sign ambiguity in the graph notation for three of the terms. This can be adequately resolved by writing them out explicitly in regular tensor notation:

$$\begin{aligned}
 \beta_{AB}^{(4)} \supset & \mathfrak{g}_1^{(4)} G_{AC}^6 f^{CGH} f^{DHI} f^{EIJ} f^{FJG} f^{BKL} f^{DLM} f^{EMN} f^{FNK} \\
 & + \mathfrak{g}_3^{(4)} (T_\phi^A T_\phi^C T_\phi^D T_\phi^E T_\phi^F T_\phi^G) G_{DG}^2 f^{CEH} f^{FHI} G_{IB}^4 \\
 & + \mathfrak{g}_{55}^{(4)} (T_\phi^A T_\phi^C)_{ab} (T_\phi^D T_\phi^E)_{cd} \lambda_{abcd} f^{CDF} f^{EFG} G_{GB}^4.
 \end{aligned}$$

1.2 Yukawa  $\beta$ -function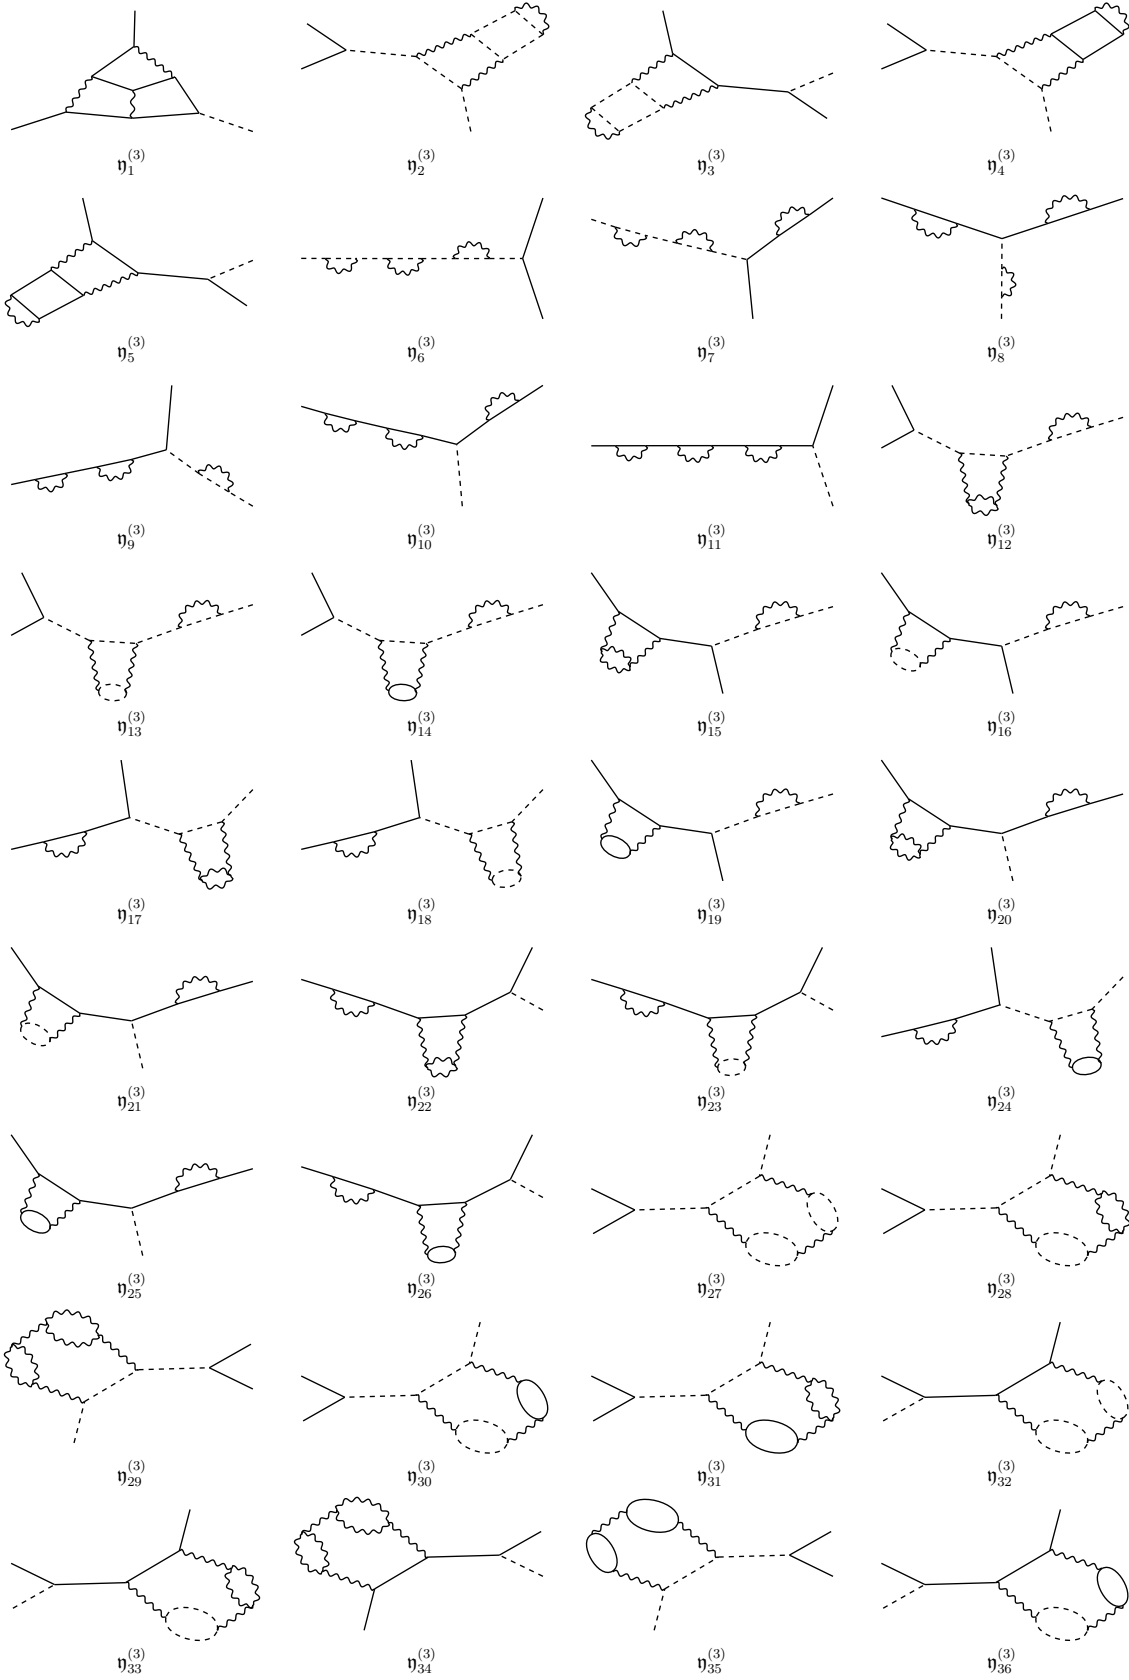



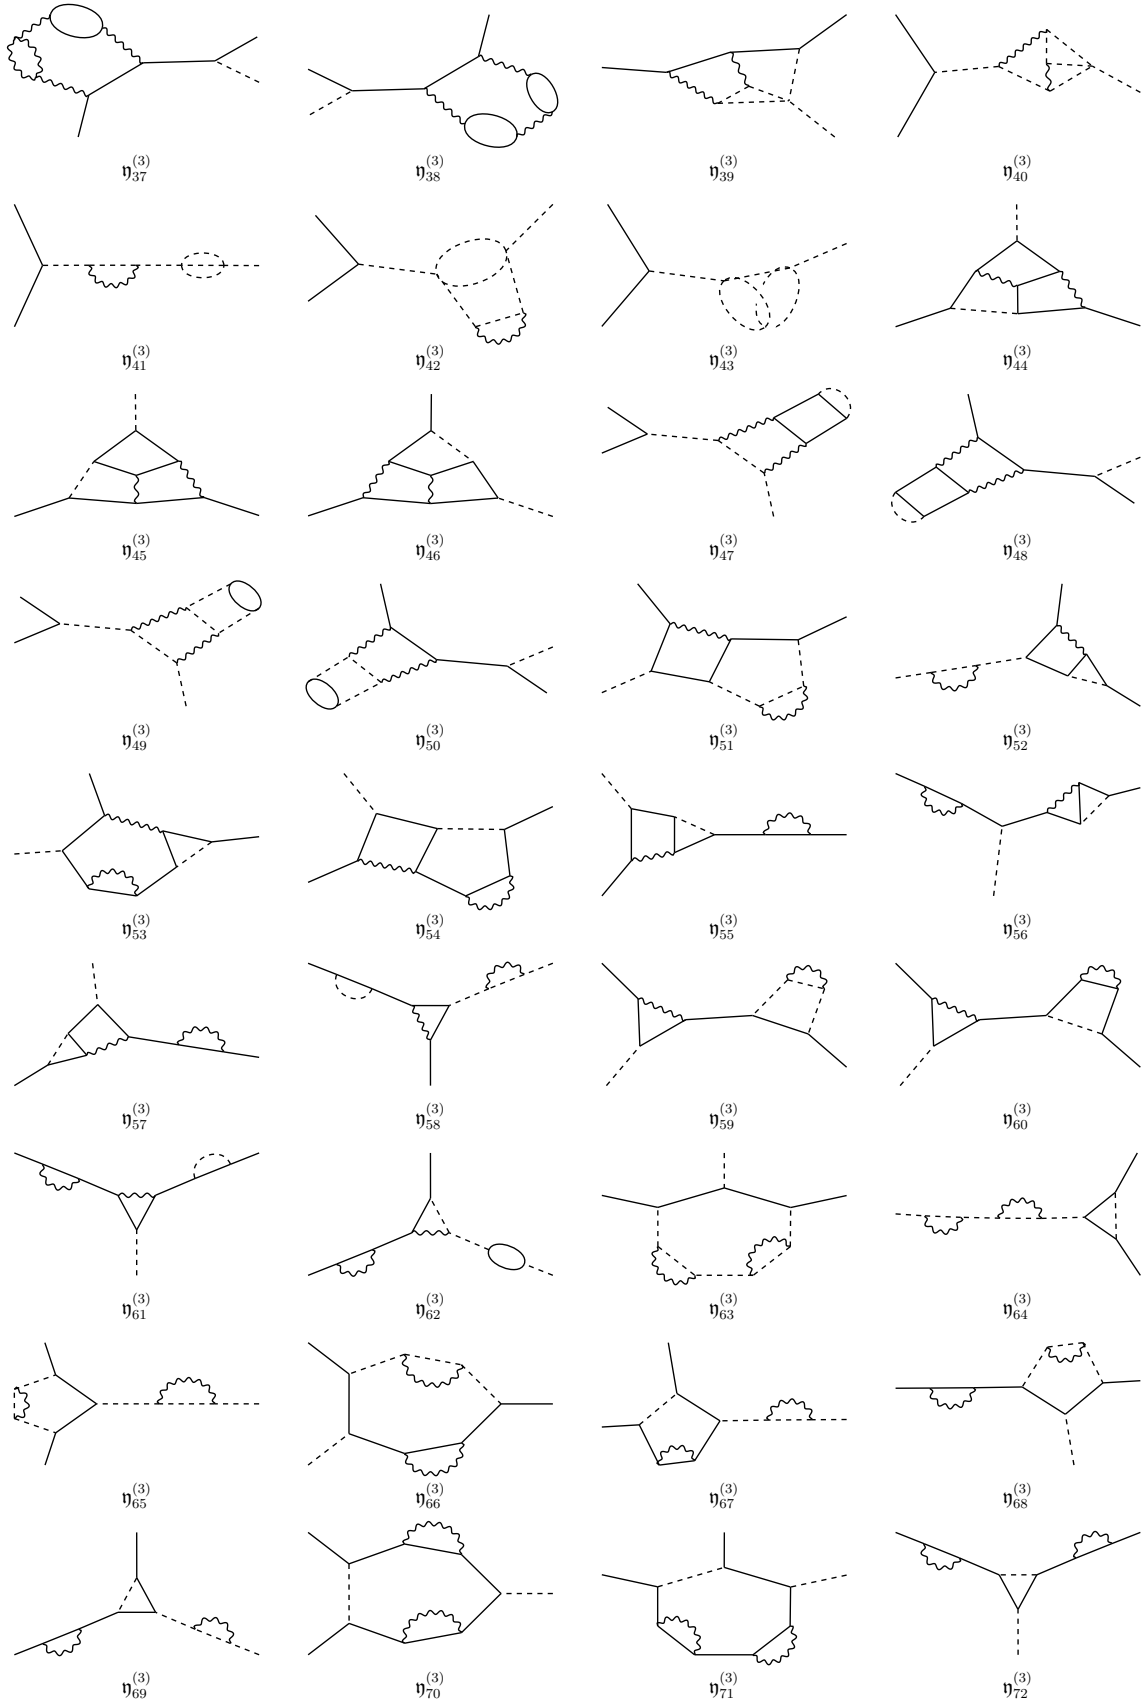

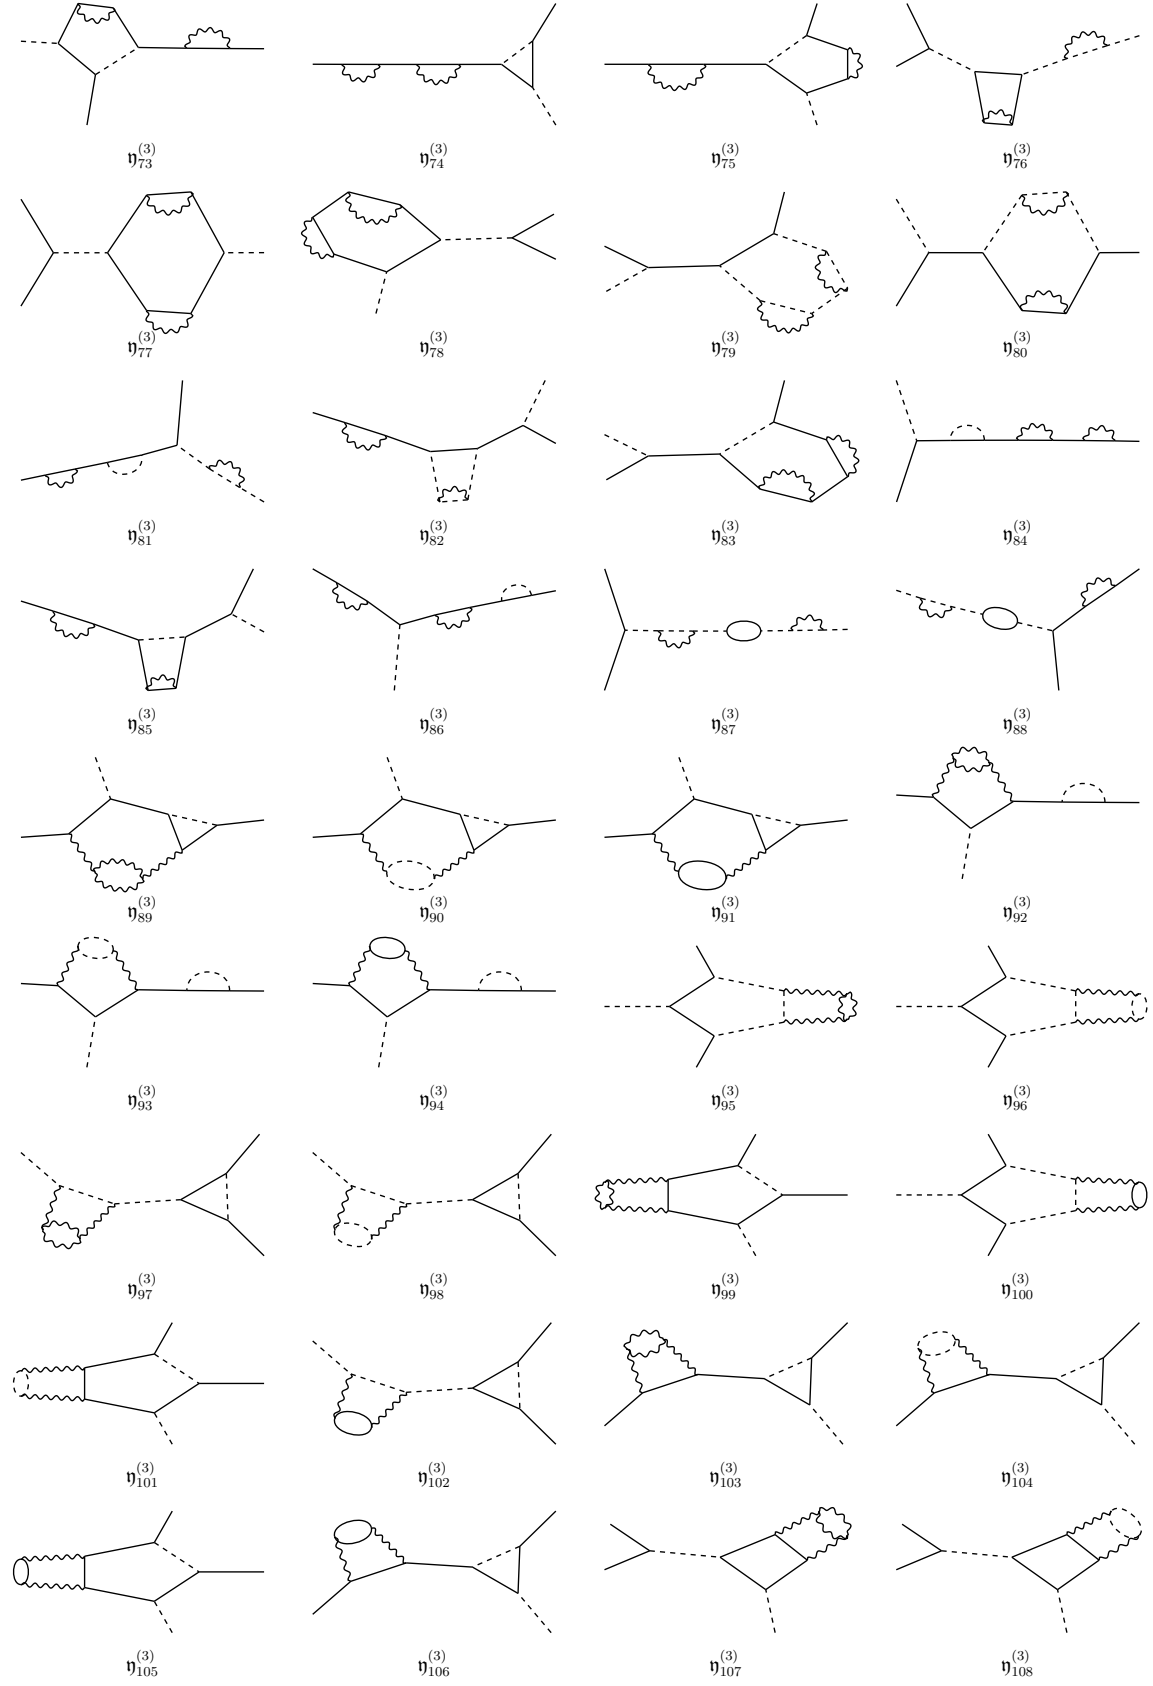

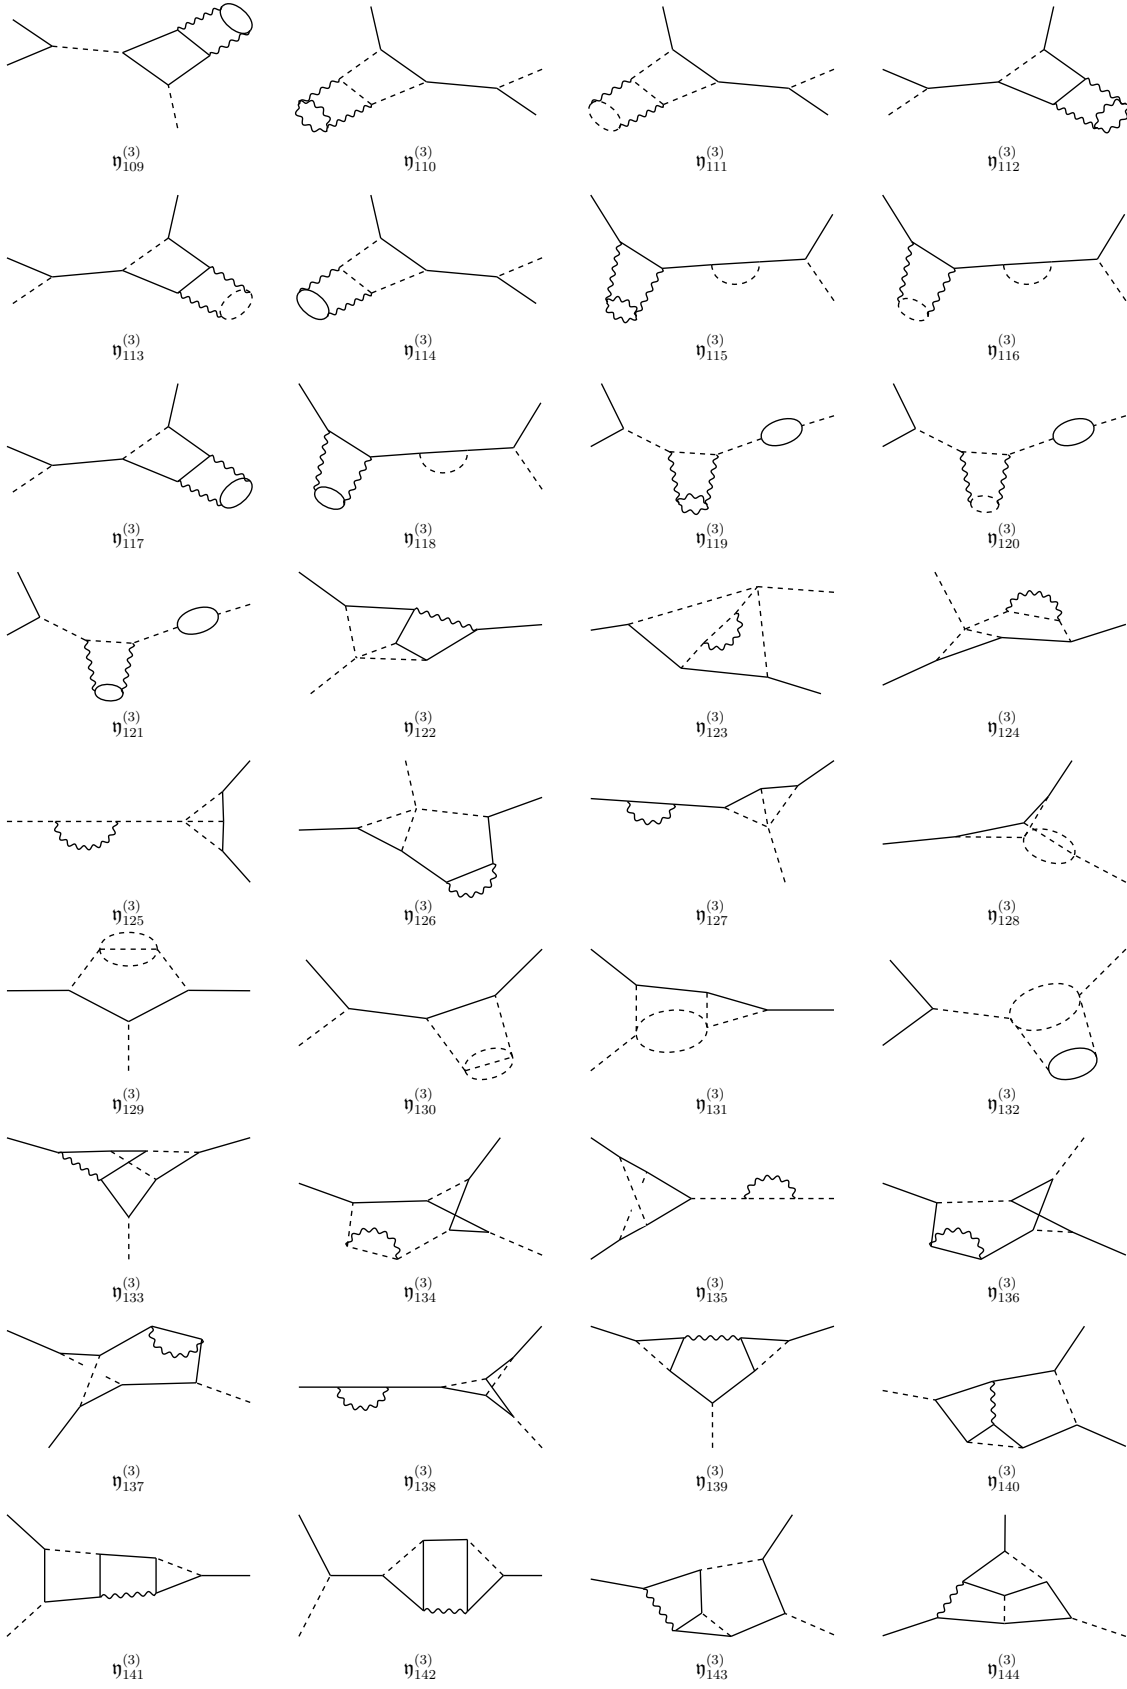

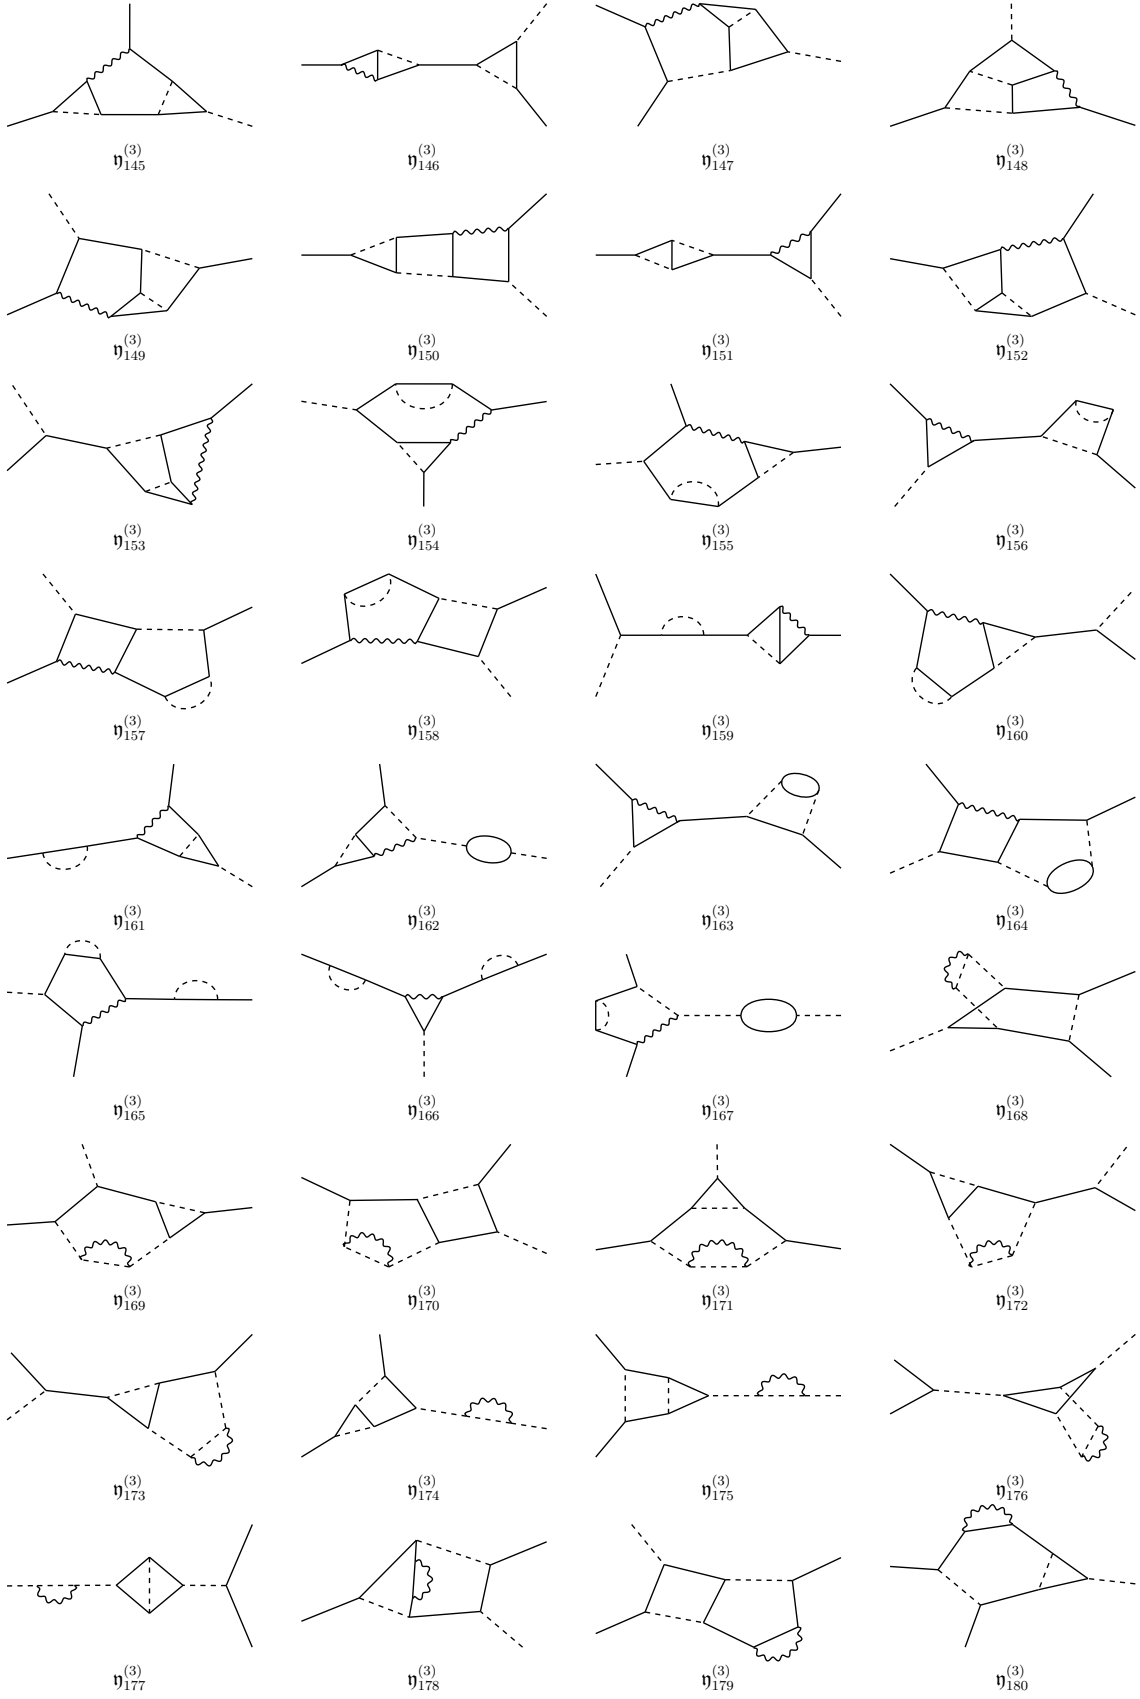

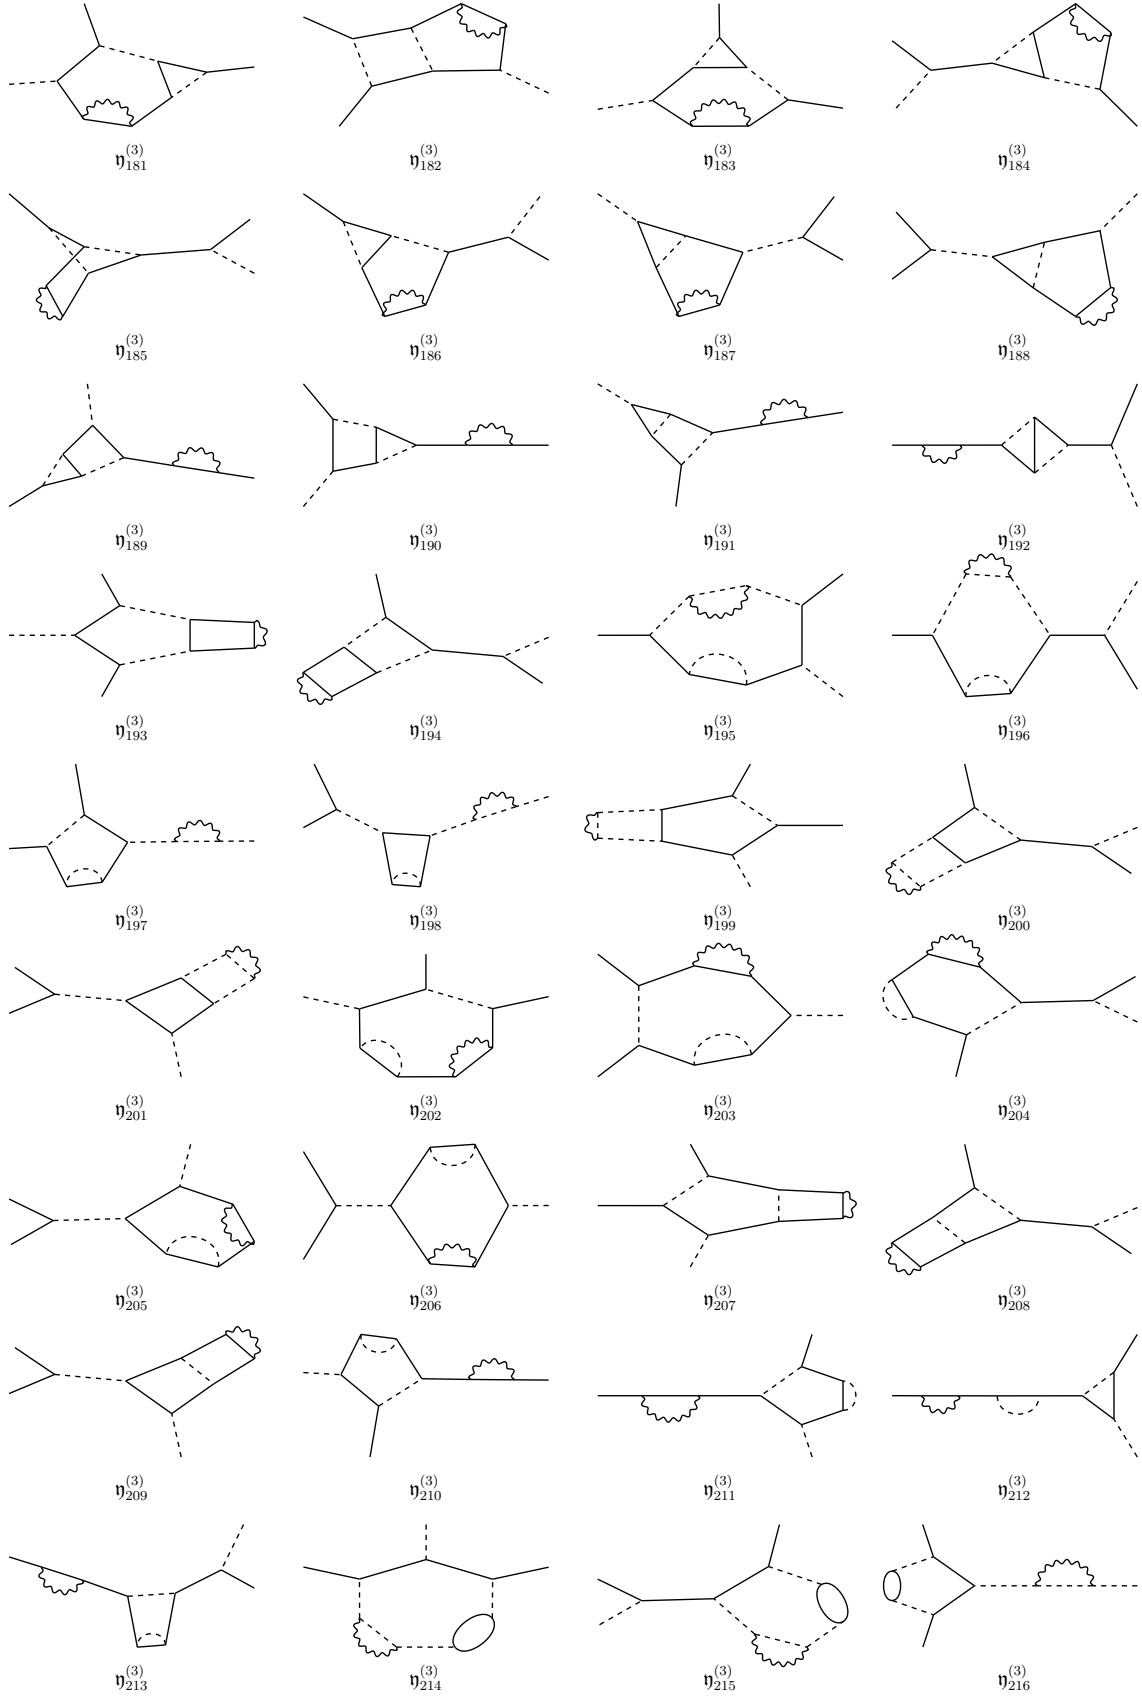

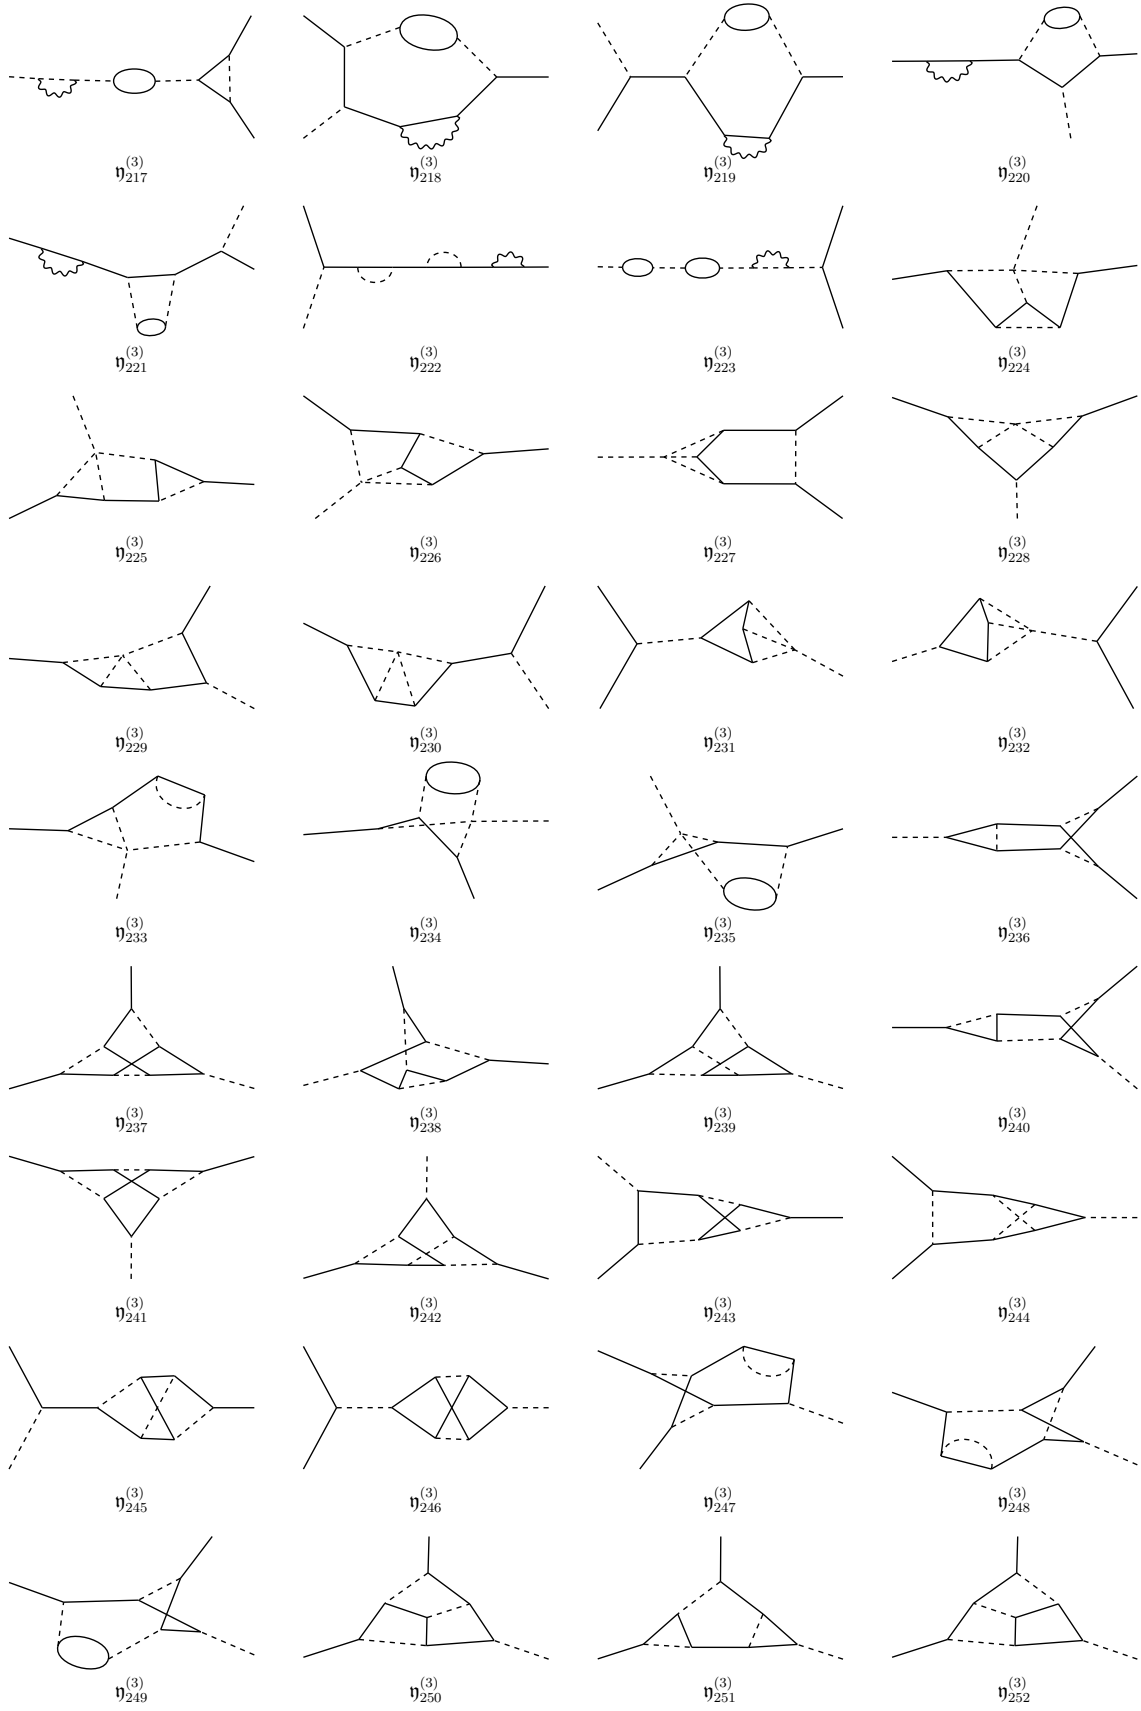

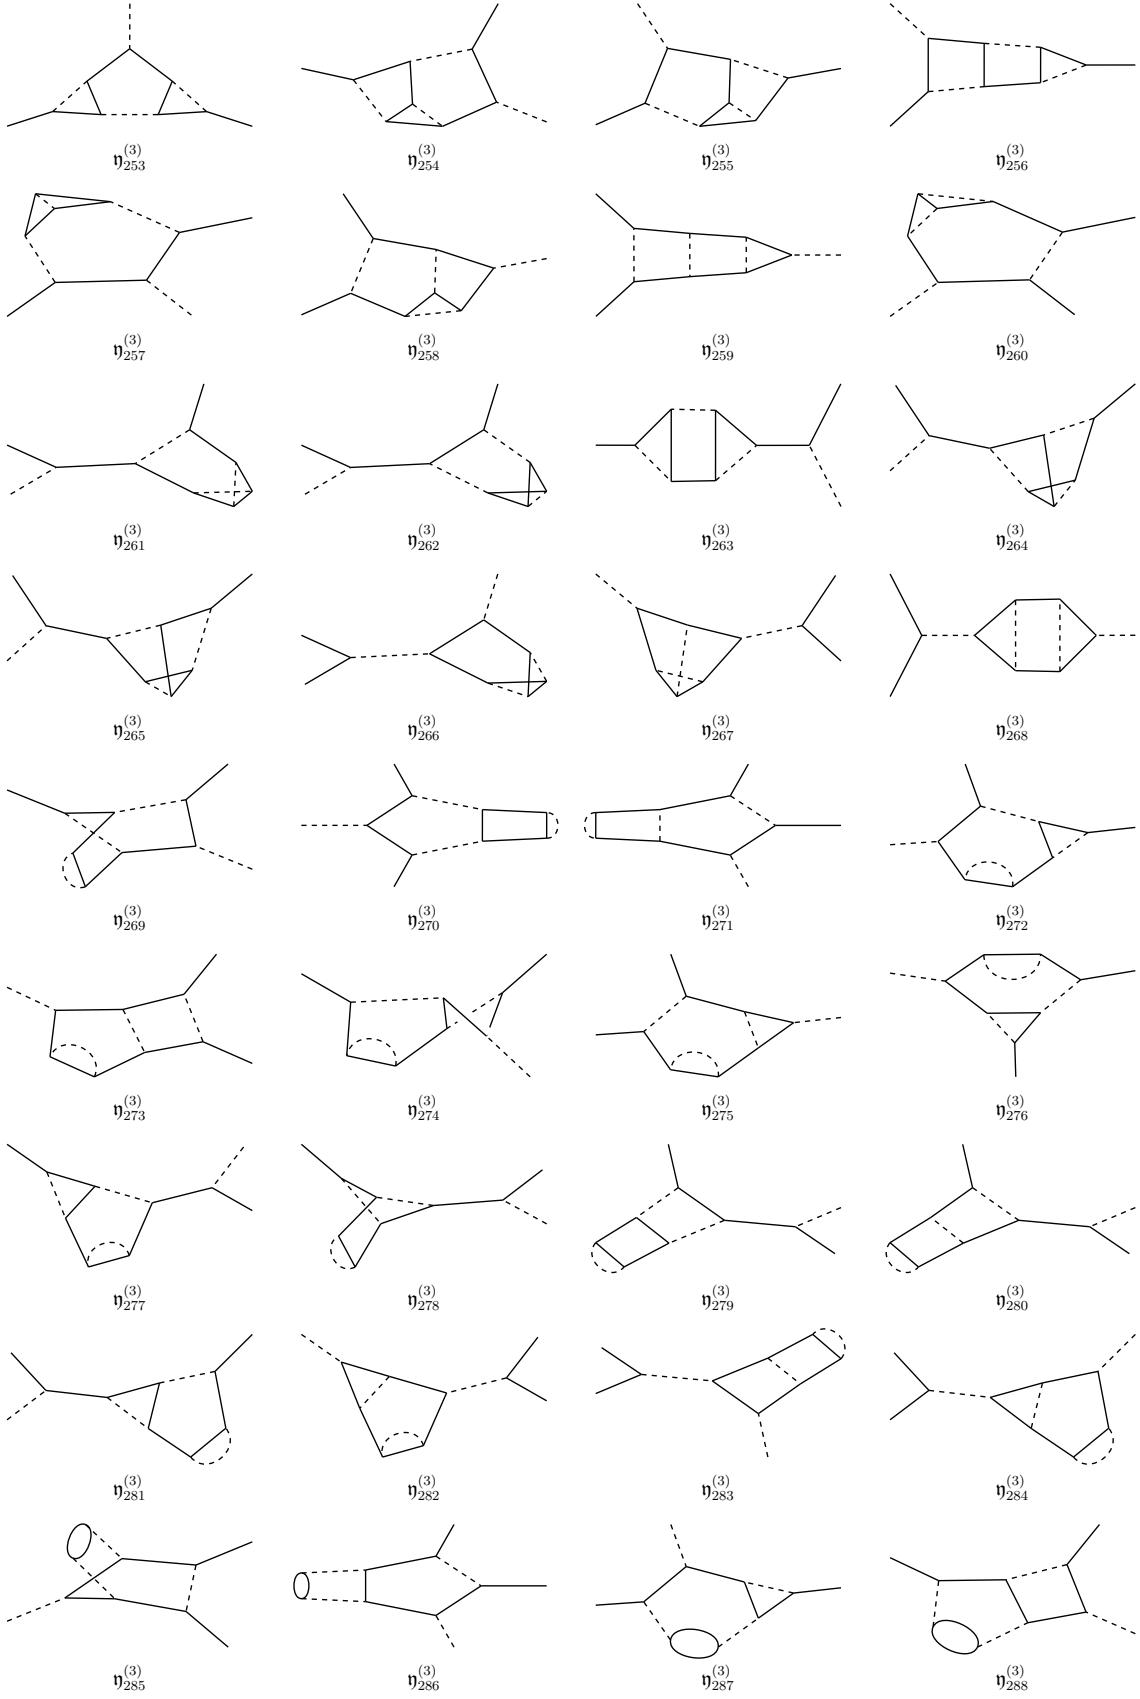

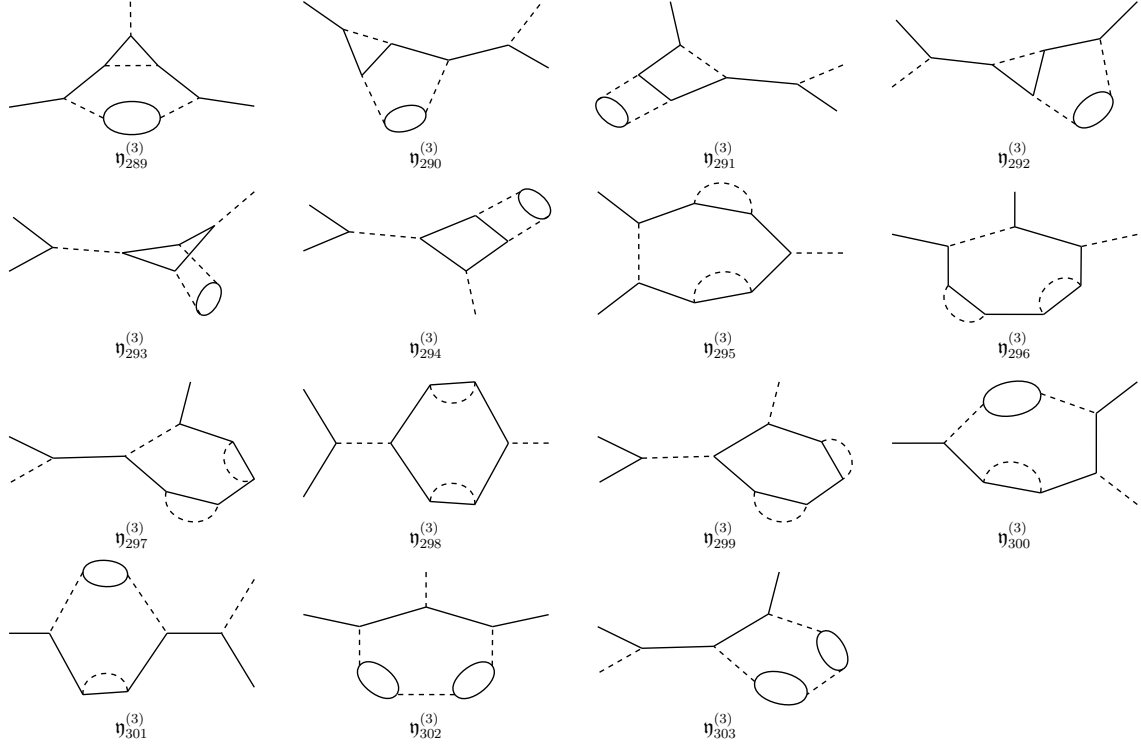

Of the TSs appearing in the 3-loop Yukawa  $\beta$ -function, there is a sign ambiguity in the graph notation for three of the terms. This can be adequately resolved by writing them out explicitly in regular tensor notation:

$$\begin{aligned}
 \beta_a^{(3)} \supset & \eta_{62}^{(3)} y_b T^A C_2(F) G_{AB}^2 (T_\phi^B)_{bc} [Y_2(S)]_{ca} \\
 & + \eta_{162}^{(3)} y_c \tilde{y}_b \tilde{T}^A y_b G_{AB}^2 (T_\phi^B)_{cd} [Y_2(S)]_{da} \\
 & + \eta_{167}^{(3)} y_b \tilde{Y}_2(F) T^A G_{AB}^2 (T_\phi^B)_{bc} [Y_2(S)]_{ca}.
 \end{aligned}$$



1.3 Quartic  $\beta$ -function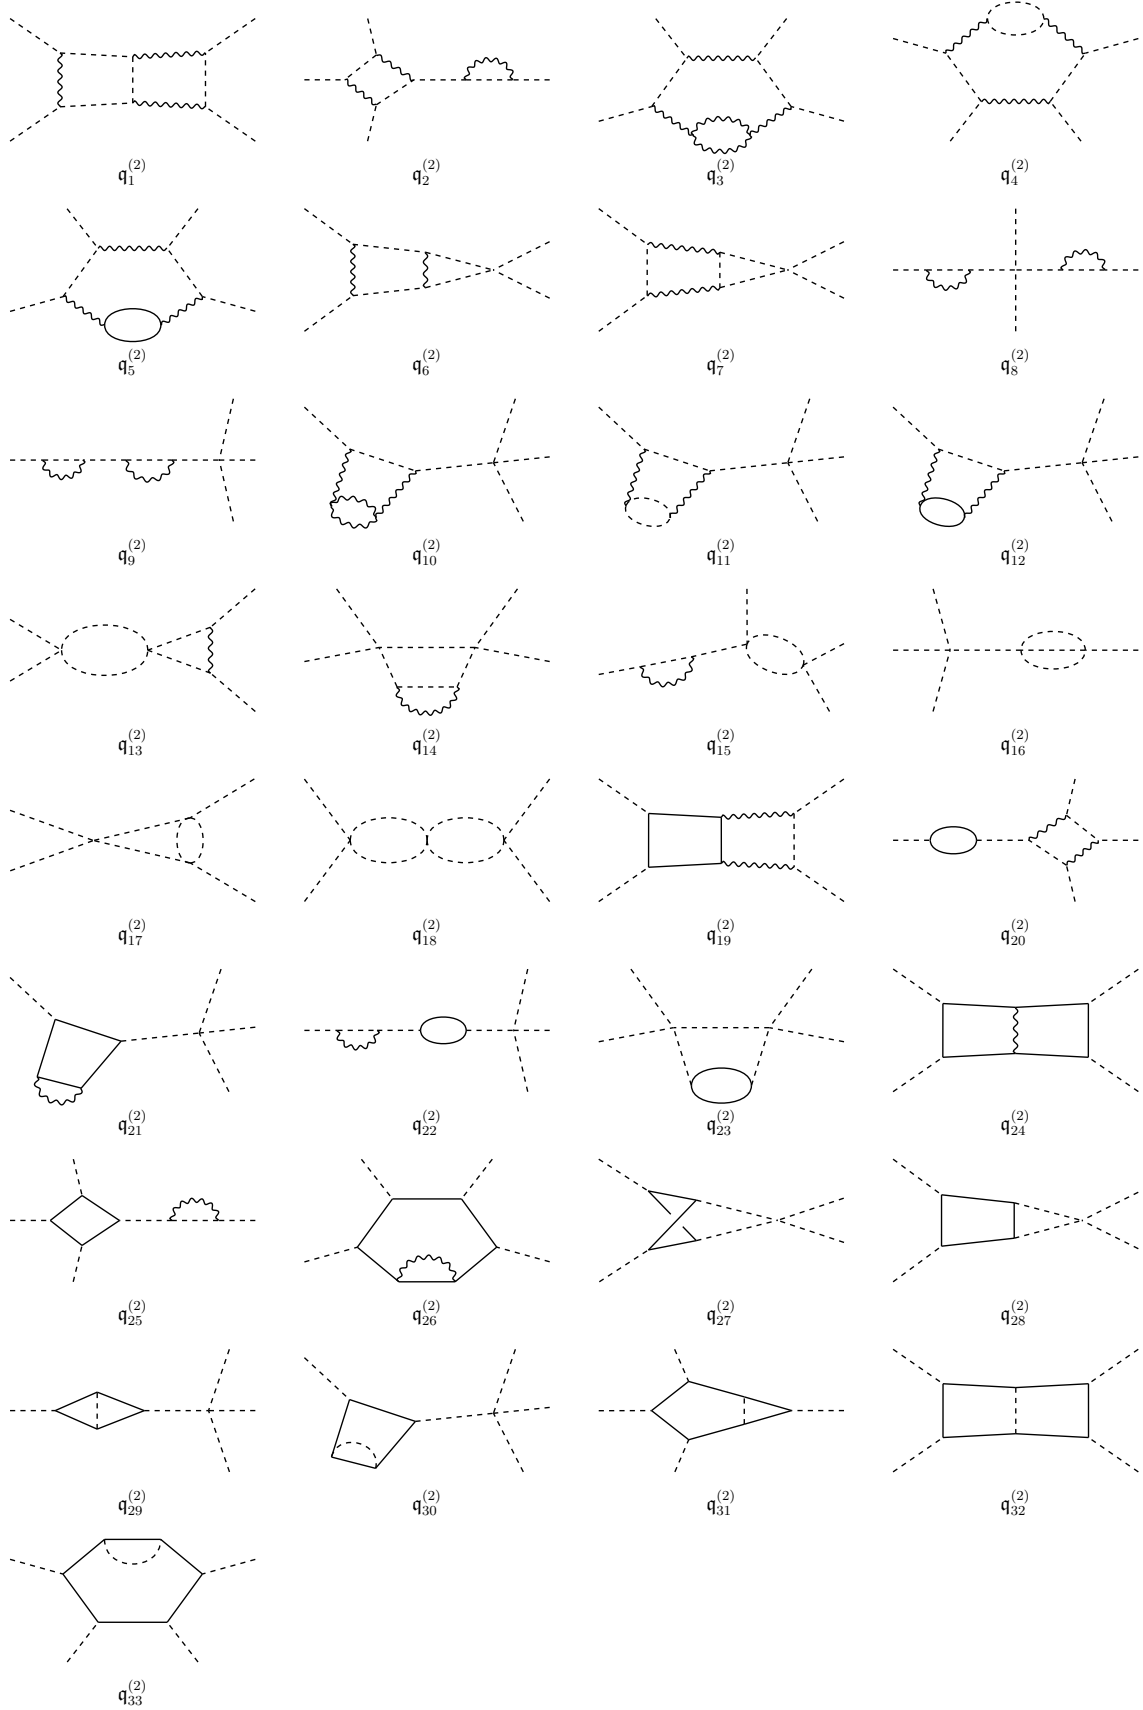

The sign ambiguity in the graph notation for  $q_{13}^{(2)}$  is determined in the tensor notation as it

appears in the appendix of the article.

## 2 Consistency conditions at 4–3–2

With this ancillary file comes included the file `ccs.mx`, which contains the set of consistency conditions ready to be loaded into Mathematica. We recommend using this file for any serious analysis. It is most simply loaded into a Mathematica notebook by placing it in the current directory and typing

```
<<ccs.mx
```

into the notebook. This loads three lists into the kernel: `ccs432` is a list with all 265 new CCs at 4–3–2 having substituted in the known 3–2–1  $\overline{\text{MS}}$  coefficients. `ccs432sym` is the 275 CCs from using a symmetric  $T_{IJ}$ . Finally, `msbarcoef` is a list of replacement rules for all  $\overline{\text{MS}}$   $\beta$ -function coefficients up to 3–2–2. In order to achieve the CCs after substituting in the known 2-loop quartic coefficients, one can use

```
Reduce[ccs432 /.msbarcoef, {}]
```

As for notation in the Mathematica framework we have used  $B[1, \ell, n]$  for the gauge coefficients  $\mathfrak{g}_n^{(\ell)}$ ,  $B[2, \ell, n]$  for the Yukawa coefficients  $\mathfrak{y}_n^{(\ell)}$ , and  $B[3, \ell, n]$  for the quartic coefficients  $\mathfrak{q}_n^{(\ell)}$ .

### 2.1 List of all CCs

The full list of  $\overline{\text{MS}}$  CCs at 4–3–2 is:

$$\begin{aligned}
\mathfrak{g}_9^{(4)} &= \frac{\mathfrak{g}_7^{(4)}}{2} + \frac{1}{2} \\
\mathfrak{g}_{10}^{(4)} &= \frac{\mathfrak{g}_8^{(4)}}{2} + \frac{1}{4} \\
\mathfrak{g}_{17}^{(4)} &= \frac{\mathfrak{g}_{15}^{(4)}}{2} + \frac{1}{3} \\
\mathfrak{g}_{18}^{(4)} &= \frac{\mathfrak{g}_{16}^{(4)}}{2} - \frac{29}{6} \\
\mathfrak{g}_{19}^{(4)} &= \mathfrak{g}_{13}^{(4)} + 11\mathfrak{g}_{15}^{(4)} - \frac{4}{3} \\
\mathfrak{g}_{20}^{(4)} &= \mathfrak{g}_{14}^{(4)} + 11\mathfrak{g}_{16}^{(4)} + \frac{58}{3} \\
\mathfrak{g}_{32}^{(4)} &= 2\mathfrak{g}_{21}^{(4)} - 4\mathfrak{g}_{22}^{(4)} + 8\mathfrak{g}_{23}^{(4)} - 4\mathfrak{g}_{24}^{(4)} + 2\mathfrak{g}_{27}^{(4)} \\
\mathfrak{g}_{39}^{(4)} &= \frac{\mathfrak{g}_{37}^{(4)}}{2} - \frac{2}{3} \\
\mathfrak{g}_{40}^{(4)} &= \frac{\mathfrak{g}_{38}^{(4)}}{2} - \frac{25}{12} \\
\mathfrak{g}_{42}^{(4)} &= -132\mathfrak{g}_{22}^{(4)} + 264\mathfrak{g}_{23}^{(4)} - 132\mathfrak{g}_{24}^{(4)} - 6\mathfrak{g}_{25}^{(4)} + 66\mathfrak{g}_{27}^{(4)} - \frac{6\mathfrak{g}_{29}^{(4)}}{11} + \frac{\mathfrak{g}_3^{(4)}}{44} \\
&\quad + \frac{3\mathfrak{g}_{30}^{(4)}}{11} + 3\mathfrak{g}_{31}^{(4)} + \frac{2\mathfrak{g}_{33}^{(4)}}{11} - \frac{\mathfrak{g}_{34}^{(4)}}{11} + 2\mathfrak{g}_{41}^{(4)} + \frac{7\mathfrak{g}_7^{(4)}}{22} - \frac{7\mathfrak{g}_8^{(4)}}{11} + \frac{3}{2}
\end{aligned}$$

$$\begin{aligned}
\mathfrak{g}_{44}^{(4)} &= -132\mathfrak{g}_{23}^{(4)} + 66\mathfrak{g}_{24}^{(4)} + 3\mathfrak{g}_{26}^{(4)} - 6\mathfrak{g}_{28}^{(4)} - \frac{3\mathfrak{g}_{29}^{(4)}}{11} + \frac{\mathfrak{g}_3^{(4)}}{88} \\
&\quad + \frac{3\mathfrak{g}_{30}^{(4)}}{22} + \frac{\mathfrak{g}_{33}^{(4)}}{11} - \frac{\mathfrak{g}_{34}^{(4)}}{22} + 2\mathfrak{g}_{43}^{(4)} - \frac{\mathfrak{g}_7^{(4)}}{11} + \frac{2\mathfrak{g}_8^{(4)}}{11} + \frac{3}{2} \\
\mathfrak{g}_{60}^{(4)} &= 2\mathfrak{g}_{58}^{(4)} + 44\mathfrak{g}_{59}^{(4)} + \frac{26}{3} \\
\mathfrak{g}_{61}^{(4)} &= 2\mathfrak{g}_{59}^{(4)} + \frac{1}{3} \\
\mathfrak{g}_{72}^{(4)} &= \frac{\mathfrak{g}_{70}^{(4)}}{2} - \frac{1}{8} \\
\mathfrak{g}_{73}^{(4)} &= \frac{\mathfrak{g}_{71}^{(4)}}{2} \\
\mathfrak{g}_{82}^{(4)} &= -2\mathfrak{g}_{75}^{(4)} + 2\mathfrak{g}_{79}^{(4)} + \mathfrak{g}_{80}^{(4)} - 6 \\
\mathfrak{g}_{93}^{(4)} &= -\frac{\mathfrak{g}_{85}^{(4)}}{2} + \mathfrak{g}_{86}^{(4)} + \frac{\mathfrak{g}_{90}^{(4)}}{2} - \frac{1}{6} \\
\mathfrak{g}_{95}^{(4)} &= \frac{\mathfrak{g}_{92}^{(4)}}{2} + \frac{1}{6} \\
\mathfrak{g}_{97}^{(4)} &= -2\mathfrak{g}_{84}^{(4)} - 22\mathfrak{g}_{85}^{(4)} + 2\mathfrak{g}_{87}^{(4)} + 22\mathfrak{g}_{90}^{(4)} + \mathfrak{g}_{96}^{(4)} + \frac{4}{3} \\
\mathfrak{g}_{99}^{(4)} &= \frac{\mathfrak{g}_{69}^{(4)}}{4} + 2\mathfrak{g}_{89}^{(4)} + 22\mathfrak{g}_{92}^{(4)} - \frac{112}{3} \\
\mathfrak{g}_{102}^{(4)} &= \frac{\mathfrak{g}_{101}^{(4)}}{2} + \frac{7}{12} \\
\mathfrak{g}_{103}^{(4)} &= 2\mathfrak{g}_{100}^{(4)} + 22\mathfrak{g}_{101}^{(4)} - \frac{\mathfrak{g}_{69}^{(4)}}{8} + \frac{53}{6} \\
\mathfrak{g}_{119}^{(4)} &= \mathfrak{g}_{118}^{(4)} - 12 \\
\mathfrak{g}_{123}^{(4)} &= -\mathfrak{g}_{120}^{(4)} + \mathfrak{g}_{121}^{(4)} + \mathfrak{g}_{122}^{(4)} \\
\mathfrak{g}_{143}^{(4)} &= -\mathfrak{g}_{138}^{(4)} + \mathfrak{g}_{139}^{(4)} - \mathfrak{g}_{140}^{(4)} + \mathfrak{g}_{141}^{(4)} + \mathfrak{g}_{142}^{(4)} + 3 \\
\eta_1^{(3)} &= 2\mathfrak{g}_{69}^{(3)} \\
\eta_2^{(3)} &= -3 \\
\eta_3^{(3)} &= -\frac{3\mathfrak{g}_7^{(4)}}{2} - \frac{5}{2} \\
\eta_4^{(3)} &= -\frac{3}{2} \\
\eta_5^{(3)} &= -\frac{3\mathfrak{g}_8^{(4)}}{2} - \frac{5}{4} \\
\eta_6^{(3)} &= 2\mathfrak{g}_{83}^{(4)} + \frac{147}{2} \\
\eta_9^{(3)} &= -6\mathfrak{g}_{75}^{(4)} + 6\mathfrak{g}_{79}^{(4)} + \eta_8^{(3)} + 9 \\
\eta_{13}^{(3)} &= \frac{3\mathfrak{g}_{100}^{(4)}}{11} + 3\mathfrak{g}_{101}^{(4)} - \frac{\mathfrak{g}_{69}^{(4)}}{88} - \frac{\eta_{12}^{(3)}}{22} + \frac{227}{88} \\
\eta_{14}^{(3)} &= \frac{6\mathfrak{g}_{100}^{(4)}}{11} + 6\mathfrak{g}_{101}^{(4)} - \frac{\mathfrak{g}_{69}^{(4)}}{44} - \frac{\eta_{12}^{(3)}}{11} - \frac{81}{44}
\end{aligned}$$

$$\begin{aligned}
\eta_{16}^{(3)} &= \frac{\mathfrak{g}_{69}^{(4)}}{44} + \frac{3\mathfrak{g}_{89}^{(4)}}{11} + 3\mathfrak{g}_{92}^{(4)} - \frac{\eta_{15}^{(3)}}{22} - \frac{1}{11} \\
\eta_{18}^{(3)} &= -\frac{9\mathfrak{g}_{153}^{(4)}}{11} + \frac{9\mathfrak{g}_{154}^{(4)}}{11} + \frac{9\mathfrak{g}_{156}^{(4)}}{11} - \frac{\mathfrak{g}_{69}^{(4)}}{88} + \frac{3\mathfrak{g}_{98}^{(4)}}{22} - \frac{\eta_{17}^{(3)}}{22} + \frac{29}{22} \\
\eta_{19}^{(3)} &= \frac{\mathfrak{g}_{69}^{(4)}}{22} + \frac{6\mathfrak{g}_{89}^{(4)}}{11} + 6\mathfrak{g}_{92}^{(4)} - \frac{\eta_{15}^{(3)}}{11} + \frac{42}{11} \\
\eta_{21}^{(3)} &= \frac{9\mathfrak{g}_{153}^{(4)}}{11} + \frac{\mathfrak{g}_{69}^{(4)}}{88} - \frac{3\mathfrak{g}_{84}^{(4)}}{11} - 3\mathfrak{g}_{85}^{(4)} + \frac{3\mathfrak{g}_{87}^{(4)}}{11} + 3\mathfrak{g}_{90}^{(4)} + \frac{3\mathfrak{g}_{96}^{(4)}}{22} - \frac{\eta_{20}^{(3)}}{22} - \frac{43}{11} \\
\eta_{23}^{(3)} &= \frac{9\mathfrak{g}_{153}^{(4)}}{11} + \frac{\mathfrak{g}_{69}^{(4)}}{88} + \frac{3\mathfrak{g}_{96}^{(4)}}{22} - \frac{\eta_{22}^{(3)}}{22} - \frac{32}{11} \\
\eta_{24}^{(3)} &= -\frac{18\mathfrak{g}_{153}^{(4)}}{11} + \frac{18\mathfrak{g}_{154}^{(4)}}{11} + \frac{18\mathfrak{g}_{156}^{(4)}}{11} - \frac{\mathfrak{g}_{69}^{(4)}}{44} + \frac{3\mathfrak{g}_{98}^{(4)}}{11} - \frac{\eta_{17}^{(3)}}{11} + \frac{73}{11} \\
\eta_{25}^{(3)} &= \frac{18\mathfrak{g}_{153}^{(4)}}{11} + \frac{\mathfrak{g}_{69}^{(4)}}{44} - \frac{6\mathfrak{g}_{84}^{(4)}}{11} - 6\mathfrak{g}_{85}^{(4)} + \frac{6\mathfrak{g}_{87}^{(4)}}{11} + 6\mathfrak{g}_{90}^{(4)} + \frac{3\mathfrak{g}_{96}^{(4)}}{11} - \frac{\eta_{20}^{(3)}}{11} - \frac{86}{11} \\
\eta_{26}^{(3)} &= \frac{18\mathfrak{g}_{153}^{(4)}}{11} + \frac{\mathfrak{g}_{69}^{(4)}}{44} + \frac{3\mathfrak{g}_{96}^{(4)}}{11} - \frac{\eta_{22}^{(3)}}{11} - \frac{86}{11} \\
\eta_{29}^{(3)} &= 2\mathfrak{g}_{107}^{(4)} + 44\mathfrak{g}_{109}^{(4)} + 4\mathfrak{g}_{71}^{(4)} - 484\eta_{27}^{(3)} - 22\eta_{28}^{(3)} - 33 \\
\eta_{31}^{(3)} &= 2\mathfrak{g}_{108}^{(4)} - 4\mathfrak{g}_{109}^{(4)} - \mathfrak{g}_{71}^{(4)} + 88\eta_{27}^{(3)} + 2\eta_{28}^{(3)} - 22\eta_{30}^{(3)} + \frac{3}{2} \\
\eta_{34}^{(3)} &= 2\mathfrak{g}_{104}^{(4)} + 44\mathfrak{g}_{106}^{(4)} - 1452\mathfrak{g}_{23}^{(4)} - 66\mathfrak{g}_{28}^{(4)} - 3\mathfrak{g}_{29}^{(4)} + \mathfrak{g}_{33}^{(4)} \\
&\quad + 22\mathfrak{g}_{43}^{(4)} + 4\mathfrak{g}_{70}^{(4)} + 2\mathfrak{g}_8^{(4)} - 484\eta_{32}^{(3)} - 22\eta_{33}^{(3)} + \frac{214}{3} \\
\eta_{35}^{(3)} &= 2\eta_{30}^{(3)} - 4\eta_{27}^{(3)} \\
\eta_{37}^{(3)} &= 2\mathfrak{g}_{105}^{(4)} - 4\mathfrak{g}_{106}^{(4)} - 66\mathfrak{g}_{22}^{(4)} + 264\mathfrak{g}_{23}^{(4)} - 3\mathfrak{g}_{25}^{(4)} + 6\mathfrak{g}_{28}^{(4)} + \mathfrak{g}_{41}^{(4)} \\
&\quad - 2\mathfrak{g}_{43}^{(4)} - \mathfrak{g}_{70}^{(4)} - \frac{\mathfrak{g}_8^{(4)}}{2} + 88\eta_{32}^{(3)} + 2\eta_{33}^{(3)} - 22\eta_{36}^{(3)} - \frac{35}{6} \\
\eta_{38}^{(3)} &= -3\mathfrak{g}_{21}^{(4)} + 6\mathfrak{g}_{22}^{(4)} - 12\mathfrak{g}_{23}^{(4)} - 4\eta_{32}^{(3)} + 2\eta_{36}^{(3)} \\
\eta_{39}^{(3)} &= 3\mathfrak{g}_{110}^{(4)} \\
\eta_{41}^{(3)} &= \frac{\mathfrak{g}_{111}^{(4)}}{4} + 6\mathfrak{g}_{113}^{(4)} + \frac{\mathfrak{g}_{56}^{(4)}}{24} - \frac{\mathfrak{g}_{57}^{(4)}}{12} - \frac{\eta_{40}^{(3)}}{12} - \frac{1}{4} \\
\eta_{42}^{(3)} &= \frac{3\mathfrak{g}_{111}^{(4)}}{4} + 6\mathfrak{g}_{114}^{(4)} + \frac{\mathfrak{g}_{56}^{(4)}}{8} - \frac{\mathfrak{g}_{57}^{(4)}}{4} - \frac{\eta_{40}^{(3)}}{4} \\
\eta_{45}^{(3)} &= 6\mathfrak{g}_{116}^{(4)} \\
\eta_{46}^{(3)} &= 6\mathfrak{g}_{115}^{(4)} - 12\mathfrak{g}_{117}^{(4)} + 2\eta_{44}^{(3)} \\
\eta_{47}^{(3)} &= \frac{3}{4} \\
\eta_{48}^{(3)} &= \frac{5}{8} - \frac{3\mathfrak{g}_{70}^{(4)}}{2} \\
\eta_{49}^{(3)} &= 0 \\
\eta_{50}^{(3)} &= -\frac{3\mathfrak{g}_{71}^{(4)}}{2} \\
\eta_{51}^{(3)} &= -12\mathfrak{g}_{117}^{(4)} + 6\mathfrak{g}_{118}^{(4)} + 2\eta_{44}^{(3)}
\end{aligned}$$

$$\begin{aligned}
\eta_{52}^{(3)} &= -12g_{117}^{(4)} + 6g_{118}^{(4)} + 2\eta_{44}^{(3)} - 108 \\
\eta_{54}^{(3)} &= 12g_{117}^{(4)} - 6g_{120}^{(4)} + 6g_{121}^{(4)} + 36g_{167}^{(4)} - 36g_{169}^{(4)} - 72g_{186}^{(4)} + 72g_{190}^{(4)} - 2\eta_{44}^{(3)} + \eta_{53}^{(3)} - 18 \\
\eta_{55}^{(3)} &= 6g_{120}^{(4)} + 36g_{167}^{(4)} + 24 \\
\eta_{56}^{(3)} &= -12g_{137}^{(4)} - 12g_{142}^{(4)} - 72g_{186}^{(4)} + 42 \\
\eta_{57}^{(3)} &= 12g_{117}^{(4)} + 6g_{121}^{(4)} + 36g_{169}^{(4)} + 72g_{186}^{(4)} - 72g_{190}^{(4)} - 2\eta_{44}^{(3)} + 42 \\
\eta_{58}^{(3)} &= 6g_{117}^{(4)} - 6g_{136}^{(4)} - \frac{g_{69}^{(4)}}{12} - g_{81}^{(4)} - \eta_{44}^{(3)} + \frac{\eta_7^{(3)}}{3} + 38 \\
\eta_{59}^{(3)} &= 12g_{117}^{(4)} - 12g_{137}^{(4)} - 2\eta_{44}^{(3)} + 54 \\
\eta_{62}^{(3)} &= 3g_{134}^{(4)} - 3g_{135}^{(4)} - \frac{g_{74}^{(4)}}{2} + \frac{g_{78}^{(4)}}{2} - \frac{\eta_{10}^{(3)}}{12} + \frac{\eta_{11}^{(3)}}{4} + \frac{5}{2} \\
\eta_{63}^{(3)} &= 3g_{125}^{(4)} + \frac{g_{69}^{(4)}}{4} - 2g_{77}^{(4)} + g_{81}^{(4)} - \frac{131}{4} \\
\eta_{64}^{(3)} &= 3g_{125}^{(4)} + \frac{g_{69}^{(4)}}{12} + g_{81}^{(4)} - \frac{\eta_7^{(3)}}{3} + 55 \\
\eta_{65}^{(3)} &= \frac{3g_{117}^{(4)}}{2} + 6g_{124}^{(4)} - \frac{\eta_{44}^{(3)}}{4} - 18 \\
\eta_{75}^{(3)} &= -24g_{117}^{(4)} + 6g_{128}^{(4)} - 6g_{129}^{(4)} + 6g_{130}^{(4)} + 2g_{74}^{(4)} + 2g_{76}^{(4)} - 6g_{78}^{(4)} \\
&\quad + \frac{\eta_{10}^{(3)}}{3} - \eta_{11}^{(3)} + 4\eta_{44}^{(3)} + \eta_{70}^{(3)} - \eta_{71}^{(3)} + \eta_{72}^{(3)} + \eta_{73}^{(3)} - \eta_{74}^{(3)} - \frac{1}{2} \\
\eta_{78}^{(3)} &= -3g_{134}^{(4)} + 3g_{135}^{(4)} + \frac{g_{76}^{(4)}}{2} - g_{78}^{(4)} + \eta_{77}^{(3)} - \frac{11}{8} \\
\eta_{79}^{(3)} &= -3g_{117}^{(4)} + 3g_{136}^{(4)} + \frac{g_{69}^{(4)}}{8} - g_{77}^{(4)} + \frac{g_{81}^{(4)}}{2} + \frac{\eta_{44}^{(3)}}{2} - \frac{29}{8} \\
\eta_{81}^{(3)} &= -12g_{117}^{(4)} + 6g_{138}^{(4)} - 6g_{139}^{(4)} - 6g_{142}^{(4)} + 2\eta_{44}^{(3)} - \frac{\eta_{60}^{(3)}}{2} - \frac{\eta_{61}^{(3)}}{2} + 9 \\
\eta_{82}^{(3)} &= -12g_{117}^{(4)} + 6g_{137}^{(4)} + 6g_{138}^{(4)} - 6g_{139}^{(4)} + 36g_{186}^{(4)} + 2\eta_{44}^{(3)} + \eta_{80}^{(3)} - 39 \\
\eta_{86}^{(3)} &= 12g_{117}^{(4)} - 6g_{144}^{(4)} + 6g_{145}^{(4)} + 6g_{146}^{(4)} - 6g_{147}^{(4)} - 6g_{148}^{(4)} - g_{74}^{(4)} - g_{76}^{(4)} \\
&\quad + 3g_{78}^{(4)} - \frac{\eta_{10}^{(3)}}{6} + \frac{\eta_{11}^{(3)}}{2} - 2\eta_{44}^{(3)} + \eta_{83}^{(3)} + \eta_{84}^{(3)} - \eta_{85}^{(3)} + \frac{19}{4} \\
\eta_{87}^{(3)} &= 6g_{149}^{(4)} + \frac{g_{69}^{(4)}}{12} - \frac{g_{77}^{(4)}}{2} + \frac{g_{81}^{(4)}}{2} - \frac{\eta_7^{(3)}}{12} - \frac{265}{16} \\
\eta_{88}^{(3)} &= 3g_{117}^{(4)} + 6g_{133}^{(4)} + \frac{3g_{134}^{(4)}}{2} - \frac{3g_{135}^{(4)}}{2} + 3g_{136}^{(4)} + 6g_{139}^{(4)} - 3g_{144}^{(4)} + 3g_{146}^{(4)} + 36g_{189}^{(4)} \\
&\quad + 18g_{191}^{(4)} - 18g_{192}^{(4)} + 18g_{193}^{(4)} - \frac{g_{69}^{(4)}}{8} - \frac{g_{74}^{(4)}}{4} + 2g_{75}^{(4)} - \frac{g_{76}^{(4)}}{2} + \frac{5g_{78}^{(4)}}{4} + \frac{g_{81}^{(4)}}{2} \\
&\quad - \frac{\eta_{10}^{(3)}}{24} + \frac{\eta_{11}^{(3)}}{8} - \frac{\eta_{44}^{(3)}}{2} - \frac{\eta_{60}^{(3)}}{4} + \frac{\eta_{61}^{(3)}}{4} - \frac{\eta_7^{(3)}}{6} - \frac{\eta_8^{(3)}}{3} + \frac{\eta_{83}^{(3)}}{2} + \frac{\eta_{84}^{(3)}}{2} - \frac{\eta_{85}^{(3)}}{2} - \frac{55}{8} \\
\eta_{90}^{(3)} &= \frac{3g_{117}^{(4)}}{22} + \frac{3g_{150}^{(4)}}{11} - \frac{\eta_{44}^{(3)}}{44} - \frac{\eta_{89}^{(3)}}{22} - \frac{26}{11} \\
\eta_{91}^{(3)} &= \frac{3g_{117}^{(4)}}{11} + \frac{6g_{150}^{(4)}}{11} - \frac{\eta_{44}^{(3)}}{22} - \frac{\eta_{89}^{(3)}}{11} - \frac{8}{11}
\end{aligned}$$

$$\begin{aligned}
\eta_{93}^{(3)} &= -\frac{3g_{117}^{(4)}}{22} - \frac{3g_{153}^{(4)}}{11} + \frac{3g_{156}^{(4)}}{11} + \frac{\eta_{44}^{(3)}}{44} - \frac{\eta_{92}^{(3)}}{22} + \frac{9}{11} \\
\eta_{94}^{(3)} &= -\frac{3g_{117}^{(4)}}{11} - \frac{6g_{153}^{(4)}}{11} + \frac{6g_{156}^{(4)}}{11} + \frac{\eta_{44}^{(3)}}{22} - \frac{\eta_{92}^{(3)}}{11} + \frac{18}{11} \\
\eta_{96}^{(3)} &= \frac{3g_{117}^{(4)}}{44} + \frac{3g_{151}^{(4)}}{22} - \frac{g_{69}^{(4)}}{88} - \frac{g_{88}^{(4)}}{11} - 2g_{94}^{(4)} + \frac{g_{98}^{(4)}}{22} - \frac{\eta_{44}^{(3)}}{88} - \frac{\eta_{95}^{(3)}}{22} + \frac{967}{528} \\
\eta_{98}^{(3)} &= \frac{3g_{117}^{(4)}}{44} + \frac{3g_{151}^{(4)}}{22} + \frac{3g_{153}^{(4)}}{11} - \frac{3g_{154}^{(4)}}{11} - \frac{3g_{156}^{(4)}}{11} - \frac{\eta_{44}^{(3)}}{88} - \frac{\eta_{97}^{(3)}}{22} + \frac{41}{44} \\
\eta_{100}^{(3)} &= \frac{3g_{117}^{(4)}}{22} + \frac{3g_{151}^{(4)}}{11} - \frac{g_{69}^{(4)}}{44} - \frac{2g_{88}^{(4)}}{11} - 2g_{91}^{(4)} + \frac{g_{98}^{(4)}}{11} - \frac{\eta_{44}^{(3)}}{44} - \frac{\eta_{95}^{(3)}}{11} + \frac{263}{264} \\
\eta_{101}^{(3)} &= -\frac{3g_{117}^{(4)}}{44} + \frac{3g_{152}^{(4)}}{22} + \frac{g_{69}^{(4)}}{44} - \frac{2g_{84}^{(4)}}{11} - 4g_{86}^{(4)} + \frac{g_{96}^{(4)}}{11} + \frac{\eta_{44}^{(3)}}{88} - \frac{\eta_{99}^{(3)}}{22} - \frac{28}{33} \\
\eta_{102}^{(3)} &= \frac{3g_{117}^{(4)}}{22} + \frac{3g_{151}^{(4)}}{11} + \frac{6g_{153}^{(4)}}{11} - \frac{6g_{154}^{(4)}}{11} - \frac{6g_{156}^{(4)}}{11} - \frac{\eta_{44}^{(3)}}{44} - \frac{\eta_{97}^{(3)}}{11} - \frac{47}{22} \\
\eta_{104}^{(3)} &= -\frac{3g_{117}^{(4)}}{44} + \frac{3g_{152}^{(4)}}{22} - \frac{6g_{153}^{(4)}}{11} - \frac{\eta_{103}^{(3)}}{22} + \frac{\eta_{44}^{(3)}}{88} + \frac{14}{11} \\
\eta_{105}^{(3)} &= -\frac{3g_{117}^{(4)}}{22} + \frac{3g_{152}^{(4)}}{11} + \frac{g_{69}^{(4)}}{22} - \frac{4g_{84}^{(4)}}{11} - 4g_{85}^{(4)} + \frac{2g_{96}^{(4)}}{11} + \frac{\eta_{44}^{(3)}}{44} - \frac{\eta_{99}^{(3)}}{11} - \frac{1}{33} \\
\eta_{106}^{(3)} &= -\frac{3g_{117}^{(4)}}{22} + \frac{3g_{152}^{(4)}}{11} - \frac{12g_{153}^{(4)}}{11} - \frac{\eta_{103}^{(3)}}{11} + \frac{\eta_{44}^{(3)}}{44} + \frac{50}{11} \\
\eta_{108}^{(3)} &= \frac{3g_{153}^{(4)}}{22} + \frac{g_{69}^{(4)}}{176} - \frac{g_{84}^{(4)}}{22} - g_{86}^{(4)} + \frac{g_{96}^{(4)}}{44} - \frac{\eta_{107}^{(3)}}{22} - \frac{41}{66} \\
\eta_{109}^{(3)} &= \frac{3g_{153}^{(4)}}{11} + \frac{g_{69}^{(4)}}{88} - \frac{g_{84}^{(4)}}{11} - g_{85}^{(4)} + \frac{g_{96}^{(4)}}{22} - \frac{\eta_{107}^{(3)}}{11} - \frac{109}{132} \\
\eta_{111}^{(3)} &= \frac{3g_{117}^{(4)}}{44} + \frac{3g_{154}^{(4)}}{22} - \frac{g_{69}^{(4)}}{176} - \frac{g_{88}^{(4)}}{22} - g_{94}^{(4)} + \frac{g_{98}^{(4)}}{44} - \frac{\eta_{110}^{(3)}}{22} - \frac{\eta_{44}^{(3)}}{88} - \frac{119}{1056} \\
\eta_{113}^{(3)} &= -\frac{3g_{117}^{(4)}}{44} + \frac{3g_{156}^{(4)}}{22} + \frac{g_{69}^{(4)}}{176} - \frac{g_{84}^{(4)}}{22} - g_{86}^{(4)} + \frac{g_{96}^{(4)}}{44} - \frac{\eta_{112}^{(3)}}{22} + \frac{\eta_{44}^{(3)}}{88} - \frac{1}{33} \\
\eta_{114}^{(3)} &= \frac{3g_{117}^{(4)}}{22} + \frac{3g_{154}^{(4)}}{11} - \frac{g_{69}^{(4)}}{88} - \frac{g_{88}^{(4)}}{11} - g_{91}^{(4)} + \frac{g_{98}^{(4)}}{22} - \frac{\eta_{110}^{(3)}}{11} - \frac{\eta_{44}^{(3)}}{44} + \frac{233}{528} \\
\eta_{116}^{(3)} &= \frac{3g_{117}^{(4)}}{44} + \frac{3g_{155}^{(4)}}{11} - \frac{3g_{156}^{(4)}}{22} + \frac{g_{69}^{(4)}}{176} - \frac{g_{84}^{(4)}}{22} - g_{86}^{(4)} + \frac{g_{96}^{(4)}}{44} - \frac{\eta_{115}^{(3)}}{22} - \frac{\eta_{44}^{(3)}}{88} + \frac{37}{66} \\
\eta_{117}^{(3)} &= -\frac{3g_{117}^{(4)}}{22} + \frac{3g_{156}^{(4)}}{11} + \frac{g_{69}^{(4)}}{88} - \frac{g_{84}^{(4)}}{11} - g_{85}^{(4)} + \frac{g_{96}^{(4)}}{22} - \frac{\eta_{112}^{(3)}}{11} + \frac{\eta_{44}^{(3)}}{44} - \frac{85}{132} \\
\eta_{118}^{(3)} &= \frac{3g_{117}^{(4)}}{22} + \frac{6g_{155}^{(4)}}{11} - \frac{3g_{156}^{(4)}}{11} + \frac{g_{69}^{(4)}}{88} - \frac{g_{84}^{(4)}}{11} - g_{85}^{(4)} + \frac{g_{96}^{(4)}}{22} - \frac{\eta_{115}^{(3)}}{11} - \frac{\eta_{44}^{(3)}}{44} - \frac{61}{132} \\
\eta_{120}^{(3)} &= \frac{3g_{153}^{(4)}}{44} - \frac{3g_{154}^{(4)}}{44} - \frac{3g_{156}^{(4)}}{44} + \frac{3g_{157}^{(4)}}{11} - \frac{g_{69}^{(4)}}{352} - \frac{g_{88}^{(4)}}{44} - \frac{g_{94}^{(4)}}{2} + \frac{g_{98}^{(4)}}{88} - \frac{\eta_{119}^{(3)}}{22} + \frac{1645}{2112} \\
\eta_{121}^{(3)} &= \frac{3g_{153}^{(4)}}{22} - \frac{3g_{154}^{(4)}}{22} - \frac{3g_{156}^{(4)}}{22} + \frac{6g_{157}^{(4)}}{11} - \frac{g_{69}^{(4)}}{176} - \frac{g_{88}^{(4)}}{22} - \frac{g_{91}^{(4)}}{2} + \frac{g_{98}^{(4)}}{44} - \frac{\eta_{119}^{(3)}}{11} + \frac{413}{1056} \\
\eta_{122}^{(3)} &= 12g_{158}^{(4)} \\
\eta_{123}^{(3)} &= \frac{3g_{117}^{(4)}}{2} + 3g_{159}^{(4)} - \frac{g_{56}^{(4)}}{2} + g_{57}^{(4)} - \frac{\eta_{44}^{(3)}}{4} - 6
\end{aligned}$$

$$\begin{aligned}
\eta_{124}^{(3)} &= 3g_{117}^{(4)} + 6g_{159}^{(4)} - g_{56}^{(4)} + 2g_{57}^{(4)} - \frac{\eta_{44}^{(3)}}{2} - 12 \\
\eta_{125}^{(3)} &= \frac{3g_{117}^{(4)}}{2} + 3g_{159}^{(4)} - \frac{g_{56}^{(4)}}{2} + g_{57}^{(4)} - \frac{\eta_{44}^{(3)}}{4} + 12 \\
\eta_{129}^{(3)} &= \frac{1}{8} - 2g_{112}^{(4)} \\
\eta_{130}^{(3)} &= \frac{1}{48} - g_{112}^{(4)} \\
\eta_{133}^{(3)} &= 18g_{161}^{(4)} \\
\eta_{134}^{(3)} &= 12g_{162}^{(4)} + 24 \\
\eta_{135}^{(3)} &= -9g_{161}^{(4)} + 6g_{162}^{(4)} - 6 \\
\eta_{139}^{(3)} &= 6g_{166}^{(4)} \\
\eta_{140}^{(3)} &= 2g_{120}^{(4)} - 2g_{122}^{(4)} + 3g_{164}^{(4)} - 7 \\
\eta_{141}^{(3)} &= 2g_{120}^{(4)} - 2g_{122}^{(4)} + 3g_{164}^{(4)} + 5 \\
\eta_{142}^{(3)} &= g_{120}^{(4)} - g_{122}^{(4)} + 6g_{167}^{(4)} + \frac{11}{2} \\
\eta_{143}^{(3)} &= 2g_{120}^{(4)} - 2g_{122}^{(4)} + 3g_{164}^{(4)} + 5 \\
\eta_{144}^{(3)} &= 12g_{165}^{(4)} \\
\eta_{145}^{(3)} &= -2g_{120}^{(4)} + 2g_{122}^{(4)} + 3g_{164}^{(4)} - 24g_{169}^{(4)} - 48g_{186}^{(4)} + 48g_{190}^{(4)} - 29 \\
\eta_{146}^{(3)} &= -12g_{176}^{(4)} + 48g_{186}^{(4)} + 6 \\
\eta_{147}^{(3)} &= 2g_{120}^{(4)} - 2g_{122}^{(4)} + 12g_{169}^{(4)} + 11 \\
\eta_{148}^{(3)} &= 6g_{165}^{(4)} \\
\eta_{149}^{(3)} &= 12g_{166}^{(4)} \\
\eta_{150}^{(3)} &= -2g_{120}^{(4)} + 2g_{122}^{(4)} + 3g_{164}^{(4)} - 24g_{167}^{(4)} - 17 \\
\eta_{151}^{(3)} &= -8g_{117}^{(4)} - 8g_{142}^{(4)} - 12g_{176}^{(4)} + \frac{4\eta_{44}^{(3)}}{3} - \frac{2\eta_{60}^{(3)}}{3} - 2 \\
\eta_{152}^{(3)} &= 6g_{120}^{(4)} - 2g_{122}^{(4)} + 3g_{164}^{(4)} + 24g_{169}^{(4)} + 48g_{186}^{(4)} - 48g_{190}^{(4)} - \frac{2\eta_{53}^{(3)}}{3} + 29 \\
\eta_{153}^{(3)} &= g_{120}^{(4)} - g_{122}^{(4)} + 6g_{168}^{(4)} + \frac{11}{2} \\
\eta_{154}^{(3)} &= -6g_{168}^{(4)} + 6g_{169}^{(4)} + 12g_{186}^{(4)} - 12g_{190}^{(4)} + 3 \\
\eta_{155}^{(3)} &= g_{120}^{(4)} + 6g_{167}^{(4)} - \frac{\eta_{53}^{(3)}}{6} \\
\eta_{156}^{(3)} &= -2g_{117}^{(4)} - 2g_{142}^{(4)} - 12g_{186}^{(4)} + \frac{\eta_{44}^{(3)}}{3} - \frac{\eta_{60}^{(3)}}{6} - 2 \\
\eta_{157}^{(3)} &= g_{120}^{(4)} - 6g_{167}^{(4)} + 6g_{168}^{(4)} + 6g_{169}^{(4)} + 12g_{186}^{(4)} - 12g_{190}^{(4)} - \frac{\eta_{53}^{(3)}}{6} + 3 \\
\eta_{158}^{(3)} &= -\frac{g_{117}^{(4)}}{2} + g_{126}^{(4)} + 4g_{139}^{(4)} - 4g_{140}^{(4)} + 6g_{175}^{(4)} - \frac{g_{69}^{(4)}}{6} + \frac{4g_{75}^{(4)}}{3} - \frac{2g_{80}^{(4)}}{3} - \frac{\eta_{68}^{(3)}}{3} + \frac{41}{3}
\end{aligned}$$

$$\begin{aligned}
\eta_{161}^{(3)} &= -\frac{7\mathfrak{g}_{117}^{(4)}}{2} - \mathfrak{g}_{126}^{(4)} - 4\mathfrak{g}_{136}^{(4)} - 4\mathfrak{g}_{139}^{(4)} - 4\mathfrak{g}_{140}^{(4)} - 6\mathfrak{g}_{175}^{(4)} - \frac{4\mathfrak{g}_{75}^{(4)}}{3} - \frac{2\mathfrak{g}_{80}^{(4)}}{3} \\
&\quad - \frac{2\mathfrak{g}_{81}^{(4)}}{3} + \frac{7\eta_{44}^{(3)}}{12} - \frac{2\eta_{61}^{(3)}}{3} + \frac{\eta_{69}^{(3)}}{3} + \frac{2\eta_7^{(3)}}{9} + \frac{4\eta_8^{(3)}}{9} + \frac{151}{3} \\
\eta_{162}^{(3)} &= 12\mathfrak{g}_{186}^{(4)} - 12\mathfrak{g}_{190}^{(4)} - 3 \\
\eta_{163}^{(3)} &= -2\mathfrak{g}_{117}^{(4)} - 2\mathfrak{g}_{142}^{(4)} - 12\mathfrak{g}_{190}^{(4)} + \frac{\eta_{44}^{(3)}}{3} - \frac{\eta_{60}^{(3)}}{6} - 5 \\
\eta_{164}^{(3)} &= \mathfrak{g}_{120}^{(4)} - 6\mathfrak{g}_{167}^{(4)} + 12\mathfrak{g}_{169}^{(4)} + 12\mathfrak{g}_{186}^{(4)} - 12\mathfrak{g}_{190}^{(4)} - \frac{\eta_{53}^{(3)}}{6} + 3 \\
\eta_{165}^{(3)} &= -3\mathfrak{g}_{117}^{(4)} - \mathfrak{g}_{136}^{(4)} - 2\mathfrak{g}_{139}^{(4)} - 2\mathfrak{g}_{142}^{(4)} - 12\mathfrak{g}_{195}^{(4)} + \frac{\mathfrak{g}_{69}^{(4)}}{72} \\
&\quad - \frac{\mathfrak{g}_{75}^{(4)}}{3} - \frac{\mathfrak{g}_{81}^{(4)}}{6} + \frac{\eta_{44}^{(3)}}{2} - \frac{\eta_{60}^{(3)}}{6} - \frac{\eta_{61}^{(3)}}{6} + \frac{\eta_7^{(3)}}{18} + \frac{\eta_8^{(3)}}{18} + \frac{9}{2} \\
\eta_{166}^{(3)} &= -\mathfrak{g}_{117}^{(4)} - \mathfrak{g}_{136}^{(4)} - 2\mathfrak{g}_{139}^{(4)} - 12\mathfrak{g}_{185}^{(4)} + \frac{\mathfrak{g}_{69}^{(4)}}{72} - \frac{\mathfrak{g}_{75}^{(4)}}{3} - \frac{\mathfrak{g}_{81}^{(4)}}{6} + \frac{\eta_{44}^{(3)}}{6} - \frac{\eta_{61}^{(3)}}{6} + \frac{\eta_7^{(3)}}{18} + \frac{\eta_8^{(3)}}{18} + 5 \\
\eta_{167}^{(3)} &= -\mathfrak{g}_{144}^{(4)} + \mathfrak{g}_{146}^{(4)} + 6\mathfrak{g}_{191}^{(4)} - 6\mathfrak{g}_{192}^{(4)} + 6\mathfrak{g}_{193}^{(4)} - \frac{\mathfrak{g}_{76}^{(4)}}{6} \\
&\quad + \frac{\mathfrak{g}_{78}^{(4)}}{3} - \frac{\eta_{60}^{(3)}}{12} - \frac{\eta_{61}^{(3)}}{12} + \frac{\eta_{83}^{(3)}}{6} + \frac{\eta_{84}^{(3)}}{6} - \frac{\eta_{85}^{(3)}}{6} + \frac{71}{24} \\
\eta_{168}^{(3)} &= 3\mathfrak{g}_{170}^{(4)} - 12\mathfrak{g}_{182}^{(4)} - \frac{\eta_{44}^{(3)}}{12} + \frac{\eta_{66}^{(3)}}{6} - \frac{\eta_{68}^{(3)}}{6} - 2 \\
\eta_{169}^{(3)} &= -\mathfrak{g}_{117}^{(4)} + 4\mathfrak{g}_{126}^{(4)} - 2\mathfrak{g}_{127}^{(4)} + 12\mathfrak{g}_{171}^{(4)} + 48\mathfrak{g}_{182}^{(4)} - \frac{\mathfrak{g}_{69}^{(4)}}{3} + \frac{8\mathfrak{g}_{75}^{(4)}}{3} - \frac{4\mathfrak{g}_{80}^{(4)}}{3} + \frac{\eta_{44}^{(3)}}{3} - \frac{2\eta_{66}^{(3)}}{3} + \frac{79}{3} \\
\eta_{170}^{(3)} &= 6\mathfrak{g}_{170}^{(4)} - 24\mathfrak{g}_{182}^{(4)} - \frac{\eta_{44}^{(3)}}{6} + \frac{\eta_{66}^{(3)}}{3} - \frac{\eta_{68}^{(3)}}{3} + 8 \\
\eta_{171}^{(3)} &= 3\mathfrak{g}_{170}^{(4)} - 12\mathfrak{g}_{182}^{(4)} + \frac{\eta_{44}^{(3)}}{12} - \frac{\eta_{66}^{(3)}}{6} + \frac{\eta_{68}^{(3)}}{6} + 2 \\
\eta_{173}^{(3)} &= 4\mathfrak{g}_{117}^{(4)} + \mathfrak{g}_{126}^{(4)} - \mathfrak{g}_{127}^{(4)} + 4\mathfrak{g}_{139}^{(4)} + 6\mathfrak{g}_{175}^{(4)} - \frac{\mathfrak{g}_{69}^{(4)}}{6} + \frac{4\mathfrak{g}_{75}^{(4)}}{3} - \frac{2\mathfrak{g}_{80}^{(4)}}{3} - \eta_{172}^{(3)} - \frac{2\eta_{44}^{(3)}}{3} - \frac{2\eta_{80}^{(3)}}{3} + \frac{13}{6} \\
\eta_{174}^{(3)} &= -\mathfrak{g}_{117}^{(4)} + 2\mathfrak{g}_{127}^{(4)} + 6\mathfrak{g}_{170}^{(4)} - 24\mathfrak{g}_{182}^{(4)} + \frac{\mathfrak{g}_{69}^{(4)}}{9} + \frac{4\mathfrak{g}_{80}^{(4)}}{3} + \frac{\eta_{66}^{(3)}}{3} - \frac{\eta_{68}^{(3)}}{3} - \frac{2\eta_{69}^{(3)}}{3} - \frac{4\eta_8^{(3)}}{9} - \frac{95}{3} \\
\eta_{175}^{(3)} &= 2\mathfrak{g}_{126}^{(4)} - 2\mathfrak{g}_{127}^{(4)} + 6\mathfrak{g}_{171}^{(4)} + 24\mathfrak{g}_{182}^{(4)} - \frac{2\mathfrak{g}_{69}^{(4)}}{9} + \frac{4\mathfrak{g}_{75}^{(4)}}{3} - \frac{4\mathfrak{g}_{80}^{(4)}}{3} \\
&\quad + \frac{\eta_{44}^{(3)}}{6} - \frac{\eta_{66}^{(3)}}{3} - \frac{\eta_{67}^{(3)}}{3} + \frac{\eta_{68}^{(3)}}{3} + \frac{\eta_{69}^{(3)}}{3} + \frac{2\eta_8^{(3)}}{9} + 27 \\
\eta_{176}^{(3)} &= -\frac{\eta_{44}^{(3)}}{24} + \frac{\eta_{66}^{(3)}}{12} - \frac{\eta_{68}^{(3)}}{12} - \frac{5}{2} \\
\eta_{177}^{(3)} &= \frac{\mathfrak{g}_{126}^{(4)}}{2} - \frac{\mathfrak{g}_{127}^{(4)}}{2} + 2\mathfrak{g}_{133}^{(4)} + 6\mathfrak{g}_{181}^{(4)} + 6\mathfrak{g}_{182}^{(4)} - \frac{\mathfrak{g}_{69}^{(4)}}{12} + \frac{2\mathfrak{g}_{75}^{(4)}}{3} \\
&\quad - \frac{\mathfrak{g}_{80}^{(4)}}{3} + \frac{\eta_{44}^{(3)}}{24} - \frac{\eta_{66}^{(3)}}{12} + \frac{\eta_{68}^{(3)}}{12} - \frac{\eta_{76}^{(3)}}{3} + \frac{31}{12}
\end{aligned}$$



$$\begin{aligned}
\eta_{186}^{(3)} &= \frac{7g_{117}^{(4)}}{4} - 2g_{126}^{(4)} - g_{130}^{(4)} - 8g_{136}^{(4)} - 4g_{137}^{(4)} + 4g_{138}^{(4)} - 12g_{139}^{(4)} - 4g_{141}^{(4)} - 8g_{142}^{(4)} \\
&\quad - 4g_{147}^{(4)} - 4g_{148}^{(4)} - 12g_{175}^{(4)} - 6g_{176}^{(4)} + 6g_{177}^{(4)} - 6g_{178}^{(4)} - 6g_{180}^{(4)} + \frac{g_{69}^{(4)}}{18} - \frac{2g_{74}^{(4)}}{3} \\
&\quad - \frac{8g_{75}^{(4)}}{3} - \frac{2g_{76}^{(4)}}{3} + \frac{2g_{78}^{(4)}}{3} - \frac{2g_{80}^{(4)}}{3} - \frac{4g_{81}^{(4)}}{3} + \frac{\eta_{10}^{(3)}}{9} + \frac{\eta_{11}^{(3)}}{3} - \eta_{184}^{(3)} + \eta_{185}^{(3)} - \frac{\eta_{44}^{(3)}}{4} \\
&\quad + \frac{\eta_{68}^{(3)}}{3} + \frac{\eta_{69}^{(3)}}{3} + \frac{4\eta_7^{(3)}}{9} - \frac{\eta_{70}^{(3)}}{3} + \frac{\eta_{71}^{(3)}}{3} + \frac{\eta_{72}^{(3)}}{3} + \frac{2\eta_8^{(3)}}{3} - \frac{2\eta_{80}^{(3)}}{3} - \frac{4\eta_{83}^{(3)}}{3} + 86 \\
\eta_{190}^{(3)} &= 12g_{165}^{(4)} + \frac{4g_{74}^{(4)}}{3} - \frac{4g_{76}^{(4)}}{3} + \frac{4g_{78}^{(4)}}{3} + \frac{2\eta_{10}^{(3)}}{9} - \frac{2\eta_{11}^{(3)}}{3} - \eta_{178}^{(3)} + \eta_{179}^{(3)} \\
&\quad + \eta_{181}^{(3)} - \eta_{183}^{(3)} + \eta_{189}^{(3)} - \frac{2\eta_{70}^{(3)}}{3} + \frac{2\eta_{71}^{(3)}}{3} + \frac{2\eta_{72}^{(3)}}{3} - \frac{2\eta_{74}^{(3)}}{3} - 1 \\
\eta_{191}^{(3)} &= 5g_{117}^{(4)} - 4g_{126}^{(4)} - 4g_{130}^{(4)} - 16g_{136}^{(4)} - 16g_{139}^{(4)} - 16g_{140}^{(4)} - 16g_{147}^{(4)} + 3g_{165}^{(4)} - 24g_{175}^{(4)} + 24g_{177}^{(4)} \\
&\quad - 24g_{178}^{(4)} - \frac{4g_{74}^{(4)}}{3} - \frac{16g_{75}^{(4)}}{3} - 4g_{76}^{(4)} + 4g_{78}^{(4)} - \frac{8g_{80}^{(4)}}{3} - \frac{8g_{81}^{(4)}}{3} + \frac{2\eta_{10}^{(3)}}{3} + \frac{2\eta_{11}^{(3)}}{3} + \eta_{189}^{(3)} \\
&\quad - \frac{7\eta_{44}^{(3)}}{6} + \frac{4\eta_{69}^{(3)}}{3} + \frac{8\eta_7^{(3)}}{9} - \frac{2\eta_{70}^{(3)}}{3} + \frac{2\eta_{71}^{(3)}}{3} + 2\eta_{72}^{(3)} - \frac{2\eta_{73}^{(3)}}{3} + \frac{2\eta_{74}^{(3)}}{3} + \frac{16\eta_8^{(3)}}{9} + \frac{592}{3} \\
\eta_{192}^{(3)} &= \frac{39g_{117}^{(4)}}{4} - 2g_{126}^{(4)} - g_{130}^{(4)} - 8g_{136}^{(4)} - 8g_{137}^{(4)} + 4g_{138}^{(4)} - 12g_{139}^{(4)} - 4g_{141}^{(4)} - 12g_{142}^{(4)} + 4g_{145}^{(4)} \\
&\quad - 8g_{147}^{(4)} - 8g_{148}^{(4)} - 12g_{175}^{(4)} - 6g_{176}^{(4)} + 12g_{177}^{(4)} - 12g_{178}^{(4)} + 6g_{179}^{(4)} - 12g_{180}^{(4)} - 24g_{186}^{(4)} \\
&\quad + \frac{g_{69}^{(4)}}{18} - \frac{2g_{74}^{(4)}}{3} - \frac{8g_{75}^{(4)}}{3} - \frac{4g_{76}^{(4)}}{3} + 2g_{78}^{(4)} - \frac{2g_{80}^{(4)}}{3} - \frac{4g_{81}^{(4)}}{3} + \frac{\eta_{10}^{(3)}}{9} + \frac{\eta_{11}^{(3)}}{3} - \frac{19\eta_{44}^{(3)}}{12} \\
&\quad + \frac{\eta_{68}^{(3)}}{3} + \frac{\eta_{69}^{(3)}}{3} + \frac{4\eta_7^{(3)}}{9} - \frac{\eta_{70}^{(3)}}{3} + \frac{\eta_{71}^{(3)}}{3} + \frac{\eta_{72}^{(3)}}{3} + \frac{2\eta_8^{(3)}}{3} - \frac{2\eta_{80}^{(3)}}{3} - \frac{2\eta_{85}^{(3)}}{3} + \frac{611}{6} \\
\eta_{195}^{(3)} &= -\frac{g_{117}^{(4)}}{4} + \frac{g_{126}^{(4)}}{2} + 2g_{139}^{(4)} - 2g_{140}^{(4)} + 3g_{175}^{(4)} - \frac{g_{69}^{(4)}}{12} + \frac{2g_{75}^{(4)}}{3} - \frac{g_{80}^{(4)}}{3} + \frac{\eta_{44}^{(3)}}{12} - \frac{\eta_{66}^{(3)}}{6} + \frac{17}{6} \\
\eta_{196}^{(3)} &= g_{117}^{(4)} + 2g_{139}^{(4)} - g_{140}^{(4)} + 12g_{185}^{(4)} - \frac{g_{69}^{(4)}}{24} + \frac{g_{75}^{(4)}}{3} - \frac{g_{80}^{(4)}}{6} - \frac{\eta_{44}^{(3)}}{6} - \frac{\eta_{80}^{(3)}}{6} + \frac{11}{12} \\
\eta_{197}^{(3)} &= -\frac{g_{117}^{(4)}}{4} + \frac{g_{126}^{(4)}}{2} + 2g_{139}^{(4)} - 2g_{140}^{(4)} + 3g_{175}^{(4)} - \frac{g_{69}^{(4)}}{12} + \frac{2g_{75}^{(4)}}{3} - \frac{g_{80}^{(4)}}{3} + \frac{\eta_{44}^{(3)}}{24} - \frac{\eta_{67}^{(3)}}{6} + \frac{23}{6} \\
\eta_{198}^{(3)} &= g_{133}^{(4)} + g_{139}^{(4)} - g_{140}^{(4)} + 6g_{189}^{(4)} - \frac{g_{69}^{(4)}}{24} + \frac{g_{75}^{(4)}}{3} - \frac{g_{80}^{(4)}}{6} - \frac{\eta_{76}^{(3)}}{6} + \frac{23}{12} \\
\eta_{199}^{(3)} &= 4g_{138}^{(4)} - 4g_{139}^{(4)} + 4g_{140}^{(4)} - 4g_{141}^{(4)} + 6g_{176}^{(4)} - \frac{31}{2} \\
\eta_{200}^{(3)} &= g_{138}^{(4)} - g_{139}^{(4)} + g_{140}^{(4)} - g_{141}^{(4)} + 6g_{186}^{(4)} - \frac{7}{8} \\
\eta_{201}^{(3)} &= -\frac{g_{120}^{(4)}}{2} + \frac{g_{122}^{(4)}}{2} + g_{138}^{(4)} - g_{139}^{(4)} + g_{140}^{(4)} - g_{141}^{(4)} - 3g_{169}^{(4)} + 6g_{190}^{(4)} - \frac{53}{8} \\
\eta_{206}^{(3)} &= g_{117}^{(4)} - \frac{g_{131}^{(4)}}{2} - g_{135}^{(4)} - g_{144}^{(4)} + g_{146}^{(4)} - g_{147}^{(4)} - 3g_{184}^{(4)} - 6g_{192}^{(4)} + 6g_{193}^{(4)} - \frac{g_{74}^{(4)}}{6} - \frac{g_{76}^{(4)}}{3} \\
&\quad + \frac{g_{78}^{(4)}}{2} + \frac{\eta_{10}^{(3)}}{36} + \frac{\eta_{11}^{(3)}}{12} - \frac{\eta_{44}^{(3)}}{6} - \frac{\eta_{60}^{(3)}}{12} + \frac{\eta_{61}^{(3)}}{12} - \frac{\eta_{77}^{(3)}}{3} + \frac{\eta_{83}^{(3)}}{6} + \frac{\eta_{84}^{(3)}}{6} - \frac{\eta_{85}^{(3)}}{6} - \frac{1}{8}
\end{aligned}$$

$$\begin{aligned}
\eta_{207}^{(3)} &= 2g_{117}^{(4)} + g_{129}^{(4)} - 2g_{130}^{(4)} + 2g_{134}^{(4)} + 2g_{135}^{(4)} + 6g_{136}^{(4)} + 8g_{139}^{(4)} + 4g_{140}^{(4)} + 6g_{144}^{(4)} \\
&\quad - 4g_{145}^{(4)} - 2g_{146}^{(4)} + 8g_{147}^{(4)} + 6g_{177}^{(4)} - 6g_{179}^{(4)} + 6g_{180}^{(4)} + 48g_{185}^{(4)} + 24g_{187}^{(4)} - 24g_{188}^{(4)} \\
&\quad + 12g_{191}^{(4)} + 12g_{192}^{(4)} - 12g_{193}^{(4)} + \frac{g_{69}^{(4)}}{36} + \frac{2g_{74}^{(4)}}{3} + \frac{4g_{75}^{(4)}}{3} + \frac{2g_{76}^{(4)}}{3} - \frac{2g_{78}^{(4)}}{3} + \frac{2g_{80}^{(4)}}{3} \\
&\quad + g_{81}^{(4)} - \frac{\eta_{10}^{(3)}}{9} - \frac{\eta_{11}^{(3)}}{3} + \eta_{202}^{(3)} - \frac{\eta_{44}^{(3)}}{4} + \frac{\eta_{60}^{(3)}}{2} + \frac{\eta_{61}^{(3)}}{6} + \frac{\eta_{68}^{(3)}}{6} - \frac{\eta_{69}^{(3)}}{6} - \frac{\eta_7^{(3)}}{3} \\
&\quad - \frac{\eta_{70}^{(3)}}{6} + \frac{\eta_{71}^{(3)}}{2} - \frac{\eta_{72}^{(3)}}{6} - \frac{\eta_{73}^{(3)}}{6} + \frac{\eta_{74}^{(3)}}{6} - \frac{4\eta_8^{(3)}}{9} - \eta_{83}^{(3)} - \eta_{84}^{(3)} + \eta_{85}^{(3)} - \frac{167}{3} \\
\eta_{208}^{(3)} &= 3g_{136}^{(4)} + g_{137}^{(4)} - g_{138}^{(4)} + 5g_{139}^{(4)} + g_{141}^{(4)} + 2g_{142}^{(4)} + 2g_{144}^{(4)} - g_{145}^{(4)} - g_{146}^{(4)} + 2g_{147}^{(4)} \\
&\quad + g_{148}^{(4)} + 24g_{185}^{(4)} + 6g_{186}^{(4)} + 6g_{187}^{(4)} + \frac{g_{74}^{(4)}}{3} + \frac{2g_{75}^{(4)}}{3} + \frac{g_{76}^{(4)}}{3} - \frac{2g_{78}^{(4)}}{3} + \frac{g_{80}^{(4)}}{6} \\
&\quad + \frac{g_{81}^{(4)}}{2} - \frac{\eta_{11}^{(3)}}{6} + \eta_{204}^{(3)} + \frac{\eta_{60}^{(3)}}{6} + \frac{\eta_{61}^{(3)}}{6} - \frac{\eta_7^{(3)}}{6} - \frac{\eta_8^{(3)}}{6} + \frac{\eta_{80}^{(3)}}{6} - \frac{\eta_{84}^{(3)}}{3} + \frac{\eta_{85}^{(3)}}{3} - \frac{183}{8} \\
\eta_{209}^{(3)} &= -g_{117}^{(4)} + \frac{g_{131}^{(4)}}{2} + g_{135}^{(4)} + g_{144}^{(4)} - g_{145}^{(4)} + g_{147}^{(4)} + 3g_{184}^{(4)} + 6g_{191}^{(4)} + \frac{g_{74}^{(4)}}{6} + \frac{g_{76}^{(4)}}{3} - \frac{g_{78}^{(4)}}{2} \\
&\quad - \frac{\eta_{10}^{(3)}}{36} - \frac{\eta_{11}^{(3)}}{12} + \eta_{205}^{(3)} + \frac{\eta_{44}^{(3)}}{6} + \frac{\eta_{60}^{(3)}}{12} - \frac{\eta_{61}^{(3)}}{12} + \frac{\eta_{77}^{(3)}}{3} - \frac{\eta_{83}^{(3)}}{6} - \frac{\eta_{84}^{(3)}}{6} + \frac{\eta_{85}^{(3)}}{6} + \frac{3}{2} \\
\eta_{210}^{(3)} &= \frac{g_{117}^{(4)}}{4} - \frac{g_{126}^{(4)}}{2} - 8g_{136}^{(4)} - 10g_{139}^{(4)} - 6g_{140}^{(4)} - 4g_{144}^{(4)} + 4g_{146}^{(4)} - 8g_{147}^{(4)} - 3g_{175}^{(4)} - 48g_{185}^{(4)} - 24g_{187}^{(4)} \\
&\quad + 24g_{188}^{(4)} - \frac{g_{69}^{(4)}}{36} - \frac{2g_{74}^{(4)}}{3} - 2g_{75}^{(4)} - \frac{4g_{76}^{(4)}}{3} + 2g_{78}^{(4)} - g_{80}^{(4)} - \frac{4g_{81}^{(4)}}{3} + \frac{\eta_{10}^{(3)}}{9} + \frac{\eta_{11}^{(3)}}{3} - \frac{\eta_{44}^{(3)}}{8} \\
&\quad - \frac{\eta_{60}^{(3)}}{3} - \frac{\eta_{61}^{(3)}}{3} - \frac{\eta_{68}^{(3)}}{6} + \frac{\eta_{69}^{(3)}}{3} + \frac{4\eta_7^{(3)}}{9} + \frac{\eta_{72}^{(3)}}{3} - \frac{\eta_{73}^{(3)}}{6} + \frac{2\eta_8^{(3)}}{3} + \frac{2\eta_{83}^{(3)}}{3} + \frac{2\eta_{84}^{(3)}}{3} - \frac{2\eta_{85}^{(3)}}{3} + 81 \\
\eta_{211}^{(3)} &= \frac{9g_{117}^{(4)}}{4} - \frac{g_{126}^{(4)}}{2} + g_{129}^{(4)} - 2g_{130}^{(4)} + 2g_{134}^{(4)} + 2g_{135}^{(4)} - 2g_{136}^{(4)} - 2g_{139}^{(4)} - 2g_{140}^{(4)} + 2g_{144}^{(4)} \\
&\quad - 2g_{146}^{(4)} - 3g_{175}^{(4)} + 12g_{177}^{(4)} - 6g_{178}^{(4)} + 12g_{191}^{(4)} + 12g_{192}^{(4)} - 12g_{193}^{(4)} - \frac{g_{74}^{(4)}}{3} - \frac{2g_{75}^{(4)}}{3} \\
&\quad - \frac{g_{76}^{(4)}}{3} + g_{78}^{(4)} - \frac{g_{80}^{(4)}}{3} - \frac{g_{81}^{(4)}}{3} - \frac{\eta_{10}^{(3)}}{18} + \frac{\eta_{11}^{(3)}}{6} + \eta_{203}^{(3)} - \frac{3\eta_{44}^{(3)}}{8} + \frac{\eta_{60}^{(3)}}{6} - \frac{\eta_{61}^{(3)}}{6} \\
&\quad + \frac{\eta_{69}^{(3)}}{6} + \frac{\eta_7^{(3)}}{9} + \frac{\eta_{71}^{(3)}}{3} - \frac{\eta_{73}^{(3)}}{3} + \frac{\eta_{74}^{(3)}}{3} + \frac{2\eta_8^{(3)}}{9} - \frac{\eta_{83}^{(3)}}{3} - \frac{\eta_{84}^{(3)}}{3} + \frac{\eta_{85}^{(3)}}{3} + \frac{313}{12} \\
\eta_{212}^{(3)} &= 4g_{144}^{(4)} - 4g_{146}^{(4)} + 6g_{177}^{(4)} - 6g_{178}^{(4)} + 6g_{179}^{(4)} - 6g_{180}^{(4)} + \frac{g_{74}^{(4)}}{3} + \frac{g_{76}^{(4)}}{3} - g_{78}^{(4)} + \frac{\eta_{10}^{(3)}}{18} \\
&\quad - \frac{\eta_{11}^{(3)}}{6} + \frac{\eta_{60}^{(3)}}{3} + \frac{\eta_{61}^{(3)}}{3} - \frac{\eta_{70}^{(3)}}{6} + \frac{\eta_{71}^{(3)}}{6} + \frac{\eta_{72}^{(3)}}{6} - \frac{\eta_{74}^{(3)}}{6} - \frac{2\eta_{83}^{(3)}}{3} - \frac{2\eta_{84}^{(3)}}{3} + \frac{2\eta_{85}^{(3)}}{3} - \frac{37}{12} \\
\eta_{213}^{(3)} &= 2g_{117}^{(4)} - 3g_{136}^{(4)} - 2g_{137}^{(4)} + g_{138}^{(4)} - 5g_{139}^{(4)} - g_{141}^{(4)} - 3g_{142}^{(4)} - 2g_{144}^{(4)} + g_{145}^{(4)} + 2g_{146}^{(4)} - 3g_{147}^{(4)} \\
&\quad - 2g_{148}^{(4)} - 24g_{185}^{(4)} - 12g_{186}^{(4)} - 6g_{187}^{(4)} - \frac{g_{74}^{(4)}}{3} - \frac{2g_{75}^{(4)}}{3} - \frac{g_{76}^{(4)}}{2} + g_{78}^{(4)} - \frac{g_{80}^{(4)}}{6} - \frac{g_{81}^{(4)}}{2} \\
&\quad + \frac{\eta_{11}^{(3)}}{6} - \frac{\eta_{44}^{(3)}}{3} - \frac{\eta_{60}^{(3)}}{6} - \frac{\eta_{61}^{(3)}}{6} + \frac{\eta_7^{(3)}}{6} + \frac{\eta_8^{(3)}}{6} - \frac{\eta_{80}^{(3)}}{6} + \frac{\eta_{83}^{(3)}}{3} + \frac{\eta_{84}^{(3)}}{3} - \frac{\eta_{85}^{(3)}}{2} + \frac{677}{24}
\end{aligned}$$

$$\begin{aligned}
\eta_{214}^{(3)} &= -\frac{\mathfrak{g}_{117}^{(4)}}{4} + \frac{\mathfrak{g}_{126}^{(4)}}{2} - 2\mathfrak{g}_{132}^{(4)} + 2\mathfrak{g}_{133}^{(4)} + 6\mathfrak{g}_{181}^{(4)} + 6\mathfrak{g}_{182}^{(4)} \\
&\quad - \frac{\mathfrak{g}_{69}^{(4)}}{12} + \frac{2\mathfrak{g}_{75}^{(4)}}{3} - \frac{\mathfrak{g}_{80}^{(4)}}{3} + \frac{\eta_{44}^{(3)}}{24} - \frac{\eta_{66}^{(3)}}{12} - \frac{\eta_{68}^{(3)}}{12} + \frac{59}{6} \\
\eta_{215}^{(3)} &= \mathfrak{g}_{117}^{(4)} - \mathfrak{g}_{132}^{(4)} + \mathfrak{g}_{133}^{(4)} + \mathfrak{g}_{139}^{(4)} + 6\mathfrak{g}_{189}^{(4)} - \frac{\mathfrak{g}_{69}^{(4)}}{24} + \frac{\mathfrak{g}_{75}^{(4)}}{3} - \frac{\mathfrak{g}_{80}^{(4)}}{6} - \frac{\eta_{44}^{(3)}}{6} - \frac{\eta_{80}^{(3)}}{6} - \frac{13}{12} \\
\eta_{216}^{(3)} &= -\frac{\mathfrak{g}_{117}^{(4)}}{4} + \frac{\mathfrak{g}_{127}^{(4)}}{2} + \frac{\mathfrak{g}_{69}^{(4)}}{36} + \frac{\mathfrak{g}_{80}^{(4)}}{3} + \frac{\eta_{66}^{(3)}}{12} - \frac{\eta_{68}^{(3)}}{12} - \frac{\eta_{69}^{(3)}}{6} - \frac{\eta_8^{(3)}}{9} - \frac{59}{12} \\
\eta_{217}^{(3)} &= -\mathfrak{g}_{117}^{(4)} + \frac{\mathfrak{g}_{126}^{(4)}}{2} - \frac{\mathfrak{g}_{127}^{(4)}}{2} - \mathfrak{g}_{136}^{(4)} - 2\mathfrak{g}_{139}^{(4)} + \mathfrak{g}_{144}^{(4)} - \mathfrak{g}_{146}^{(4)} + 6\mathfrak{g}_{181}^{(4)} + 6\mathfrak{g}_{182}^{(4)} - 12\mathfrak{g}_{189}^{(4)} \\
&\quad - 6\mathfrak{g}_{191}^{(4)} + 6\mathfrak{g}_{192}^{(4)} - 6\mathfrak{g}_{193}^{(4)} - \frac{\mathfrak{g}_{69}^{(4)}}{24} + \frac{\mathfrak{g}_{76}^{(4)}}{6} - \frac{\mathfrak{g}_{78}^{(4)}}{3} - \frac{\mathfrak{g}_{80}^{(4)}}{3} - \frac{\mathfrak{g}_{81}^{(4)}}{6} + \frac{5\eta_{44}^{(3)}}{24} + \frac{\eta_{60}^{(3)}}{12} \\
&\quad - \frac{\eta_{61}^{(3)}}{12} - \frac{\eta_{66}^{(3)}}{12} - \frac{\eta_{67}^{(3)}}{12} + \frac{\eta_{68}^{(3)}}{12} + \frac{\eta_{69}^{(3)}}{12} + \frac{\eta_7^{(3)}}{18} + \frac{\eta_8^{(3)}}{9} - \frac{\eta_{83}^{(3)}}{6} - \frac{\eta_{84}^{(3)}}{6} + \frac{\eta_{85}^{(3)}}{6} + \frac{31}{24} \\
\eta_{219}^{(3)} &= \mathfrak{g}_{117}^{(4)} - \frac{\mathfrak{g}_{134}^{(4)}}{2} - \frac{\mathfrak{g}_{135}^{(4)}}{2} - \mathfrak{g}_{136}^{(4)} - \mathfrak{g}_{137}^{(4)} + \mathfrak{g}_{138}^{(4)} - \mathfrak{g}_{139}^{(4)} - \mathfrak{g}_{141}^{(4)} - 2\mathfrak{g}_{142}^{(4)} - \mathfrak{g}_{144}^{(4)} + \mathfrak{g}_{146}^{(4)} \\
&\quad - \mathfrak{g}_{147}^{(4)} - \mathfrak{g}_{148}^{(4)} - 6\mathfrak{g}_{190}^{(4)} - 6\mathfrak{g}_{192}^{(4)} - \frac{\mathfrak{g}_{69}^{(4)}}{36} - \frac{\mathfrak{g}_{74}^{(4)}}{4} - \frac{\mathfrak{g}_{76}^{(4)}}{6} + \frac{\mathfrak{g}_{78}^{(4)}}{4} - \frac{\mathfrak{g}_{80}^{(4)}}{6} - \frac{\mathfrak{g}_{81}^{(4)}}{6} + \frac{\eta_{10}^{(3)}}{72} \\
&\quad + \frac{\eta_{11}^{(3)}}{8} - \frac{\eta_{44}^{(3)}}{6} - \frac{\eta_{60}^{(3)}}{12} + \frac{\eta_{61}^{(3)}}{12} + \frac{\eta_7^{(3)}}{18} + \frac{\eta_8^{(3)}}{18} - \frac{\eta_{80}^{(3)}}{6} - \frac{\eta_{83}^{(3)}}{6} + \frac{\eta_{84}^{(3)}}{6} - \frac{\eta_{85}^{(3)}}{6} + 11 \\
\eta_{220}^{(3)} &= -\frac{\mathfrak{g}_{117}^{(4)}}{2} + 2\mathfrak{g}_{126}^{(4)} + 2\mathfrak{g}_{130}^{(4)} - 2\mathfrak{g}_{134}^{(4)} - 2\mathfrak{g}_{135}^{(4)} + 6\mathfrak{g}_{136}^{(4)} + 8\mathfrak{g}_{139}^{(4)} + 4\mathfrak{g}_{140}^{(4)} - 2\mathfrak{g}_{144}^{(4)} + 2\mathfrak{g}_{146}^{(4)} \\
&\quad + 4\mathfrak{g}_{147}^{(4)} + 12\mathfrak{g}_{175}^{(4)} - 12\mathfrak{g}_{177}^{(4)} + 12\mathfrak{g}_{178}^{(4)} - 12\mathfrak{g}_{191}^{(4)} - 12\mathfrak{g}_{192}^{(4)} + 12\mathfrak{g}_{193}^{(4)} - \frac{\mathfrak{g}_{69}^{(4)}}{12} + \frac{\mathfrak{g}_{74}^{(4)}}{3} \\
&\quad + \frac{8\mathfrak{g}_{75}^{(4)}}{3} + \mathfrak{g}_{76}^{(4)} - \mathfrak{g}_{78}^{(4)} + \frac{2\mathfrak{g}_{80}^{(4)}}{3} + \mathfrak{g}_{81}^{(4)} - \frac{\eta_{10}^{(3)}}{6} - \frac{\eta_{11}^{(3)}}{6} + \frac{\eta_{44}^{(3)}}{6} - \frac{\eta_{60}^{(3)}}{6} + \frac{\eta_{61}^{(3)}}{6} - \frac{\eta_{68}^{(3)}}{6} - \frac{\eta_{69}^{(3)}}{2} \\
&\quad - \frac{\eta_7^{(3)}}{3} + \frac{\eta_{70}^{(3)}}{3} - \frac{\eta_{71}^{(3)}}{3} - \frac{2\eta_{72}^{(3)}}{3} + \frac{\eta_{73}^{(3)}}{6} - \frac{\eta_{74}^{(3)}}{3} - \frac{2\eta_8^{(3)}}{3} + \frac{\eta_{83}^{(3)}}{3} + \frac{\eta_{84}^{(3)}}{3} - \frac{\eta_{85}^{(3)}}{3} - \frac{833}{12} \\
\eta_{221}^{(3)} &= 3\mathfrak{g}_{117}^{(4)} - \frac{\mathfrak{g}_{134}^{(4)}}{2} - \frac{\mathfrak{g}_{135}^{(4)}}{2} - \mathfrak{g}_{136}^{(4)} - 2\mathfrak{g}_{137}^{(4)} + \mathfrak{g}_{138}^{(4)} - \mathfrak{g}_{139}^{(4)} - \mathfrak{g}_{141}^{(4)} - 3\mathfrak{g}_{142}^{(4)} \\
&\quad - \mathfrak{g}_{144}^{(4)} + \mathfrak{g}_{145}^{(4)} + \mathfrak{g}_{146}^{(4)} - 2\mathfrak{g}_{147}^{(4)} - 2\mathfrak{g}_{148}^{(4)} - 6\mathfrak{g}_{186}^{(4)} - 6\mathfrak{g}_{190}^{(4)} - 6\mathfrak{g}_{191}^{(4)} - 6\mathfrak{g}_{193}^{(4)} \\
&\quad - \frac{\mathfrak{g}_{69}^{(4)}}{36} - \frac{\mathfrak{g}_{74}^{(4)}}{4} - \frac{\mathfrak{g}_{76}^{(4)}}{3} + \frac{7\mathfrak{g}_{78}^{(4)}}{12} - \frac{\mathfrak{g}_{80}^{(4)}}{6} - \frac{\mathfrak{g}_{81}^{(4)}}{6} + \frac{\eta_{10}^{(3)}}{72} + \frac{\eta_{11}^{(3)}}{8} - \frac{\eta_{44}^{(3)}}{2} \\
&\quad - \frac{\eta_{60}^{(3)}}{12} + \frac{\eta_{61}^{(3)}}{12} + \frac{\eta_7^{(3)}}{18} + \frac{\eta_8^{(3)}}{18} - \frac{\eta_{80}^{(3)}}{6} + \frac{\eta_{83}^{(3)}}{6} + \frac{\eta_{84}^{(3)}}{6} - \frac{\eta_{85}^{(3)}}{3} + \frac{359}{24} \\
\eta_{222}^{(3)} &= 2\mathfrak{g}_{117}^{(4)} - \mathfrak{g}_{137}^{(4)} - \mathfrak{g}_{142}^{(4)} + \mathfrak{g}_{144}^{(4)} + 2\mathfrak{g}_{145}^{(4)} - 2\mathfrak{g}_{146}^{(4)} - \mathfrak{g}_{147}^{(4)} - \mathfrak{g}_{148}^{(4)} - 6\mathfrak{g}_{186}^{(4)} \\
&\quad + 18\mathfrak{g}_{196}^{(4)} - 18\mathfrak{g}_{197}^{(4)} - \frac{\eta_{44}^{(3)}}{3} + \frac{\eta_{60}^{(3)}}{12} + \frac{\eta_{61}^{(3)}}{12} + \frac{\eta_{83}^{(3)}}{6} - \frac{\eta_{84}^{(3)}}{6} + \frac{9}{8}
\end{aligned}$$

$$\begin{aligned}
\eta_{223}^{(3)} &= -\frac{\mathfrak{g}_{117}^{(4)}}{4} - \frac{\mathfrak{g}_{132}^{(4)}}{2} + \mathfrak{g}_{133}^{(4)} - \frac{\mathfrak{g}_{136}^{(4)}}{4} - \frac{\mathfrak{g}_{139}^{(4)}}{2} + \frac{\mathfrak{g}_{144}^{(4)}}{4} - \frac{\mathfrak{g}_{146}^{(4)}}{4} - 3\mathfrak{g}_{189}^{(4)} - \frac{3\mathfrak{g}_{191}^{(4)}}{2} \\
&\quad + \frac{3\mathfrak{g}_{192}^{(4)}}{2} - \frac{3\mathfrak{g}_{193}^{(4)}}{2} + 18\mathfrak{g}_{198}^{(4)} - \frac{5\mathfrak{g}_{69}^{(4)}}{288} + \frac{\mathfrak{g}_{75}^{(4)}}{12} + \frac{\mathfrak{g}_{76}^{(4)}}{24} - \frac{\mathfrak{g}_{78}^{(4)}}{12} - \frac{\mathfrak{g}_{80}^{(4)}}{12} - \frac{\mathfrak{g}_{81}^{(4)}}{24} \\
&\quad + \frac{\eta_{44}^{(3)}}{24} + \frac{\eta_{60}^{(3)}}{48} - \frac{\eta_{61}^{(3)}}{48} + \frac{\eta_7^{(3)}}{72} - \frac{\eta_{76}^{(3)}}{12} + \frac{\eta_8^{(3)}}{72} - \frac{\eta_{83}^{(3)}}{24} - \frac{\eta_{84}^{(3)}}{24} + \frac{\eta_{85}^{(3)}}{24} + \frac{123}{32} \\
\eta_{225}^{(3)} &= 4\mathfrak{g}_{160}^{(4)} + \frac{2\eta_{126}^{(3)}}{3} - \frac{4\eta_{127}^{(3)}}{3} + 2\eta_{224}^{(3)} + \frac{2}{3} \\
\eta_{227}^{(3)} &= \frac{\eta_{126}^{(3)}}{3} - \frac{\eta_{127}^{(3)}}{3} + \eta_{224}^{(3)} + \frac{4}{3} \\
\eta_{228}^{(3)} &= \frac{\eta_{226}^{(3)}}{2} \\
\eta_{229}^{(3)} &= \frac{2\eta_{126}^{(3)}}{3} - \frac{2\eta_{127}^{(3)}}{3} + 2\eta_{224}^{(3)} - \frac{4}{3} \\
\eta_{230}^{(3)} &= -\mathfrak{g}_{160}^{(4)} + \frac{\eta_{127}^{(3)}}{6} - \frac{1}{2} \\
\eta_{232}^{(3)} &= \mathfrak{g}_{111}^{(4)} + \frac{\mathfrak{g}_{117}^{(4)}}{2} - \eta_{231}^{(3)} - \frac{\eta_{40}^{(3)}}{3} - \frac{\eta_{44}^{(3)}}{12} + \frac{5}{2} \\
\eta_{233}^{(3)} &= -\frac{\eta_{126}^{(3)}}{6} + \frac{\eta_{127}^{(3)}}{6} + \frac{4}{3} \\
\eta_{234}^{(3)} &= -\frac{\eta_{126}^{(3)}}{12} + \frac{\eta_{127}^{(3)}}{12} + \frac{5}{3} \\
\eta_{235}^{(3)} &= \mathfrak{g}_{160}^{(4)} - \frac{\eta_{127}^{(3)}}{6} + \frac{7}{2} \\
\eta_{238}^{(3)} &= -14\mathfrak{g}_{161}^{(4)} - 4\mathfrak{g}_{163}^{(4)} - \frac{4\eta_{136}^{(3)}}{3} + \frac{2\eta_{137}^{(3)}}{3} + \frac{4\eta_{138}^{(3)}}{3} + 2\eta_{236}^{(3)} + \frac{2}{3} \\
\eta_{240}^{(3)} &= -6\mathfrak{g}_{161}^{(4)} - \frac{2\eta_{136}^{(3)}}{3} + \frac{2\eta_{137}^{(3)}}{3} + 2\eta_{236}^{(3)} \\
\eta_{242}^{(3)} &= \eta_{237}^{(3)} \\
\eta_{243}^{(3)} &= -8\mathfrak{g}_{161}^{(4)} - 4\mathfrak{g}_{163}^{(4)} - \frac{2\eta_{136}^{(3)}}{3} + \frac{2\eta_{137}^{(3)}}{3} + \frac{2\eta_{138}^{(3)}}{3} + 2\eta_{236}^{(3)} + 2 \\
\eta_{244}^{(3)} &= -4\mathfrak{g}_{161}^{(4)} - 2\mathfrak{g}_{163}^{(4)} - \frac{\eta_{136}^{(3)}}{3} + \frac{\eta_{137}^{(3)}}{3} + \frac{\eta_{138}^{(3)}}{3} + \eta_{236}^{(3)} - 1 \\
\eta_{245}^{(3)} &= -\frac{\mathfrak{g}_{161}^{(4)}}{2} - \mathfrak{g}_{163}^{(4)} + \frac{\eta_{138}^{(3)}}{6} + \frac{1}{2} \\
\eta_{246}^{(3)} &= -\mathfrak{g}_{161}^{(4)} - \frac{\mathfrak{g}_{163}^{(4)}}{2} - \frac{\eta_{136}^{(3)}}{12} + \frac{\eta_{137}^{(3)}}{12} + \frac{\eta_{138}^{(3)}}{12} - \frac{3}{4} \\
\eta_{247}^{(3)} &= -\frac{\eta_{137}^{(3)}}{6} + \frac{\eta_{138}^{(3)}}{6} - \frac{4}{3} \\
\eta_{248}^{(3)} &= -\frac{3\mathfrak{g}_{161}^{(4)}}{2} - \frac{\eta_{136}^{(3)}}{6} + \frac{\eta_{138}^{(3)}}{6} - \frac{4}{3} \\
\eta_{249}^{(3)} &= -3\mathfrak{g}_{161}^{(4)} - \frac{\eta_{136}^{(3)}}{3} + \frac{\eta_{137}^{(3)}}{6} + \frac{\eta_{138}^{(3)}}{6} - \frac{10}{3}
\end{aligned}$$

$$\begin{aligned}
\eta_{254}^{(3)} &= -3g_{117}^{(4)} - \frac{8g_{126}^{(4)}}{3} - \frac{4g_{129}^{(4)}}{3} + \frac{4g_{130}^{(4)}}{3} - \frac{32g_{136}^{(4)}}{3} - \frac{32g_{139}^{(4)}}{3} - \frac{32g_{140}^{(4)}}{3} - \frac{32g_{147}^{(4)}}{3} \\
&\quad - 6g_{165}^{(4)} - 2g_{172}^{(4)} + 4g_{173}^{(4)} - 16g_{175}^{(4)} + 16g_{177}^{(4)} - 16g_{178}^{(4)} - \frac{8g_{74}^{(4)}}{9} - \frac{32g_{75}^{(4)}}{9} \\
&\quad - \frac{8g_{78}^{(4)}}{9} - \frac{16g_{80}^{(4)}}{9} - \frac{16g_{81}^{(4)}}{9} + \frac{4\eta_{10}^{(3)}}{27} + \frac{4\eta_{11}^{(3)}}{9} - \frac{2\eta_{181}^{(3)}}{3} + \frac{4\eta_{183}^{(3)}}{3} - \frac{2\eta_{189}^{(3)}}{3} \\
&\quad + \eta_{251}^{(3)} + \frac{4\eta_{44}^{(3)}}{9} + \frac{8\eta_{69}^{(3)}}{9} + \frac{16\eta_7^{(3)}}{27} + \frac{4\eta_{70}^{(3)}}{9} - \frac{4\eta_{71}^{(3)}}{9} + \frac{4\eta_{72}^{(3)}}{9} + \frac{32\eta_8^{(3)}}{27} + \frac{1192}{9} \\
\eta_{255}^{(3)} &= -\frac{7g_{117}^{(4)}}{3} - \frac{4g_{129}^{(4)}}{3} - \frac{4g_{130}^{(4)}}{3} + 10g_{165}^{(4)} - 2g_{172}^{(4)} - 4g_{173}^{(4)} + \frac{8g_{74}^{(4)}}{9} - \frac{16g_{76}^{(4)}}{9} + \frac{8g_{78}^{(4)}}{9} + \frac{4\eta_{10}^{(3)}}{9} \\
&\quad - \frac{4\eta_{11}^{(3)}}{9} - \frac{2\eta_{178}^{(3)}}{3} + \frac{2\eta_{181}^{(3)}}{3} - \frac{2\eta_{183}^{(3)}}{3} + 2\eta_{189}^{(3)} + 2\eta_{253}^{(3)} + \frac{2\eta_{44}^{(3)}}{9} - \frac{4\eta_{70}^{(3)}}{9} + \frac{4\eta_{71}^{(3)}}{9} + \frac{4\eta_{72}^{(3)}}{3} + \frac{2}{9} \\
\eta_{256}^{(3)} &= -3g_{117}^{(4)} - \frac{8g_{126}^{(4)}}{3} - \frac{4g_{129}^{(4)}}{3} + \frac{4g_{130}^{(4)}}{3} - \frac{32g_{136}^{(4)}}{3} - \frac{32g_{139}^{(4)}}{3} - \frac{32g_{140}^{(4)}}{3} - \frac{32g_{147}^{(4)}}{3} \\
&\quad - 10g_{165}^{(4)} - 2g_{172}^{(4)} + 4g_{173}^{(4)} - 16g_{175}^{(4)} + 16g_{177}^{(4)} - 16g_{178}^{(4)} - \frac{8g_{74}^{(4)}}{9} - \frac{32g_{75}^{(4)}}{9} - \frac{8g_{78}^{(4)}}{9} \\
&\quad - \frac{16g_{80}^{(4)}}{9} - \frac{16g_{81}^{(4)}}{9} + \frac{4\eta_{10}^{(3)}}{27} + \frac{4\eta_{11}^{(3)}}{9} + \frac{2\eta_{178}^{(3)}}{3} - \frac{2\eta_{179}^{(3)}}{3} - \frac{2\eta_{181}^{(3)}}{3} + \frac{4\eta_{183}^{(3)}}{3} - \frac{2\eta_{189}^{(3)}}{3} \\
&\quad + \eta_{251}^{(3)} + \frac{4\eta_{44}^{(3)}}{9} + \frac{8\eta_{69}^{(3)}}{9} + \frac{16\eta_7^{(3)}}{27} + \frac{4\eta_{70}^{(3)}}{9} - \frac{4\eta_{71}^{(3)}}{9} + \frac{4\eta_{72}^{(3)}}{9} + \frac{32\eta_8^{(3)}}{27} + \frac{1192}{9} \\
\eta_{257}^{(3)} &= -\frac{2g_{131}^{(4)}}{3} - 2g_{174}^{(4)} - \frac{\eta_{193}^{(3)}}{3} + \frac{1}{2} \\
\eta_{258}^{(3)} &= -4g_{117}^{(4)} - \frac{16g_{126}^{(4)}}{3} - \frac{8g_{129}^{(4)}}{3} - \frac{64g_{136}^{(4)}}{3} - \frac{64g_{139}^{(4)}}{3} - \frac{64g_{140}^{(4)}}{3} - \frac{64g_{147}^{(4)}}{3} \\
&\quad - 4g_{172}^{(4)} + 4g_{173}^{(4)} - 32g_{175}^{(4)} + 32g_{177}^{(4)} - 32g_{178}^{(4)} - \frac{8g_{74}^{(4)}}{9} - \frac{64g_{75}^{(4)}}{9} - \frac{8g_{76}^{(4)}}{3} \\
&\quad + \frac{8g_{78}^{(4)}}{9} - \frac{32g_{80}^{(4)}}{9} - \frac{32g_{81}^{(4)}}{9} + \frac{20\eta_{10}^{(3)}}{27} + \frac{4\eta_{11}^{(3)}}{9} - \frac{2\eta_{180}^{(3)}}{3} + \frac{2\eta_{183}^{(3)}}{3} + \frac{2\eta_{189}^{(3)}}{3} \\
&\quad + \eta_{251}^{(3)} + \frac{\eta_{44}^{(3)}}{3} + \frac{16\eta_{69}^{(3)}}{9} + \frac{32\eta_7^{(3)}}{27} - \frac{4\eta_{70}^{(3)}}{9} + \frac{20\eta_{72}^{(3)}}{9} + \frac{64\eta_8^{(3)}}{27} + \frac{2338}{9} \\
\eta_{259}^{(3)} &= -\frac{2g_{117}^{(4)}}{3} + \frac{4g_{126}^{(4)}}{3} + \frac{16g_{136}^{(4)}}{3} + \frac{16g_{139}^{(4)}}{3} + \frac{16g_{140}^{(4)}}{3} + \frac{16g_{147}^{(4)}}{3} + g_{165}^{(4)} - 2g_{173}^{(4)} + 8g_{175}^{(4)} \\
&\quad - 8g_{177}^{(4)} + 8g_{178}^{(4)} + \frac{4g_{74}^{(4)}}{9} + \frac{16g_{75}^{(4)}}{9} + \frac{4g_{76}^{(4)}}{9} - \frac{4g_{78}^{(4)}}{9} + \frac{8g_{80}^{(4)}}{9} + \frac{8g_{81}^{(4)}}{9} - \frac{2\eta_{10}^{(3)}}{27} - \frac{2\eta_{11}^{(3)}}{9} \\
&\quad + \frac{\eta_{180}^{(3)}}{3} - \frac{\eta_{182}^{(3)}}{3} + \frac{\eta_{189}^{(3)}}{3} + \eta_{253}^{(3)} + \frac{\eta_{44}^{(3)}}{6} - \frac{4\eta_{69}^{(3)}}{9} - \frac{8\eta_7^{(3)}}{27} + \frac{2\eta_{70}^{(3)}}{9} - \frac{2\eta_{72}^{(3)}}{9} - \frac{16\eta_8^{(3)}}{27} - \frac{584}{9}
\end{aligned}$$

$$\begin{aligned}
\eta_{260}^{(3)} = & -\frac{4g_{117}^{(4)}}{3} - \frac{2g_{129}^{(4)}}{3} + \frac{4g_{130}^{(4)}}{3} - \frac{4g_{134}^{(4)}}{3} - \frac{4g_{135}^{(4)}}{3} - 4g_{136}^{(4)} - \frac{8g_{137}^{(4)}}{3} - \frac{16g_{139}^{(4)}}{3} - \frac{8g_{140}^{(4)}}{3} \\
& - \frac{16g_{142}^{(4)}}{3} - 4g_{144}^{(4)} + \frac{8g_{145}^{(4)}}{3} + \frac{4g_{146}^{(4)}}{3} - \frac{16g_{147}^{(4)}}{3} - \frac{8g_{148}^{(4)}}{3} - 8g_{176}^{(4)} - 4g_{177}^{(4)} + 4g_{179}^{(4)} - 8g_{180}^{(4)} \\
& - 32g_{185}^{(4)} - 16g_{187}^{(4)} + 16g_{188}^{(4)} - 8g_{191}^{(4)} - 8g_{192}^{(4)} + 8g_{193}^{(4)} - \frac{g_{69}^{(4)}}{54} - \frac{4g_{74}^{(4)}}{9} - \frac{8g_{75}^{(4)}}{9} - \frac{4g_{76}^{(4)}}{9} \\
& + \frac{4g_{78}^{(4)}}{9} - \frac{4g_{80}^{(4)}}{9} - \frac{2g_{81}^{(4)}}{3} + \frac{2\eta_{10}^{(3)}}{27} + \frac{2\eta_{11}^{(3)}}{9} - \frac{2\eta_{202}^{(3)}}{3} + \frac{\eta_{44}^{(3)}}{6} - \frac{\eta_{60}^{(3)}}{3} - \frac{\eta_{61}^{(3)}}{9} - \frac{\eta_{68}^{(3)}}{9} + \frac{\eta_{69}^{(3)}}{9} \\
& + \frac{2\eta_7^{(3)}}{9} + \frac{\eta_{70}^{(3)}}{9} - \frac{\eta_{71}^{(3)}}{3} + \frac{\eta_{72}^{(3)}}{9} + \frac{\eta_{73}^{(3)}}{9} - \frac{\eta_{74}^{(3)}}{9} + \frac{8\eta_8^{(3)}}{27} + \frac{2\eta_{83}^{(3)}}{3} + \frac{2\eta_{84}^{(3)}}{3} - \frac{2\eta_{85}^{(3)}}{3} + \frac{863}{18} \\
\eta_{261}^{(3)} = & -2g_{136}^{(4)} - \frac{4g_{137}^{(4)}}{3} + \frac{2g_{138}^{(4)}}{3} - \frac{10g_{139}^{(4)}}{3} - \frac{2g_{141}^{(4)}}{3} - \frac{8g_{142}^{(4)}}{3} - \frac{4g_{144}^{(4)}}{3} + \frac{2g_{145}^{(4)}}{3} + \frac{2g_{146}^{(4)}}{3} - \frac{4g_{147}^{(4)}}{3} \\
& - \frac{4g_{148}^{(4)}}{3} - g_{176}^{(4)} - g_{180}^{(4)} - 16g_{185}^{(4)} - 8g_{186}^{(4)} - 4g_{187}^{(4)} - \frac{2g_{74}^{(4)}}{9} - \frac{4g_{75}^{(4)}}{9} - \frac{2g_{76}^{(4)}}{9} + \frac{4g_{78}^{(4)}}{9} - \frac{g_{80}^{(4)}}{9} \\
& - \frac{g_{81}^{(4)}}{3} + \frac{\eta_{11}^{(3)}}{9} - \frac{2\eta_{204}^{(3)}}{3} - \frac{\eta_{60}^{(3)}}{9} - \frac{\eta_{61}^{(3)}}{9} + \frac{\eta_7^{(3)}}{9} + \frac{\eta_8^{(3)}}{9} - \frac{\eta_{80}^{(3)}}{9} + \frac{2\eta_{84}^{(3)}}{9} - \frac{2\eta_{85}^{(3)}}{9} + \frac{139}{8} \\
\eta_{262}^{(3)} = & -\frac{g_{131}^{(4)}}{3} - g_{174}^{(4)} - \frac{\eta_{194}^{(3)}}{3} + \frac{1}{12} \\
\eta_{263}^{(3)} = & -\frac{5g_{117}^{(4)}}{3} + \frac{2g_{126}^{(4)}}{3} + 4g_{136}^{(4)} + \frac{8g_{137}^{(4)}}{3} - \frac{8g_{138}^{(4)}}{3} + \frac{16g_{139}^{(4)}}{3} + \frac{8g_{141}^{(4)}}{3} + \frac{16g_{142}^{(4)}}{3} \\
& + \frac{8g_{147}^{(4)}}{3} + \frac{8g_{148}^{(4)}}{3} + 2g_{165}^{(4)} - g_{173}^{(4)} + 4g_{175}^{(4)} + 4g_{176}^{(4)} - 4g_{177}^{(4)} + 4g_{178}^{(4)} + 4g_{180}^{(4)} \\
& + \frac{g_{69}^{(4)}}{54} + \frac{4g_{74}^{(4)}}{9} + \frac{8g_{75}^{(4)}}{9} + \frac{4g_{80}^{(4)}}{9} + \frac{2g_{81}^{(4)}}{3} - \frac{2\eta_{11}^{(3)}}{9} - \frac{\eta_{178}^{(3)}}{6} + \frac{\eta_{179}^{(3)}}{6} + \frac{\eta_{181}^{(3)}}{6} \\
& - \frac{\eta_{183}^{(3)}}{6} + \frac{\eta_{189}^{(3)}}{6} + \frac{\eta_{44}^{(3)}}{4} - \frac{\eta_{68}^{(3)}}{9} - \frac{\eta_{69}^{(3)}}{9} - \frac{2\eta_7^{(3)}}{9} - \frac{8\eta_8^{(3)}}{27} + \frac{4\eta_{80}^{(3)}}{9} + \frac{4\eta_{83}^{(3)}}{9} - \frac{407}{9} \\
\eta_{265}^{(3)} = & -\frac{4g_{117}^{(4)}}{3} - \frac{2g_{126}^{(4)}}{3} - \frac{2g_{129}^{(4)}}{3} - \frac{8g_{136}^{(4)}}{3} - \frac{8g_{139}^{(4)}}{3} - \frac{8g_{140}^{(4)}}{3} - \frac{8g_{147}^{(4)}}{3} + g_{165}^{(4)} \\
& - g_{172}^{(4)} - 4g_{175}^{(4)} + 4g_{177}^{(4)} - 4g_{178}^{(4)} - \frac{8g_{75}^{(4)}}{9} - \frac{4g_{76}^{(4)}}{9} - \frac{4g_{80}^{(4)}}{9} - \frac{4g_{81}^{(4)}}{9} + \frac{4\eta_{10}^{(3)}}{27} \\
& - \frac{2\eta_{185}^{(3)}}{3} + \frac{\eta_{189}^{(3)}}{3} - \eta_{264}^{(3)} + \frac{\eta_{44}^{(3)}}{6} + \frac{2\eta_{69}^{(3)}}{9} + \frac{4\eta_7^{(3)}}{27} + \frac{4\eta_{72}^{(3)}}{9} + \frac{8\eta_8^{(3)}}{27} + \frac{199}{6} \\
\eta_{266}^{(3)} = & \frac{2g_{117}^{(4)}}{3} + \frac{g_{120}^{(4)}}{3} - \frac{g_{122}^{(4)}}{3} - \frac{g_{131}^{(4)}}{3} - \frac{2g_{135}^{(4)}}{3} - \frac{2g_{137}^{(4)}}{3} - \frac{4g_{142}^{(4)}}{3} - \frac{2g_{144}^{(4)}}{3} + \frac{2g_{145}^{(4)}}{3} - \frac{2g_{147}^{(4)}}{3} \\
& - \frac{2g_{148}^{(4)}}{3} + 2g_{169}^{(4)} - g_{176}^{(4)} - g_{180}^{(4)} - 2g_{184}^{(4)} - 4g_{190}^{(4)} - 4g_{191}^{(4)} - \frac{g_{74}^{(4)}}{9} - \frac{2g_{76}^{(4)}}{9} + \frac{g_{78}^{(4)}}{3} \\
& + \frac{\eta_{10}^{(3)}}{54} + \frac{\eta_{11}^{(3)}}{18} - \frac{2\eta_{205}^{(3)}}{3} - \frac{\eta_{44}^{(3)}}{9} - \frac{\eta_{60}^{(3)}}{18} + \frac{\eta_{61}^{(3)}}{18} - \frac{2\eta_{77}^{(3)}}{9} + \frac{\eta_{83}^{(3)}}{9} + \frac{\eta_{84}^{(3)}}{9} - \frac{\eta_{85}^{(3)}}{9} + \frac{17}{8} \\
\eta_{267}^{(3)} = & -\frac{2g_{131}^{(4)}}{3} + \frac{2g_{134}^{(4)}}{3} - \frac{2g_{135}^{(4)}}{3} - g_{165}^{(4)} - 2g_{174}^{(4)} - \frac{g_{74}^{(4)}}{9} + \frac{g_{78}^{(4)}}{9} - \frac{\eta_{10}^{(3)}}{54} + \frac{\eta_{11}^{(3)}}{18} \\
& + \frac{\eta_{183}^{(3)}}{6} - \frac{\eta_{187}^{(3)}}{3} - \frac{\eta_{188}^{(3)}}{3} - \frac{\eta_{189}^{(3)}}{6} + \frac{\eta_{44}^{(3)}}{36} + \frac{\eta_{70}^{(3)}}{9} - \frac{\eta_{72}^{(3)}}{9} - \frac{4\eta_{77}^{(3)}}{9} + \frac{1}{18}
\end{aligned}$$

$$\begin{aligned}
\eta_{268}^{(3)} &= -\frac{11g_{117}^{(4)}}{12} - \frac{g_{126}^{(4)}}{3} - \frac{g_{129}^{(4)}}{3} + \frac{g_{130}^{(4)}}{3} + \frac{2g_{131}^{(4)}}{3} - \frac{g_{134}^{(4)}}{3} + \frac{g_{135}^{(4)}}{3} - \frac{4g_{136}^{(4)}}{3} - \frac{4g_{139}^{(4)}}{3} \\
&\quad - \frac{4g_{140}^{(4)}}{3} - \frac{4g_{147}^{(4)}}{3} + \frac{g_{165}^{(4)}}{4} - \frac{g_{172}^{(4)}}{2} + \frac{g_{173}^{(4)}}{2} + 2g_{174}^{(4)} - 2g_{175}^{(4)} + 2g_{177}^{(4)} - 2g_{178}^{(4)} + \frac{g_{74}^{(4)}}{18} \\
&\quad - \frac{4g_{75}^{(4)}}{9} - \frac{5g_{78}^{(4)}}{18} - \frac{2g_{80}^{(4)}}{9} - \frac{2g_{81}^{(4)}}{9} + \frac{5\eta_{10}^{(3)}}{108} - \frac{\eta_{11}^{(3)}}{36} - \frac{\eta_{180}^{(3)}}{12} + \frac{\eta_{182}^{(3)}}{12} + \frac{\eta_{189}^{(3)}}{12} + \frac{\eta_{44}^{(3)}}{8} \\
&\quad + \frac{\eta_{69}^{(3)}}{9} + \frac{2\eta_7^{(3)}}{27} - \frac{\eta_{70}^{(3)}}{18} - \frac{\eta_{71}^{(3)}}{18} + \frac{\eta_{72}^{(3)}}{6} + \frac{\eta_{73}^{(3)}}{18} - \frac{\eta_{74}^{(3)}}{18} + \frac{2\eta_{77}^{(3)}}{9} + \frac{4\eta_8^{(3)}}{27} + \frac{185}{12} \\
\eta_{269}^{(3)} &= -\frac{2g_{117}^{(4)}}{3} - \frac{g_{126}^{(4)}}{3} - \frac{g_{129}^{(4)}}{3} - \frac{4g_{136}^{(4)}}{3} - \frac{4g_{139}^{(4)}}{3} - \frac{4g_{140}^{(4)}}{3} - \frac{4g_{147}^{(4)}}{3} \\
&\quad + g_{165}^{(4)} - 2g_{175}^{(4)} - 2g_{178}^{(4)} - \frac{4g_{75}^{(4)}}{9} - \frac{2g_{76}^{(4)}}{9} - \frac{2g_{80}^{(4)}}{9} - \frac{2g_{81}^{(4)}}{9} + \frac{2\eta_{10}^{(3)}}{27} \\
&\quad - \frac{\eta_{178}^{(3)}}{6} + \frac{\eta_{189}^{(3)}}{6} + \frac{\eta_{44}^{(3)}}{12} + \frac{\eta_{69}^{(3)}}{9} + \frac{2\eta_7^{(3)}}{27} + \frac{2\eta_{72}^{(3)}}{9} + \frac{4\eta_8^{(3)}}{27} + \frac{95}{6} \\
\eta_{270}^{(3)} &= -\frac{g_{131}^{(4)}}{3} - 2g_{184}^{(4)} - \frac{\eta_{193}^{(3)}}{6} - \frac{1}{2} \\
\eta_{271}^{(3)} &= -\frac{g_{117}^{(4)}}{3} - \frac{g_{129}^{(4)}}{6} + \frac{g_{130}^{(4)}}{3} - \frac{g_{134}^{(4)}}{3} - \frac{g_{135}^{(4)}}{3} - g_{136}^{(4)} - \frac{2g_{137}^{(4)}}{3} - \frac{4g_{139}^{(4)}}{3} - \frac{2g_{140}^{(4)}}{3} - \frac{4g_{142}^{(4)}}{3} \\
&\quad - g_{144}^{(4)} + \frac{2g_{145}^{(4)}}{3} + \frac{g_{146}^{(4)}}{3} - \frac{4g_{147}^{(4)}}{3} - \frac{2g_{148}^{(4)}}{3} - g_{176}^{(4)} - g_{177}^{(4)} + g_{179}^{(4)} - g_{180}^{(4)} - 8g_{185}^{(4)} \\
&\quad - 4g_{186}^{(4)} - 4g_{187}^{(4)} - 2g_{191}^{(4)} - 2g_{192}^{(4)} + 2g_{193}^{(4)} - \frac{g_{69}^{(4)}}{216} - \frac{g_{74}^{(4)}}{9} - \frac{2g_{75}^{(4)}}{9} - \frac{g_{76}^{(4)}}{9} + \frac{g_{78}^{(4)}}{9} \\
&\quad - \frac{g_{80}^{(4)}}{9} - \frac{g_{81}^{(4)}}{6} + \frac{\eta_{10}^{(3)}}{54} + \frac{\eta_{11}^{(3)}}{18} - \frac{\eta_{202}^{(3)}}{6} + \frac{\eta_{44}^{(3)}}{24} - \frac{\eta_{60}^{(3)}}{12} - \frac{\eta_{61}^{(3)}}{36} - \frac{\eta_{68}^{(3)}}{36} + \frac{\eta_{69}^{(3)}}{36} + \frac{\eta_7^{(3)}}{18} \\
&\quad + \frac{\eta_{70}^{(3)}}{36} - \frac{\eta_{71}^{(3)}}{12} + \frac{\eta_{72}^{(3)}}{36} + \frac{\eta_{73}^{(3)}}{36} - \frac{\eta_{74}^{(3)}}{36} + \frac{2\eta_8^{(3)}}{27} + \frac{\eta_{83}^{(3)}}{6} + \frac{\eta_{84}^{(3)}}{6} - \frac{\eta_{85}^{(3)}}{6} + \frac{209}{18} \\
\eta_{272}^{(3)} &= \frac{3g_{117}^{(4)}}{2} - \frac{g_{126}^{(4)}}{3} + \frac{g_{129}^{(4)}}{3} - \frac{2g_{130}^{(4)}}{3} + 4g_{136}^{(4)} + 4g_{139}^{(4)} + 4g_{140}^{(4)} + \frac{8g_{144}^{(4)}}{3} - \frac{8g_{146}^{(4)}}{3} + 4g_{147}^{(4)} \\
&\quad + 2g_{165}^{(4)} - 2g_{175}^{(4)} + 4g_{177}^{(4)} - 2g_{178}^{(4)} + 32g_{185}^{(4)} + 16g_{187}^{(4)} - 16g_{188}^{(4)} + \frac{2g_{69}^{(4)}}{27} + \frac{4g_{74}^{(4)}}{9} + \frac{4g_{75}^{(4)}}{9} \\
&\quad + \frac{2g_{76}^{(4)}}{9} - \frac{4g_{78}^{(4)}}{9} + \frac{2g_{80}^{(4)}}{3} + \frac{2g_{81}^{(4)}}{3} - \frac{2\eta_{11}^{(3)}}{9} - \frac{\eta_{178}^{(3)}}{6} + \frac{\eta_{179}^{(3)}}{6} - \frac{\eta_{183}^{(3)}}{6} + \frac{\eta_{189}^{(3)}}{6} - \frac{7\eta_{44}^{(3)}}{36} + \frac{2\eta_{60}^{(3)}}{9} \\
&\quad + \frac{2\eta_{61}^{(3)}}{9} + \frac{2\eta_{68}^{(3)}}{9} - \frac{\eta_{69}^{(3)}}{9} - \frac{2\eta_7^{(3)}}{9} - \frac{2\eta_{70}^{(3)}}{9} + \frac{2\eta_{71}^{(3)}}{9} - \frac{8\eta_8^{(3)}}{27} - \frac{4\eta_{83}^{(3)}}{9} - \frac{4\eta_{84}^{(3)}}{9} + \frac{4\eta_{85}^{(3)}}{9} - \frac{128}{3} \\
\eta_{273}^{(3)} &= -\frac{2g_{117}^{(4)}}{3} - \frac{g_{126}^{(4)}}{3} - \frac{g_{129}^{(4)}}{3} - \frac{4g_{136}^{(4)}}{3} - \frac{4g_{139}^{(4)}}{3} - \frac{4g_{140}^{(4)}}{3} - \frac{4g_{147}^{(4)}}{3} \\
&\quad + \frac{g_{165}^{(4)}}{2} - 2g_{175}^{(4)} - 2g_{178}^{(4)} - \frac{4g_{75}^{(4)}}{9} - \frac{2g_{76}^{(4)}}{9} - \frac{2g_{80}^{(4)}}{9} - \frac{2g_{81}^{(4)}}{9} + \frac{2\eta_{10}^{(3)}}{27} \\
&\quad - \frac{\eta_{182}^{(3)}}{6} + \frac{\eta_{189}^{(3)}}{6} + \frac{\eta_{44}^{(3)}}{12} + \frac{\eta_{69}^{(3)}}{9} + \frac{2\eta_7^{(3)}}{27} + \frac{2\eta_{72}^{(3)}}{9} + \frac{4\eta_8^{(3)}}{27} + \frac{97}{6}
\end{aligned}$$

$$\begin{aligned}
\eta_{274}^{(3)} &= -\frac{2g_{117}^{(4)}}{3} - \frac{g_{126}^{(4)}}{3} - \frac{g_{129}^{(4)}}{3} - \frac{4g_{136}^{(4)}}{3} - \frac{4g_{139}^{(4)}}{3} - \frac{4g_{140}^{(4)}}{3} - \frac{4g_{147}^{(4)}}{3} \\
&\quad - 2g_{175}^{(4)} - 2g_{178}^{(4)} - \frac{4g_{75}^{(4)}}{9} - \frac{2g_{76}^{(4)}}{9} - \frac{2g_{80}^{(4)}}{9} - \frac{2g_{81}^{(4)}}{9} + \frac{2\eta_{10}^{(3)}}{27} \\
&\quad - \frac{\eta_{179}^{(3)}}{6} + \frac{\eta_{189}^{(3)}}{6} + \frac{\eta_{44}^{(3)}}{12} + \frac{\eta_{69}^{(3)}}{9} + \frac{2\eta_7^{(3)}}{27} + \frac{2\eta_{72}^{(3)}}{9} + \frac{4\eta_8^{(3)}}{27} + \frac{95}{6} \\
\eta_{275}^{(3)} &= g_{117}^{(4)} - g_{126}^{(4)} + \frac{g_{129}^{(4)}}{3} - \frac{4g_{130}^{(4)}}{3} + \frac{4g_{134}^{(4)}}{3} + \frac{4g_{135}^{(4)}}{3} - \frac{8g_{136}^{(4)}}{3} - 4g_{139}^{(4)} - \frac{4g_{140}^{(4)}}{3} + \frac{4g_{144}^{(4)}}{3} \\
&\quad - \frac{4g_{146}^{(4)}}{3} - \frac{4g_{147}^{(4)}}{3} + 2g_{165}^{(4)} - 6g_{175}^{(4)} + 8g_{177}^{(4)} - 6g_{178}^{(4)} + 8g_{191}^{(4)} + 8g_{192}^{(4)} - 8g_{193}^{(4)} \\
&\quad + \frac{g_{69}^{(4)}}{18} - \frac{4g_{75}^{(4)}}{3} - \frac{2g_{76}^{(4)}}{3} + \frac{8g_{78}^{(4)}}{9} - \frac{2g_{80}^{(4)}}{9} - \frac{4g_{81}^{(4)}}{9} + \frac{2\eta_{10}^{(3)}}{27} - \frac{\eta_{178}^{(3)}}{6} + \frac{\eta_{179}^{(3)}}{6} \\
&\quad - \frac{\eta_{180}^{(3)}}{6} + \frac{\eta_{181}^{(3)}}{6} - \frac{\eta_{183}^{(3)}}{6} + \frac{\eta_{189}^{(3)}}{6} - \frac{7\eta_{44}^{(3)}}{36} + \frac{\eta_{60}^{(3)}}{9} - \frac{\eta_{61}^{(3)}}{9} + \frac{\eta_{68}^{(3)}}{9} + \frac{2\eta_{69}^{(3)}}{9} + \frac{4\eta_7^{(3)}}{27} \\
&\quad - \frac{\eta_{70}^{(3)}}{3} + \frac{\eta_{71}^{(3)}}{3} + \frac{\eta_{72}^{(3)}}{3} - \frac{\eta_{73}^{(3)}}{9} + \frac{\eta_{74}^{(3)}}{9} + \frac{8\eta_8^{(3)}}{27} - \frac{2\eta_{83}^{(3)}}{9} - \frac{2\eta_{84}^{(3)}}{9} + \frac{2\eta_{85}^{(3)}}{9} + \frac{497}{18} \\
\eta_{276}^{(3)} &= -\frac{g_{129}^{(4)}}{3} + \frac{2g_{130}^{(4)}}{3} - \frac{4g_{134}^{(4)}}{3} - \frac{4g_{135}^{(4)}}{3} - \frac{4g_{144}^{(4)}}{3} + \frac{4g_{146}^{(4)}}{3} - \frac{4g_{147}^{(4)}}{3} + g_{165}^{(4)} - 4g_{177}^{(4)} \\
&\quad + 2g_{178}^{(4)} - 8g_{191}^{(4)} - 8g_{192}^{(4)} + 8g_{193}^{(4)} - \frac{2g_{76}^{(4)}}{9} + \frac{2\eta_{10}^{(3)}}{27} - \frac{\eta_{183}^{(3)}}{6} + \frac{\eta_{189}^{(3)}}{6} - \frac{2\eta_{203}^{(3)}}{3} - \frac{\eta_{44}^{(3)}}{36} \\
&\quad - \frac{\eta_{60}^{(3)}}{9} + \frac{\eta_{61}^{(3)}}{9} - \frac{\eta_{70}^{(3)}}{9} - \frac{\eta_{71}^{(3)}}{9} + \frac{\eta_{72}^{(3)}}{9} + \frac{\eta_{73}^{(3)}}{9} - \frac{\eta_{74}^{(3)}}{9} + \frac{2\eta_{83}^{(3)}}{9} + \frac{2\eta_{84}^{(3)}}{9} - \frac{2\eta_{85}^{(3)}}{9} - \frac{4}{3} \\
\eta_{278}^{(3)} &= -\frac{g_{117}^{(4)}}{6} - \frac{g_{126}^{(4)}}{12} - \frac{g_{130}^{(4)}}{6} + \frac{g_{134}^{(4)}}{3} + \frac{g_{135}^{(4)}}{3} - \frac{g_{136}^{(4)}}{3} - \frac{g_{139}^{(4)}}{3} - \frac{g_{140}^{(4)}}{3} + \frac{g_{144}^{(4)}}{3} - \frac{g_{146}^{(4)}}{3} - \frac{g_{175}^{(4)}}{2} + g_{177}^{(4)} \\
&\quad - g_{178}^{(4)} + 2g_{191}^{(4)} + 2g_{192}^{(4)} - 2g_{193}^{(4)} - \frac{g_{75}^{(4)}}{9} - \frac{g_{80}^{(4)}}{18} - \frac{g_{81}^{(4)}}{18} - \frac{\eta_{185}^{(3)}}{6} + \frac{\eta_{203}^{(3)}}{6} + \frac{\eta_{44}^{(3)}}{36} + \frac{\eta_{60}^{(3)}}{36} - \frac{\eta_{61}^{(3)}}{36} \\
&\quad + \frac{\eta_{69}^{(3)}}{36} + \frac{\eta_7^{(3)}}{54} + \frac{\eta_{70}^{(3)}}{36} + \frac{\eta_{71}^{(3)}}{36} + \frac{\eta_{72}^{(3)}}{36} - \frac{\eta_{73}^{(3)}}{36} + \frac{\eta_{74}^{(3)}}{36} + \frac{\eta_8^{(3)}}{27} - \frac{\eta_{83}^{(3)}}{18} - \frac{\eta_{84}^{(3)}}{18} + \frac{\eta_{85}^{(3)}}{18} + \frac{103}{24} \\
\eta_{279}^{(3)} &= -\frac{g_{131}^{(4)}}{6} - g_{184}^{(4)} - \frac{\eta_{194}^{(3)}}{6} - \frac{1}{12} \\
\eta_{280}^{(3)} &= -\frac{g_{136}^{(4)}}{2} - \frac{g_{137}^{(4)}}{3} + \frac{g_{138}^{(4)}}{6} - \frac{5g_{139}^{(4)}}{6} - \frac{g_{141}^{(4)}}{6} - \frac{2g_{142}^{(4)}}{3} - \frac{g_{144}^{(4)}}{3} + \frac{g_{145}^{(4)}}{6} + \frac{g_{146}^{(4)}}{6} - \frac{g_{147}^{(4)}}{3} \\
&\quad - \frac{g_{148}^{(4)}}{3} - 4g_{185}^{(4)} - 3g_{186}^{(4)} - g_{187}^{(4)} - g_{188}^{(4)} - \frac{g_{74}^{(4)}}{18} - \frac{g_{75}^{(4)}}{9} - \frac{g_{76}^{(4)}}{18} + \frac{g_{78}^{(4)}}{9} - \frac{g_{80}^{(4)}}{36} \\
&\quad - \frac{g_{81}^{(4)}}{12} + \frac{\eta_{11}^{(3)}}{36} - \frac{\eta_{204}^{(3)}}{6} - \frac{\eta_{60}^{(3)}}{36} - \frac{\eta_{61}^{(3)}}{36} + \frac{\eta_7^{(3)}}{36} + \frac{\eta_8^{(3)}}{36} - \frac{\eta_{80}^{(3)}}{36} + \frac{\eta_{84}^{(3)}}{18} - \frac{\eta_{85}^{(3)}}{18} + \frac{67}{16} \\
\eta_{281}^{(3)} &= -\frac{29g_{117}^{(4)}}{24} - \frac{g_{129}^{(4)}}{6} + \frac{g_{130}^{(4)}}{6} + \frac{2g_{136}^{(4)}}{3} + \frac{4g_{137}^{(4)}}{3} - \frac{4g_{138}^{(4)}}{3} + \frac{4g_{139}^{(4)}}{3} - \frac{4g_{140}^{(4)}}{3} + \frac{4g_{141}^{(4)}}{3} + \frac{8g_{142}^{(4)}}{3} \\
&\quad + \frac{4g_{148}^{(4)}}{3} + g_{176}^{(4)} - g_{177}^{(4)} + g_{180}^{(4)} + 4g_{186}^{(4)} + 4g_{188}^{(4)} + \frac{g_{69}^{(4)}}{108} + \frac{g_{74}^{(4)}}{9} - \frac{g_{78}^{(4)}}{9} + \frac{g_{81}^{(4)}}{9} + \frac{\eta_{10}^{(3)}}{54} - \frac{\eta_{11}^{(3)}}{18} \\
&\quad - \frac{\eta_{185}^{(3)}}{6} - \eta_{277}^{(3)} + \frac{13\eta_{44}^{(3)}}{72} - \frac{\eta_{68}^{(3)}}{18} + \frac{\eta_{69}^{(3)}}{18} - \frac{\eta_7^{(3)}}{27} + \frac{\eta_{70}^{(3)}}{18} - \frac{\eta_{71}^{(3)}}{18} + \frac{\eta_{72}^{(3)}}{18} + \frac{2\eta_{80}^{(3)}}{9} + \frac{2\eta_{83}^{(3)}}{9} - \frac{50}{9}
\end{aligned}$$



$$\begin{aligned}
\eta_{283}^{(3)} &= \frac{\mathfrak{g}_{117}^{(4)}}{6} + \frac{\mathfrak{g}_{120}^{(4)}}{12} - \frac{\mathfrak{g}_{122}^{(4)}}{12} - \frac{\mathfrak{g}_{131}^{(4)}}{12} - \frac{\mathfrak{g}_{135}^{(4)}}{6} - \frac{\mathfrak{g}_{137}^{(4)}}{6} - \frac{\mathfrak{g}_{142}^{(4)}}{3} - \frac{\mathfrak{g}_{144}^{(4)}}{6} + \frac{\mathfrak{g}_{145}^{(4)}}{6} - \frac{\mathfrak{g}_{147}^{(4)}}{6} \\
&\quad - \frac{\mathfrak{g}_{148}^{(4)}}{6} + \frac{\mathfrak{g}_{169}^{(4)}}{2} - \frac{\mathfrak{g}_{184}^{(4)}}{2} - \mathfrak{g}_{186}^{(4)} - \mathfrak{g}_{188}^{(4)} - \mathfrak{g}_{190}^{(4)} - \mathfrak{g}_{191}^{(4)} - \frac{\mathfrak{g}_{74}^{(4)}}{36} - \frac{\mathfrak{g}_{76}^{(4)}}{18} + \frac{\mathfrak{g}_{78}^{(4)}}{12} \\
&\quad + \frac{\eta_{10}^{(3)}}{216} + \frac{\eta_{11}^{(3)}}{72} - \frac{\eta_{205}^{(3)}}{6} - \frac{\eta_{44}^{(3)}}{36} - \frac{\eta_{60}^{(3)}}{72} + \frac{\eta_{61}^{(3)}}{72} - \frac{\eta_{77}^{(3)}}{18} + \frac{\eta_{83}^{(3)}}{36} + \frac{\eta_{84}^{(3)}}{36} - \frac{\eta_{85}^{(3)}}{36} + \frac{1}{2} \\
\eta_{284}^{(3)} &= -\frac{3\mathfrak{g}_{117}^{(4)}}{4} + \frac{\mathfrak{g}_{126}^{(4)}}{6} - \frac{\mathfrak{g}_{129}^{(4)}}{6} + \frac{\mathfrak{g}_{130}^{(4)}}{3} + \frac{\mathfrak{g}_{131}^{(4)}}{3} + \frac{2\mathfrak{g}_{136}^{(4)}}{3} + \frac{2\mathfrak{g}_{139}^{(4)}}{3} + \frac{2\mathfrak{g}_{140}^{(4)}}{3} + \frac{2\mathfrak{g}_{147}^{(4)}}{3} + \mathfrak{g}_{175}^{(4)} - 2\mathfrak{g}_{177}^{(4)} \\
&\quad + \mathfrak{g}_{178}^{(4)} + 2\mathfrak{g}_{184}^{(4)} + \frac{\mathfrak{g}_{74}^{(4)}}{9} + \frac{2\mathfrak{g}_{75}^{(4)}}{9} + \frac{2\mathfrak{g}_{76}^{(4)}}{9} - \frac{\mathfrak{g}_{78}^{(4)}}{3} + \frac{\mathfrak{g}_{80}^{(4)}}{9} + \frac{\mathfrak{g}_{81}^{(4)}}{9} - \frac{\eta_{10}^{(3)}}{54} - \frac{\eta_{11}^{(3)}}{18} - \frac{\eta_{187}^{(3)}}{6} \\
&\quad - \frac{\eta_{188}^{(3)}}{6} - \eta_{282}^{(3)} + \frac{5\eta_{44}^{(3)}}{36} - \frac{\eta_{69}^{(3)}}{18} - \frac{\eta_7^{(3)}}{27} + \frac{\eta_{70}^{(3)}}{18} - \frac{\eta_{71}^{(3)}}{18} - \frac{\eta_{72}^{(3)}}{18} + \frac{\eta_{73}^{(3)}}{18} - \frac{\eta_{74}^{(3)}}{18} - \frac{2\eta_8^{(3)}}{27} - \frac{277}{36} \\
\eta_{285}^{(3)} &= -\frac{7\mathfrak{g}_{117}^{(4)}}{6} - \frac{2\mathfrak{g}_{126}^{(4)}}{3} - \frac{\mathfrak{g}_{129}^{(4)}}{2} + \frac{\mathfrak{g}_{130}^{(4)}}{3} - \frac{\mathfrak{g}_{134}^{(4)}}{3} - \frac{\mathfrak{g}_{135}^{(4)}}{3} - \frac{8\mathfrak{g}_{136}^{(4)}}{3} - \frac{8\mathfrak{g}_{139}^{(4)}}{3} - \frac{8\mathfrak{g}_{140}^{(4)}}{3} \\
&\quad - \frac{8\mathfrak{g}_{147}^{(4)}}{3} - \frac{\mathfrak{g}_{172}^{(4)}}{2} + \mathfrak{g}_{173}^{(4)} - 4\mathfrak{g}_{175}^{(4)} + 4\mathfrak{g}_{177}^{(4)} - 4\mathfrak{g}_{178}^{(4)} - \mathfrak{g}_{183}^{(4)} - \frac{\mathfrak{g}_{74}^{(4)}}{18} - \frac{8\mathfrak{g}_{75}^{(4)}}{9} \\
&\quad - \frac{2\mathfrak{g}_{76}^{(4)}}{9} - \frac{\mathfrak{g}_{78}^{(4)}}{6} - \frac{4\mathfrak{g}_{80}^{(4)}}{9} - \frac{4\mathfrak{g}_{81}^{(4)}}{9} + \frac{11\eta_{10}^{(3)}}{108} + \frac{\eta_{11}^{(3)}}{36} - \frac{\eta_{180}^{(3)}}{6} + \frac{\eta_{183}^{(3)}}{12} + \frac{\eta_{189}^{(3)}}{12} \\
&\quad + \frac{11\eta_{44}^{(3)}}{72} + \frac{2\eta_{69}^{(3)}}{9} + \frac{4\eta_7^{(3)}}{27} - \frac{\eta_{70}^{(3)}}{18} - \frac{\eta_{71}^{(3)}}{18} + \frac{5\eta_{72}^{(3)}}{18} + \frac{\eta_{73}^{(3)}}{18} - \frac{\eta_{74}^{(3)}}{18} + \frac{8\eta_8^{(3)}}{27} + \frac{94}{3} \\
\eta_{286}^{(3)} &= -\frac{\mathfrak{g}_{117}^{(4)}}{3} - \frac{\mathfrak{g}_{129}^{(4)}}{6} + \frac{\mathfrak{g}_{130}^{(4)}}{3} - \frac{\mathfrak{g}_{134}^{(4)}}{3} - \frac{\mathfrak{g}_{135}^{(4)}}{3} - \mathfrak{g}_{136}^{(4)} - \frac{2\mathfrak{g}_{137}^{(4)}}{3} - \frac{4\mathfrak{g}_{139}^{(4)}}{3} - \frac{2\mathfrak{g}_{140}^{(4)}}{3} - \frac{4\mathfrak{g}_{142}^{(4)}}{3} \\
&\quad - \mathfrak{g}_{144}^{(4)} + \frac{2\mathfrak{g}_{145}^{(4)}}{3} + \frac{\mathfrak{g}_{146}^{(4)}}{3} - \frac{4\mathfrak{g}_{147}^{(4)}}{3} - \frac{2\mathfrak{g}_{148}^{(4)}}{3} - \mathfrak{g}_{176}^{(4)} - \mathfrak{g}_{177}^{(4)} + \mathfrak{g}_{179}^{(4)} - \mathfrak{g}_{180}^{(4)} - 8\mathfrak{g}_{185}^{(4)} \\
&\quad - 4\mathfrak{g}_{187}^{(4)} + 4\mathfrak{g}_{188}^{(4)} - 4\mathfrak{g}_{190}^{(4)} - 2\mathfrak{g}_{191}^{(4)} - 2\mathfrak{g}_{192}^{(4)} - 2\mathfrak{g}_{193}^{(4)} - \frac{\mathfrak{g}_{69}^{(4)}}{216} - \frac{\mathfrak{g}_{74}^{(4)}}{9} - \frac{2\mathfrak{g}_{75}^{(4)}}{9} - \frac{\mathfrak{g}_{76}^{(4)}}{9} \\
&\quad + \frac{\mathfrak{g}_{78}^{(4)}}{9} - \frac{\mathfrak{g}_{80}^{(4)}}{9} - \frac{\mathfrak{g}_{81}^{(4)}}{6} + \frac{\eta_{10}^{(3)}}{54} + \frac{\eta_{11}^{(3)}}{18} - \frac{\eta_{202}^{(3)}}{6} + \frac{\eta_{44}^{(3)}}{24} - \frac{\eta_{60}^{(3)}}{12} - \frac{\eta_{61}^{(3)}}{36} - \frac{\eta_{68}^{(3)}}{36} + \frac{\eta_{69}^{(3)}}{36} \\
&\quad + \frac{\eta_7^{(3)}}{18} + \frac{\eta_{70}^{(3)}}{36} - \frac{\eta_{71}^{(3)}}{12} + \frac{\eta_{72}^{(3)}}{36} + \frac{\eta_{73}^{(3)}}{36} - \frac{\eta_{74}^{(3)}}{36} + \frac{2\eta_8^{(3)}}{27} + \frac{\eta_{83}^{(3)}}{6} + \frac{\eta_{84}^{(3)}}{6} - \frac{\eta_{85}^{(3)}}{6} + \frac{391}{36} \\
\eta_{287}^{(3)} &= 2\mathfrak{g}_{117}^{(4)} - 2\mathfrak{g}_{126}^{(4)} + \frac{\mathfrak{g}_{129}^{(4)}}{3} - 2\mathfrak{g}_{130}^{(4)} + 2\mathfrak{g}_{134}^{(4)} + 2\mathfrak{g}_{135}^{(4)} - \frac{20\mathfrak{g}_{136}^{(4)}}{3} - 8\mathfrak{g}_{139}^{(4)} - \frac{16\mathfrak{g}_{140}^{(4)}}{3} + \frac{4\mathfrak{g}_{144}^{(4)}}{3} \\
&\quad - \frac{4\mathfrak{g}_{146}^{(4)}}{3} - \frac{16\mathfrak{g}_{147}^{(4)}}{3} + \frac{3\mathfrak{g}_{165}^{(4)}}{2} - 12\mathfrak{g}_{175}^{(4)} + 12\mathfrak{g}_{177}^{(4)} - 12\mathfrak{g}_{178}^{(4)} + 2\mathfrak{g}_{183}^{(4)} + 8\mathfrak{g}_{191}^{(4)} + 8\mathfrak{g}_{192}^{(4)} \\
&\quad - 8\mathfrak{g}_{193}^{(4)} + \frac{\mathfrak{g}_{69}^{(4)}}{18} - \frac{\mathfrak{g}_{74}^{(4)}}{3} - \frac{8\mathfrak{g}_{75}^{(4)}}{3} - \frac{4\mathfrak{g}_{76}^{(4)}}{3} + \frac{5\mathfrak{g}_{78}^{(4)}}{3} - \frac{8\mathfrak{g}_{80}^{(4)}}{9} - \frac{10\mathfrak{g}_{81}^{(4)}}{9} + \frac{\eta_{10}^{(3)}}{6} + \frac{\eta_{11}^{(3)}}{6} - \frac{\eta_{178}^{(3)}}{6} \\
&\quad - \frac{\eta_{180}^{(3)}}{6} + \frac{\eta_{181}^{(3)}}{6} + \frac{\eta_{182}^{(3)}}{6} - \frac{\eta_{183}^{(3)}}{6} + \frac{\eta_{189}^{(3)}}{6} - \frac{5\eta_{44}^{(3)}}{12} + \frac{\eta_{60}^{(3)}}{9} - \frac{\eta_{61}^{(3)}}{9} + \frac{\eta_{68}^{(3)}}{9} + \frac{5\eta_{69}^{(3)}}{9} + \frac{10\eta_7^{(3)}}{27} \\
&\quad - \frac{4\eta_{70}^{(3)}}{9} + \frac{4\eta_{71}^{(3)}}{9} + \frac{2\eta_{72}^{(3)}}{3} - \frac{2\eta_{73}^{(3)}}{9} + \frac{2\eta_{74}^{(3)}}{9} + \frac{20\eta_8^{(3)}}{27} - \frac{2\eta_{83}^{(3)}}{9} - \frac{2\eta_{84}^{(3)}}{9} + \frac{2\eta_{85}^{(3)}}{9} + \frac{481}{6}
\end{aligned}$$

$$\begin{aligned}
\eta_{288}^{(3)} &= -\frac{11g_{117}^{(4)}}{6} - \frac{g_{129}^{(4)}}{3} + \frac{4g_{130}^{(4)}}{3} - \frac{2g_{134}^{(4)}}{3} - \frac{2g_{135}^{(4)}}{3} - 4g_{165}^{(4)} + 2g_{173}^{(4)} - 2g_{183}^{(4)} \\
&\quad - \frac{g_{74}^{(4)}}{9} + \frac{8g_{76}^{(4)}}{9} - \frac{11g_{78}^{(4)}}{9} - \frac{5\eta_{10}^{(3)}}{54} + \frac{\eta_{11}^{(3)}}{18} + \frac{\eta_{178}^{(3)}}{6} - \frac{\eta_{179}^{(3)}}{6} - \frac{\eta_{181}^{(3)}}{3} \\
&\quad + \frac{\eta_{183}^{(3)}}{2} - \frac{\eta_{189}^{(3)}}{2} + \frac{13\eta_{44}^{(3)}}{36} + \frac{\eta_{70}^{(3)}}{3} - \frac{\eta_{71}^{(3)}}{3} - \frac{\eta_{72}^{(3)}}{3} + \frac{\eta_{73}^{(3)}}{9} - \frac{\eta_{74}^{(3)}}{9} - 3 \\
\eta_{289}^{(3)} &= -\frac{g_{117}^{(4)}}{3} + \frac{4g_{126}^{(4)}}{3} + \frac{g_{129}^{(4)}}{6} + g_{130}^{(4)} - g_{134}^{(4)} - g_{135}^{(4)} + \frac{14g_{136}^{(4)}}{3} + \frac{16g_{139}^{(4)}}{3} + 4g_{140}^{(4)} - \frac{2g_{144}^{(4)}}{3} \\
&\quad + \frac{2g_{146}^{(4)}}{3} + 4g_{147}^{(4)} - g_{165}^{(4)} + \frac{g_{172}^{(4)}}{2} + 8g_{175}^{(4)} - 8g_{177}^{(4)} + 8g_{178}^{(4)} - g_{183}^{(4)} - 4g_{191}^{(4)} - 4g_{192}^{(4)} \\
&\quad + 4g_{193}^{(4)} - \frac{g_{69}^{(4)}}{36} + \frac{g_{74}^{(4)}}{6} + \frac{16g_{75}^{(4)}}{9} + \frac{8g_{76}^{(4)}}{9} - \frac{5g_{78}^{(4)}}{6} + \frac{2g_{80}^{(4)}}{3} + \frac{7g_{81}^{(4)}}{9} - \frac{17\eta_{10}^{(3)}}{108} \\
&\quad - \frac{\eta_{11}^{(3)}}{12} + \frac{\eta_{183}^{(3)}}{12} - \frac{\eta_{189}^{(3)}}{4} - \frac{\eta_{218}^{(3)}}{3} + \frac{\eta_{44}^{(3)}}{8} - \frac{\eta_{60}^{(3)}}{18} + \frac{\eta_{61}^{(3)}}{18} - \frac{\eta_{68}^{(3)}}{18} - \frac{7\eta_{69}^{(3)}}{18} - \frac{7\eta_7^{(3)}}{27} \\
&\quad + \frac{2\eta_{70}^{(3)}}{9} - \frac{2\eta_{71}^{(3)}}{9} - \frac{5\eta_{72}^{(3)}}{9} + \frac{\eta_{73}^{(3)}}{9} - \frac{\eta_{74}^{(3)}}{9} - \frac{14\eta_8^{(3)}}{27} + \frac{\eta_{83}^{(3)}}{9} + \frac{\eta_{84}^{(3)}}{9} - \frac{\eta_{85}^{(3)}}{9} - \frac{172}{3} \\
\eta_{291}^{(3)} &= -\frac{g_{136}^{(4)}}{2} - \frac{g_{137}^{(4)}}{3} + \frac{g_{138}^{(4)}}{6} - \frac{5g_{139}^{(4)}}{6} - \frac{g_{141}^{(4)}}{6} - \frac{2g_{142}^{(4)}}{3} - \frac{g_{144}^{(4)}}{3} + \frac{g_{145}^{(4)}}{6} + \frac{g_{146}^{(4)}}{6} - \frac{g_{147}^{(4)}}{3} \\
&\quad - \frac{g_{148}^{(4)}}{3} - 4g_{185}^{(4)} - 2g_{186}^{(4)} - g_{187}^{(4)} - g_{190}^{(4)} - g_{193}^{(4)} - \frac{g_{74}^{(4)}}{18} - \frac{g_{75}^{(4)}}{9} - \frac{g_{76}^{(4)}}{18} + \frac{g_{78}^{(4)}}{9} - \frac{g_{80}^{(4)}}{36} \\
&\quad - \frac{g_{81}^{(4)}}{12} + \frac{\eta_{11}^{(3)}}{36} - \frac{\eta_{204}^{(3)}}{6} - \frac{\eta_{60}^{(3)}}{36} - \frac{\eta_{61}^{(3)}}{36} + \frac{\eta_7^{(3)}}{36} + \frac{\eta_8^{(3)}}{36} - \frac{\eta_{80}^{(3)}}{36} + \frac{\eta_{84}^{(3)}}{18} - \frac{\eta_{85}^{(3)}}{18} + \frac{31}{8} \\
\eta_{292}^{(3)} &= -\frac{41g_{117}^{(4)}}{24} + \frac{g_{126}^{(4)}}{2} - \frac{g_{129}^{(4)}}{6} + \frac{g_{130}^{(4)}}{2} - \frac{g_{134}^{(4)}}{3} - \frac{g_{135}^{(4)}}{3} + \frac{8g_{136}^{(4)}}{3} + \frac{4g_{137}^{(4)}}{3} - \frac{4g_{138}^{(4)}}{3} \\
&\quad + \frac{10g_{139}^{(4)}}{3} + \frac{2g_{140}^{(4)}}{3} + \frac{4g_{141}^{(4)}}{3} + \frac{8g_{142}^{(4)}}{3} + 2g_{147}^{(4)} + \frac{4g_{148}^{(4)}}{3} + 3g_{175}^{(4)} + g_{176}^{(4)} - 3g_{177}^{(4)} \\
&\quad + 3g_{178}^{(4)} + g_{180}^{(4)} - g_{183}^{(4)} + 4g_{190}^{(4)} + 4g_{193}^{(4)} + \frac{g_{69}^{(4)}}{108} + \frac{5g_{74}^{(4)}}{18} + \frac{2g_{75}^{(4)}}{3} + \frac{g_{76}^{(4)}}{3} \\
&\quad - \frac{g_{78}^{(4)}}{2} + \frac{g_{80}^{(4)}}{3} + \frac{4g_{81}^{(4)}}{9} - \frac{\eta_{10}^{(3)}}{36} - \frac{5\eta_{11}^{(3)}}{36} - \frac{\eta_{185}^{(3)}}{6} - \eta_{290}^{(3)} + \frac{7\eta_{44}^{(3)}}{24} - \frac{\eta_{68}^{(3)}}{18} - \frac{\eta_{69}^{(3)}}{9} \\
&\quad - \frac{4\eta_7^{(3)}}{27} + \frac{\eta_{70}^{(3)}}{9} - \frac{\eta_{71}^{(3)}}{9} - \frac{\eta_{72}^{(3)}}{9} + \frac{\eta_{73}^{(3)}}{18} - \frac{\eta_{74}^{(3)}}{18} - \frac{2\eta_8^{(3)}}{9} + \frac{2\eta_{80}^{(3)}}{9} + \frac{2\eta_{83}^{(3)}}{9} - \frac{119}{4} \\
\eta_{293}^{(3)} &= \frac{g_{117}^{(4)}}{24} - \frac{g_{126}^{(4)}}{6} - \frac{g_{130}^{(4)}}{6} - \frac{g_{131}^{(4)}}{6} + \frac{g_{134}^{(4)}}{3} - \frac{g_{136}^{(4)}}{2} - \frac{2g_{139}^{(4)}}{3} - \frac{g_{140}^{(4)}}{3} + \frac{g_{144}^{(4)}}{6} - \frac{g_{146}^{(4)}}{6} - \frac{g_{147}^{(4)}}{3} \\
&\quad - \frac{g_{174}^{(4)}}{2} - g_{175}^{(4)} + g_{177}^{(4)} - g_{178}^{(4)} + g_{191}^{(4)} + g_{192}^{(4)} - g_{193}^{(4)} + \frac{g_{69}^{(4)}}{144} - \frac{g_{74}^{(4)}}{36} - \frac{2g_{75}^{(4)}}{9} - \frac{g_{76}^{(4)}}{9} + \frac{5g_{78}^{(4)}}{36} \\
&\quad - \frac{g_{80}^{(4)}}{18} - \frac{g_{81}^{(4)}}{12} + \frac{\eta_{10}^{(3)}}{72} + \frac{\eta_{11}^{(3)}}{72} - \frac{\eta_{187}^{(3)}}{12} - \frac{\eta_{188}^{(3)}}{12} + \frac{\eta_{218}^{(3)}}{12} - \frac{\eta_{44}^{(3)}}{144} + \frac{\eta_{60}^{(3)}}{72} - \frac{\eta_{61}^{(3)}}{72} + \frac{\eta_{68}^{(3)}}{72} + \frac{\eta_{69}^{(3)}}{24} \\
&\quad + \frac{\eta_7^{(3)}}{36} - \frac{\eta_{70}^{(3)}}{72} + \frac{\eta_{71}^{(3)}}{24} + \frac{\eta_{72}^{(3)}}{24} - \frac{\eta_{73}^{(3)}}{72} + \frac{\eta_{74}^{(3)}}{72} - \frac{\eta_{77}^{(3)}}{9} + \frac{\eta_8^{(3)}}{18} - \frac{\eta_{83}^{(3)}}{36} - \frac{\eta_{84}^{(3)}}{36} + \frac{\eta_{85}^{(3)}}{36} + \frac{223}{36}
\end{aligned}$$

$$\begin{aligned}
\eta_{294}^{(3)} &= \frac{\mathfrak{g}_{117}^{(4)}}{6} + \frac{\mathfrak{g}_{120}^{(4)}}{12} - \frac{\mathfrak{g}_{122}^{(4)}}{12} - \frac{\mathfrak{g}_{131}^{(4)}}{12} - \frac{\mathfrak{g}_{135}^{(4)}}{6} - \frac{\mathfrak{g}_{137}^{(4)}}{6} - \frac{\mathfrak{g}_{142}^{(4)}}{3} - \frac{\mathfrak{g}_{144}^{(4)}}{6} + \frac{\mathfrak{g}_{145}^{(4)}}{6} - \frac{\mathfrak{g}_{147}^{(4)}}{6} \\
&\quad - \frac{\mathfrak{g}_{148}^{(4)}}{6} + \frac{\mathfrak{g}_{169}^{(4)}}{2} - \frac{\mathfrak{g}_{184}^{(4)}}{2} - 2\mathfrak{g}_{190}^{(4)} - \mathfrak{g}_{191}^{(4)} - \mathfrak{g}_{193}^{(4)} - \frac{\mathfrak{g}_{74}^{(4)}}{36} - \frac{\mathfrak{g}_{76}^{(4)}}{18} + \frac{\mathfrak{g}_{78}^{(4)}}{12} + \frac{\eta_{10}^{(3)}}{216} \\
&\quad + \frac{\eta_{11}^{(3)}}{72} - \frac{\eta_{205}^{(3)}}{6} - \frac{\eta_{44}^{(3)}}{36} - \frac{\eta_{60}^{(3)}}{72} + \frac{\eta_{61}^{(3)}}{72} - \frac{\eta_{77}^{(3)}}{18} + \frac{\eta_{83}^{(3)}}{36} + \frac{\eta_{84}^{(3)}}{36} - \frac{\eta_{85}^{(3)}}{36} + \frac{7}{16} \\
\eta_{295}^{(3)} &= \frac{\mathfrak{g}_{117}^{(4)}}{24} - \frac{\mathfrak{g}_{126}^{(4)}}{12} - \frac{2\mathfrak{g}_{136}^{(4)}}{3} - \mathfrak{g}_{139}^{(4)} - \frac{\mathfrak{g}_{140}^{(4)}}{3} - \frac{\mathfrak{g}_{144}^{(4)}}{3} + \frac{\mathfrak{g}_{146}^{(4)}}{3} - \frac{2\mathfrak{g}_{147}^{(4)}}{3} - \frac{\mathfrak{g}_{175}^{(4)}}{2} - 4\mathfrak{g}_{185}^{(4)} - 2\mathfrak{g}_{187}^{(4)} \\
&\quad + 2\mathfrak{g}_{188}^{(4)} + \frac{\mathfrak{g}_{69}^{(4)}}{216} - \frac{\mathfrak{g}_{74}^{(4)}}{18} - \frac{2\mathfrak{g}_{75}^{(4)}}{9} - \frac{\mathfrak{g}_{76}^{(4)}}{9} + \frac{\mathfrak{g}_{78}^{(4)}}{6} - \frac{\mathfrak{g}_{80}^{(4)}}{18} - \frac{\mathfrak{g}_{81}^{(4)}}{9} + \frac{\eta_{10}^{(3)}}{108} + \frac{\eta_{11}^{(3)}}{36} - \frac{\eta_{203}^{(3)}}{6} \\
&\quad - \frac{\eta_{44}^{(3)}}{72} - \frac{\eta_{60}^{(3)}}{36} - \frac{\eta_{61}^{(3)}}{36} + \frac{\eta_{69}^{(3)}}{36} + \frac{\eta_7^{(3)}}{27} - \frac{\eta_{70}^{(3)}}{36} + \frac{\eta_{72}^{(3)}}{36} + \frac{\eta_8^{(3)}}{18} + \frac{\eta_{83}^{(3)}}{18} + \frac{\eta_{84}^{(3)}}{18} - \frac{\eta_{85}^{(3)}}{18} + \frac{449}{72} \\
\eta_{296}^{(3)} &= \frac{\mathfrak{g}_{117}^{(4)}}{12} - \frac{\mathfrak{g}_{126}^{(4)}}{6} - \frac{2\mathfrak{g}_{136}^{(4)}}{3} - \frac{2\mathfrak{g}_{137}^{(4)}}{3} - \frac{4\mathfrak{g}_{139}^{(4)}}{3} - \frac{4\mathfrak{g}_{142}^{(4)}}{3} + \frac{2\mathfrak{g}_{145}^{(4)}}{3} - \frac{2\mathfrak{g}_{146}^{(4)}}{3} - \frac{2\mathfrak{g}_{147}^{(4)}}{3} - \frac{2\mathfrak{g}_{148}^{(4)}}{3} - \mathfrak{g}_{175}^{(4)} \\
&\quad - \mathfrak{g}_{176}^{(4)} + \mathfrak{g}_{177}^{(4)} - \mathfrak{g}_{178}^{(4)} + \mathfrak{g}_{179}^{(4)} - \mathfrak{g}_{180}^{(4)} - 4\mathfrak{g}_{195}^{(4)} - 4\mathfrak{g}_{197}^{(4)} + \frac{\mathfrak{g}_{69}^{(4)}}{54} - \frac{\mathfrak{g}_{74}^{(4)}}{18} - \frac{\mathfrak{g}_{75}^{(4)}}{3} - \frac{\mathfrak{g}_{76}^{(4)}}{18} + \frac{\mathfrak{g}_{78}^{(4)}}{18} \\
&\quad - \frac{\mathfrak{g}_{81}^{(4)}}{9} + \frac{\eta_{10}^{(3)}}{108} + \frac{\eta_{11}^{(3)}}{36} - \frac{\eta_{202}^{(3)}}{6} - \frac{\eta_{44}^{(3)}}{72} + \frac{\eta_{68}^{(3)}}{36} + \frac{\eta_{69}^{(3)}}{36} + \frac{\eta_7^{(3)}}{27} - \frac{\eta_{70}^{(3)}}{36} + \frac{\eta_{72}^{(3)}}{36} + \frac{\eta_8^{(3)}}{18} + \frac{533}{72} \\
\eta_{297}^{(3)} &= -\frac{\mathfrak{g}_{117}^{(4)}}{12} - \frac{\mathfrak{g}_{136}^{(4)}}{4} - \frac{\mathfrak{g}_{137}^{(4)}}{6} - \frac{\mathfrak{g}_{139}^{(4)}}{2} - \frac{\mathfrak{g}_{142}^{(4)}}{3} - \frac{\mathfrak{g}_{144}^{(4)}}{6} + \frac{\mathfrak{g}_{145}^{(4)}}{6} - \frac{\mathfrak{g}_{147}^{(4)}}{6} - \frac{\mathfrak{g}_{148}^{(4)}}{6} \\
&\quad - 2\mathfrak{g}_{185}^{(4)} - \mathfrak{g}_{186}^{(4)} - \mathfrak{g}_{195}^{(4)} - \mathfrak{g}_{197}^{(4)} + \frac{\mathfrak{g}_{69}^{(4)}}{288} - \frac{\mathfrak{g}_{74}^{(4)}}{36} - \frac{\mathfrak{g}_{75}^{(4)}}{12} - \frac{\mathfrak{g}_{76}^{(4)}}{36} + \frac{\mathfrak{g}_{78}^{(4)}}{18} - \frac{\mathfrak{g}_{81}^{(4)}}{24} \\
&\quad + \frac{\eta_{11}^{(3)}}{72} - \frac{\eta_{204}^{(3)}}{6} + \frac{\eta_{44}^{(3)}}{72} - \frac{\eta_{60}^{(3)}}{72} - \frac{\eta_{61}^{(3)}}{72} + \frac{\eta_7^{(3)}}{72} + \frac{\eta_8^{(3)}}{72} + \frac{\eta_{84}^{(3)}}{36} - \frac{\eta_{85}^{(3)}}{36} + \frac{265}{144} \\
\eta_{298}^{(3)} &= -\frac{\mathfrak{g}_{117}^{(4)}}{12} + \frac{\mathfrak{g}_{131}^{(4)}}{12} + \frac{\mathfrak{g}_{134}^{(4)}}{24} + \frac{\mathfrak{g}_{135}^{(4)}}{8} - \frac{\mathfrak{g}_{136}^{(4)}}{12} - \frac{\mathfrak{g}_{139}^{(4)}}{6} + \frac{\mathfrak{g}_{184}^{(4)}}{2} - \mathfrak{g}_{185}^{(4)} - \frac{\mathfrak{g}_{187}^{(4)}}{2} \\
&\quad + \frac{\mathfrak{g}_{188}^{(4)}}{2} + \frac{\mathfrak{g}_{191}^{(4)}}{2} + \frac{\mathfrak{g}_{192}^{(4)}}{2} - \frac{\mathfrak{g}_{193}^{(4)}}{2} + \frac{\mathfrak{g}_{69}^{(4)}}{864} + \frac{\mathfrak{g}_{74}^{(4)}}{144} - \frac{\mathfrak{g}_{75}^{(4)}}{36} + \frac{\mathfrak{g}_{76}^{(4)}}{72} - \frac{\mathfrak{g}_{78}^{(4)}}{144} \\
&\quad - \frac{\mathfrak{g}_{81}^{(4)}}{72} - \frac{\eta_{10}^{(3)}}{288} - \frac{\eta_{11}^{(3)}}{288} + \frac{\eta_{44}^{(3)}}{72} - \frac{\eta_{61}^{(3)}}{72} + \frac{\eta_7^{(3)}}{216} + \frac{\eta_{77}^{(3)}}{36} + \frac{\eta_8^{(3)}}{216} + \frac{43}{48} \\
\eta_{299}^{(3)} &= \frac{\mathfrak{g}_{117}^{(4)}}{12} + \frac{\mathfrak{g}_{120}^{(4)}}{12} - \frac{\mathfrak{g}_{122}^{(4)}}{12} + \frac{\mathfrak{g}_{134}^{(4)}}{24} - \frac{\mathfrak{g}_{135}^{(4)}}{24} - \frac{\mathfrak{g}_{136}^{(4)}}{12} - \frac{\mathfrak{g}_{137}^{(4)}}{6} - \frac{\mathfrak{g}_{139}^{(4)}}{6} - \frac{\mathfrak{g}_{142}^{(4)}}{3} - \frac{\mathfrak{g}_{144}^{(4)}}{12} \\
&\quad + \frac{\mathfrak{g}_{145}^{(4)}}{6} - \frac{\mathfrak{g}_{146}^{(4)}}{12} - \frac{\mathfrak{g}_{147}^{(4)}}{6} - \frac{\mathfrak{g}_{148}^{(4)}}{6} + \frac{\mathfrak{g}_{169}^{(4)}}{2} - \mathfrak{g}_{190}^{(4)} - \frac{\mathfrak{g}_{191}^{(4)}}{2} + \frac{\mathfrak{g}_{192}^{(4)}}{2} - \frac{\mathfrak{g}_{193}^{(4)}}{2} - \mathfrak{g}_{195}^{(4)} \\
&\quad - \mathfrak{g}_{197}^{(4)} + \frac{\mathfrak{g}_{69}^{(4)}}{864} - \frac{\mathfrak{g}_{74}^{(4)}}{48} - \frac{\mathfrak{g}_{75}^{(4)}}{36} - \frac{\mathfrak{g}_{76}^{(4)}}{36} + \frac{7\mathfrak{g}_{78}^{(4)}}{144} - \frac{\mathfrak{g}_{81}^{(4)}}{72} + \frac{\eta_{10}^{(3)}}{864} + \frac{\eta_{11}^{(3)}}{96} - \frac{\eta_{205}^{(3)}}{6} \\
&\quad - \frac{\eta_{44}^{(3)}}{72} - \frac{\eta_{60}^{(3)}}{144} + \frac{\eta_{61}^{(3)}}{144} + \frac{\eta_7^{(3)}}{216} - \frac{\eta_{77}^{(3)}}{36} + \frac{\eta_8^{(3)}}{216} + \frac{\eta_{83}^{(3)}}{72} + \frac{\eta_{84}^{(3)}}{72} - \frac{\eta_{85}^{(3)}}{72} + \frac{47}{36}
\end{aligned}$$

$$\begin{aligned}
\eta_{300}^{(3)} &= \frac{7g_{117}^{(4)}}{24} + \frac{g_{126}^{(4)}}{4} + \frac{g_{130}^{(4)}}{3} - \frac{2g_{134}^{(4)}}{3} - \frac{2g_{135}^{(4)}}{3} + 2g_{136}^{(4)} + \frac{7g_{139}^{(4)}}{3} + \frac{5g_{140}^{(4)}}{3} + \frac{4g_{147}^{(4)}}{3} \\
&\quad + \frac{3g_{175}^{(4)}}{2} - 2g_{177}^{(4)} + 2g_{178}^{(4)} + 8g_{185}^{(4)} + 4g_{187}^{(4)} - 4g_{188}^{(4)} - 4g_{191}^{(4)} - 4g_{192}^{(4)} + 4g_{193}^{(4)} + \frac{g_{69}^{(4)}}{216} \\
&\quad + \frac{g_{74}^{(4)}}{9} + \frac{5g_{75}^{(4)}}{9} + \frac{2g_{76}^{(4)}}{9} - \frac{g_{78}^{(4)}}{3} + \frac{5g_{80}^{(4)}}{18} + \frac{g_{81}^{(4)}}{3} - \frac{\eta_{10}^{(3)}}{54} - \frac{\eta_{11}^{(3)}}{18} - \frac{\eta_{203}^{(3)}}{6} - \frac{\eta_{218}^{(3)}}{6} \\
&\quad - \frac{\eta_{44}^{(3)}}{36} + \frac{\eta_{61}^{(3)}}{9} + \frac{\eta_{68}^{(3)}}{36} - \frac{\eta_{69}^{(3)}}{9} - \frac{\eta_7^{(3)}}{9} - \frac{\eta_{71}^{(3)}}{18} - \frac{\eta_{72}^{(3)}}{9} + \frac{\eta_{73}^{(3)}}{18} - \frac{\eta_{74}^{(3)}}{18} - \frac{5\eta_8^{(3)}}{27} - \frac{787}{36} \\
\eta_{301}^{(3)} &= -\frac{g_{117}^{(4)}}{6} + \frac{g_{136}^{(4)}}{2} + \frac{g_{137}^{(4)}}{3} - \frac{g_{138}^{(4)}}{3} + \frac{2g_{139}^{(4)}}{3} + \frac{g_{141}^{(4)}}{3} + \frac{2g_{142}^{(4)}}{3} + \frac{g_{144}^{(4)}}{6} - \frac{g_{146}^{(4)}}{6} + \frac{g_{147}^{(4)}}{3} + \frac{g_{148}^{(4)}}{3} \\
&\quad + 2g_{185}^{(4)} + g_{186}^{(4)} + g_{187}^{(4)} + g_{190}^{(4)} + g_{193}^{(4)} + \frac{g_{69}^{(4)}}{144} + \frac{g_{74}^{(4)}}{18} + \frac{g_{75}^{(4)}}{18} + \frac{g_{76}^{(4)}}{36} - \frac{g_{78}^{(4)}}{18} + \frac{g_{80}^{(4)}}{18} \\
&\quad + \frac{g_{81}^{(4)}}{12} - \frac{\eta_{11}^{(3)}}{36} + \frac{\eta_{44}^{(3)}}{36} + \frac{\eta_{60}^{(3)}}{72} + \frac{\eta_{61}^{(3)}}{72} - \frac{\eta_7^{(3)}}{36} - \frac{\eta_8^{(3)}}{36} + \frac{\eta_{80}^{(3)}}{18} + \frac{\eta_{83}^{(3)}}{36} - \frac{\eta_{84}^{(3)}}{36} + \frac{\eta_{85}^{(3)}}{36} - \frac{605}{144} \\
\eta_{302}^{(3)} &= \frac{7g_{117}^{(4)}}{24} - \frac{g_{126}^{(4)}}{3} + \frac{g_{129}^{(4)}}{12} - \frac{g_{130}^{(4)}}{3} - \frac{g_{131}^{(4)}}{6} + \frac{g_{134}^{(4)}}{3} + \frac{g_{135}^{(4)}}{3} - g_{136}^{(4)} - \frac{4g_{139}^{(4)}}{3} - \frac{2g_{140}^{(4)}}{3} + \frac{g_{144}^{(4)}}{3} \\
&\quad - \frac{g_{146}^{(4)}}{3} - \frac{2g_{147}^{(4)}}{3} - 2g_{175}^{(4)} + 2g_{177}^{(4)} - 2g_{178}^{(4)} + \frac{g_{183}^{(4)}}{2} + 2g_{191}^{(4)} + 2g_{192}^{(4)} - 2g_{193}^{(4)} - 2g_{194}^{(4)} + \frac{g_{69}^{(4)}}{72} \\
&\quad - \frac{g_{74}^{(4)}}{18} - \frac{4g_{75}^{(4)}}{9} - \frac{g_{76}^{(4)}}{6} + \frac{2g_{78}^{(4)}}{9} - \frac{g_{80}^{(4)}}{9} - \frac{g_{81}^{(4)}}{6} + \frac{\eta_{10}^{(3)}}{54} + \frac{\eta_{11}^{(3)}}{36} - \frac{\eta_{193}^{(3)}}{12} - \frac{\eta_{44}^{(3)}}{18} + \frac{\eta_{60}^{(3)}}{36} - \frac{\eta_{61}^{(3)}}{36} \\
&\quad + \frac{\eta_{68}^{(3)}}{36} + \frac{\eta_{69}^{(3)}}{12} + \frac{\eta_7^{(3)}}{18} - \frac{\eta_{70}^{(3)}}{18} + \frac{5\eta_{71}^{(3)}}{72} + \frac{\eta_{72}^{(3)}}{12} - \frac{\eta_{73}^{(3)}}{24} + \frac{\eta_{74}^{(3)}}{24} + \frac{\eta_8^{(3)}}{9} - \frac{\eta_{83}^{(3)}}{18} - \frac{\eta_{84}^{(3)}}{18} + \frac{\eta_{85}^{(3)}}{18} \\
&\quad + \frac{833}{72} \\
\eta_{303}^{(3)} &= -\frac{g_{117}^{(4)}}{6} - \frac{g_{131}^{(4)}}{12} + \frac{g_{136}^{(4)}}{6} + \frac{g_{137}^{(4)}}{6} - \frac{g_{138}^{(4)}}{6} + \frac{g_{139}^{(4)}}{6} + \frac{g_{141}^{(4)}}{6} + \frac{g_{142}^{(4)}}{3} + \frac{g_{144}^{(4)}}{12} - \frac{g_{146}^{(4)}}{12} + \frac{g_{147}^{(4)}}{6} \\
&\quad + \frac{g_{148}^{(4)}}{6} + g_{190}^{(4)} + \frac{g_{191}^{(4)}}{2} + \frac{g_{192}^{(4)}}{2} + \frac{g_{193}^{(4)}}{2} - g_{194}^{(4)} + \frac{g_{69}^{(4)}}{216} + \frac{g_{74}^{(4)}}{36} + \frac{g_{76}^{(4)}}{72} - \frac{g_{78}^{(4)}}{36} + \frac{g_{80}^{(4)}}{36} + \frac{g_{81}^{(4)}}{36} \\
&\quad - \frac{\eta_{11}^{(3)}}{72} - \frac{\eta_{194}^{(3)}}{12} + \frac{\eta_{44}^{(3)}}{36} + \frac{\eta_{60}^{(3)}}{144} - \frac{\eta_{61}^{(3)}}{144} - \frac{\eta_7^{(3)}}{108} - \frac{\eta_8^{(3)}}{108} + \frac{\eta_{80}^{(3)}}{36} + \frac{\eta_{83}^{(3)}}{72} - \frac{\eta_{84}^{(3)}}{72} + \frac{\eta_{85}^{(3)}}{72} - \frac{425}{288} \\
q_1^{(2)} &= -24g_{55}^{(4)} \\
q_2^{(2)} &= -216g_{111}^{(4)} - 3456g_{114}^{(4)} + 24g_{55}^{(4)} - 36g_{56}^{(4)} + 144g_{57}^{(4)} - 1728\eta_{132}^{(3)} + 72\eta_{40}^{(3)} \\
q_4^{(2)} &= -\frac{12g_{55}^{(4)}}{11} + \frac{36g_{58}^{(4)}}{11} + 72g_{59}^{(4)} - \frac{q_3^{(2)}}{22} \\
q_5^{(2)} &= -\frac{24g_{55}^{(4)}}{11} + \frac{72g_{58}^{(4)}}{11} + 144g_{59}^{(4)} - \frac{q_3^{(2)}}{11} + 24 \\
q_6^{(2)} &= -72g_{111}^{(4)} + 72g_{62}^{(4)} + 576\eta_{132}^{(3)} + 24\eta_{40}^{(3)} - 576\eta_{43}^{(3)} \\
q_7^{(2)} &= -36g_{111}^{(4)} + 72g_{63}^{(4)} + 288\eta_{132}^{(3)} + 12\eta_{40}^{(3)} - 288\eta_{43}^{(3)} \\
q_8^{(2)} &= 54g_{111}^{(4)} + 864g_{114}^{(4)} + 9g_{56}^{(4)} - 18g_{57}^{(4)} + 72g_{65}^{(4)} + 432\eta_{132}^{(3)} - 18\eta_{40}^{(3)} \\
q_9^{(2)} &= 18g_{111}^{(4)} + 288g_{114}^{(4)} + 3g_{56}^{(4)} - 6g_{57}^{(4)} + 72g_{64}^{(4)} + 144\eta_{132}^{(3)} - 6\eta_{40}^{(3)} \\
q_{11}^{(2)} &= \frac{3g_{111}^{(4)}}{11} + \frac{36g_{66}^{(4)}}{11} - \frac{q_{10}^{(2)}}{22} - \frac{24\eta_{132}^{(3)}}{11} - \frac{\eta_{40}^{(3)}}{11} + \frac{24\eta_{43}^{(3)}}{11} + \frac{26}{11}
\end{aligned}$$

$$\begin{aligned}
q_{12}^{(2)} &= \frac{6g_{111}^{(4)}}{11} + \frac{72g_{66}^{(4)}}{11} - \frac{q_{10}^{(2)}}{11} - \frac{48\eta_{132}^{(3)}}{11} - \frac{2\eta_{40}^{(3)}}{11} + \frac{48\eta_{43}^{(3)}}{11} + \frac{8}{11} \\
q_{13}^{(2)} &= 216g_{67}^{(4)} \\
q_{14}^{(2)} &= 18g_{111}^{(4)} + 3g_{56}^{(4)} - 6g_{57}^{(4)} - 72g_{67}^{(4)} + 72g_{68}^{(4)} - 144\eta_{132}^{(3)} - 6\eta_{40}^{(3)} + 144\eta_{43}^{(3)} \\
q_{15}^{(2)} &= -288g_{114}^{(4)} + 72g_{67}^{(4)} + 144g_{68}^{(4)} - 288\eta_{132}^{(3)} + 144\eta_{43}^{(3)} \\
q_{19}^{(2)} &= 36g_{110}^{(4)} \\
q_{20}^{(2)} &= 12\eta_{40}^{(3)} - 288\eta_{132}^{(3)} \\
q_{21}^{(2)} &= 72g_{112}^{(4)} - 48\eta_{132}^{(3)} - \frac{31}{2} \\
q_{22}^{(2)} &= 144g_{113}^{(4)} - 48g_{114}^{(4)} + 12 \\
q_{23}^{(2)} &= 24\eta_{132}^{(3)} - 12\eta_{43}^{(3)} \\
q_{24}^{(2)} &= 72g_{158}^{(4)} \\
q_{25}^{(2)} &= 72g_{111}^{(4)} + 1152g_{114}^{(4)} + 72g_{159}^{(4)} + 12g_{56}^{(4)} - 24g_{57}^{(4)} + 576\eta_{132}^{(3)} - 24\eta_{40}^{(3)} - 144 \\
q_{26}^{(2)} &= 144g_{111}^{(4)} + 72g_{117}^{(4)} + 72g_{160}^{(4)} + 1152\eta_{132}^{(3)} - 48\eta_{40}^{(3)} - 12\eta_{44}^{(3)} + 492 \\
q_{27}^{(2)} &= 12g_{111}^{(4)} + 6g_{117}^{(4)} + 12\eta_{128}^{(3)} - 96\eta_{132}^{(3)} - 4\eta_{40}^{(3)} + 96\eta_{43}^{(3)} - \eta_{44}^{(3)} \\
q_{28}^{(2)} &= 24g_{111}^{(4)} + 12g_{117}^{(4)} + 12\eta_{131}^{(3)} - 192\eta_{132}^{(3)} - 8\eta_{40}^{(3)} + 192\eta_{43}^{(3)} - 2\eta_{44}^{(3)} \\
q_{29}^{(2)} &= -24g_{112}^{(4)} + 16\eta_{132}^{(3)} + \frac{13}{2} \\
q_{30}^{(2)} &= -12g_{112}^{(4)} + 8\eta_{132}^{(3)} + \frac{5}{4} \\
q_{31}^{(2)} &= -48g_{111}^{(4)} - 24g_{117}^{(4)} + 8\eta_{126}^{(3)} - 8\eta_{127}^{(3)} - 384\eta_{132}^{(3)} + 24\eta_{224}^{(3)} + 16\eta_{40}^{(3)} + 4\eta_{44}^{(3)} - 160 \\
q_{32}^{(2)} &= 6\eta_{226}^{(3)} \\
q_{33}^{(2)} &= -24g_{111}^{(4)} - 12g_{117}^{(4)} - 12g_{160}^{(4)} + 2\eta_{127}^{(3)} - 192\eta_{132}^{(3)} + 8\eta_{40}^{(3)} + 2\eta_{44}^{(3)} - 66
\end{aligned}$$

## 2.2 Extra conditions for symmetric $T_{IJ}$

There are another 10 conditions arising from requiring a symmetric  $T_{IJ}$ :

$$\begin{aligned}
\eta_{50}^{(3)} &= -\frac{9}{4} \\
\eta_{296}^{(3)} &= -\frac{g_{139}^{(4)}}{3} + \frac{g_{141}^{(4)}}{3} + \frac{2g_{155}^{(4)}}{3} - \frac{2g_{156}^{(4)}}{3} + \frac{g_{179}^{(4)}}{2} - \frac{3g_{181}^{(4)}}{2} + \frac{3g_{182}^{(4)}}{2} - \frac{g_{183}^{(4)}}{4} + g_{192}^{(4)} + 2g_{193}^{(4)} \\
&\quad - g_{195}^{(4)} - 3g_{196}^{(4)} - g_{197}^{(4)} + 6g_{198}^{(4)} - g_{94}^{(4)} + g_{95}^{(4)} - \frac{3\eta_{100}^{(3)}}{8} + \frac{3\eta_{102}^{(3)}}{8} + \frac{\eta_{105}^{(3)}}{16} - \frac{\eta_{106}^{(3)}}{16} \\
&\quad + \frac{\eta_{112}^{(3)}}{9} + \frac{\eta_{114}^{(3)}}{4} - \frac{\eta_{115}^{(3)}}{9} + \frac{35\eta_{117}^{(3)}}{36} - \frac{11\eta_{118}^{(3)}}{9} - 2\eta_{120}^{(3)} + \eta_{121}^{(3)} - \frac{\eta_{163}^{(3)}}{4} + \frac{\eta_{165}^{(3)}}{4} - \frac{\eta_{19}^{(3)}}{12} \\
&\quad - \frac{\eta_{194}^{(3)}}{12} + \frac{\eta_{198}^{(3)}}{6} + \frac{\eta_{201}^{(3)}}{6} - \frac{\eta_{202}^{(3)}}{12} + \frac{\eta_{203}^{(3)}}{24} + \frac{\eta_{205}^{(3)}}{6} - \frac{\eta_{210}^{(3)}}{24} + \frac{\eta_{211}^{(3)}}{24} + \frac{\eta_{214}^{(3)}}{4} - \frac{\eta_{215}^{(3)}}{3} - \frac{\eta_{216}^{(3)}}{4} \\
&\quad - \frac{\eta_{219}^{(3)}}{12} + \frac{\eta_{220}^{(3)}}{24} - \frac{\eta_{221}^{(3)}}{4} + \frac{\eta_{222}^{(3)}}{6} - \frac{\eta_{223}^{(3)}}{3} + \frac{\eta_{24}^{(3)}}{12} - \frac{\eta_{279}^{(3)}}{2} + \frac{3\eta_{286}^{(3)}}{4} - \frac{\eta_{290}^{(3)}}{4} - \frac{\eta_{292}^{(3)}}{4} + \eta_{294}^{(3)} \\
&\quad + \frac{\eta_{295}^{(3)}}{2} + \frac{\eta_{77}^{(3)}}{36} + \frac{\eta_{78}^{(3)}}{36} + \frac{\eta_{80}^{(3)}}{72} - \frac{\eta_{81}^{(3)}}{24} - \frac{\eta_{82}^{(3)}}{72} - \frac{\eta_{83}^{(3)}}{36} - \frac{\eta_{85}^{(3)}}{72} + \frac{\eta_{86}^{(3)}}{72} + \frac{\eta_{94}^{(3)}}{4} + \frac{535}{288}
\end{aligned}$$

$$\begin{aligned}
\eta_{297}^{(3)} = & -\frac{g_{139}^{(4)}}{6} + \frac{g_{141}^{(4)}}{6} + \frac{g_{155}^{(4)}}{3} - \frac{g_{156}^{(4)}}{3} + \frac{g_{179}^{(4)}}{8} - \frac{3g_{181}^{(4)}}{2} + \frac{3g_{182}^{(4)}}{2} - \frac{g_{183}^{(4)}}{16} - 3g_{190}^{(4)} + \frac{g_{192}^{(4)}}{4} + \frac{g_{193}^{(4)}}{2} \\
& + g_{195}^{(4)} - \frac{3g_{196}^{(4)}}{4} - \frac{g_{197}^{(4)}}{4} + 6g_{198}^{(4)} - \frac{g_{94}^{(4)}}{2} + \frac{g_{95}^{(4)}}{2} - \frac{3\eta_{100}^{(3)}}{8} + \frac{3\eta_{102}^{(3)}}{8} + \frac{\eta_{105}^{(3)}}{64} - \frac{\eta_{106}^{(3)}}{64} + \frac{\eta_{112}^{(3)}}{18} \\
& + \frac{\eta_{114}^{(3)}}{2} - \frac{\eta_{115}^{(3)}}{18} + \frac{79\eta_{117}^{(3)}}{144} - \frac{11\eta_{118}^{(3)}}{18} - \eta_{120}^{(3)} + \frac{\eta_{121}^{(3)}}{2} - \frac{\eta_{162}^{(3)}}{24} - \frac{13\eta_{163}^{(3)}}{48} + \frac{\eta_{165}^{(3)}}{6} - \frac{\eta_{19}^{(3)}}{24} \\
& - \frac{\eta_{194}^{(3)}}{24} - \frac{\eta_{196}^{(3)}}{12} + \frac{\eta_{198}^{(3)}}{6} + \frac{\eta_{201}^{(3)}}{12} - \frac{\eta_{202}^{(3)}}{48} + \frac{\eta_{203}^{(3)}}{96} + \frac{\eta_{205}^{(3)}}{24} + \frac{\eta_{206}^{(3)}}{24} - \frac{\eta_{208}^{(3)}}{12} + \frac{\eta_{209}^{(3)}}{24} - \frac{\eta_{210}^{(3)}}{96} \\
& + \frac{\eta_{211}^{(3)}}{96} - \frac{\eta_{213}^{(3)}}{12} + \frac{\eta_{214}^{(3)}}{4} - \frac{\eta_{215}^{(3)}}{3} - \frac{\eta_{216}^{(3)}}{4} - \frac{\eta_{219}^{(3)}}{8} + \frac{\eta_{220}^{(3)}}{96} + \frac{\eta_{222}^{(3)}}{24} - \frac{\eta_{223}^{(3)}}{3} + \frac{\eta_{24}^{(3)}}{24} - \frac{\eta_{274}^{(3)}}{16} \\
& - \frac{\eta_{275}^{(3)}}{16} + \frac{\eta_{276}^{(3)}}{16} + \frac{\eta_{277}^{(3)}}{8} - \frac{\eta_{279}^{(3)}}{4} + \frac{\eta_{281}^{(3)}}{8} + \frac{\eta_{285}^{(3)}}{8} - \frac{\eta_{286}^{(3)}}{16} - \frac{3\eta_{290}^{(3)}}{16} + \frac{\eta_{291}^{(3)}}{2} - \frac{3\eta_{292}^{(3)}}{16} + \frac{\eta_{294}^{(3)}}{2} \\
& - \frac{\eta_{295}^{(3)}}{8} + \frac{\eta_{77}^{(3)}}{72} + \frac{\eta_{78}^{(3)}}{72} + \frac{\eta_{80}^{(3)}}{144} - \frac{\eta_{81}^{(3)}}{48} - \frac{\eta_{82}^{(3)}}{144} - \frac{\eta_{83}^{(3)}}{72} - \frac{\eta_{85}^{(3)}}{144} + \frac{\eta_{86}^{(3)}}{144} + \frac{9\eta_{94}^{(3)}}{32} - \frac{1}{1152} \\
\eta_{298}^{(3)} = & -\frac{g_{139}^{(4)}}{16} + \frac{g_{141}^{(4)}}{16} + \frac{g_{155}^{(4)}}{8} - \frac{g_{156}^{(4)}}{8} - \frac{15g_{181}^{(4)}}{32} + \frac{15g_{182}^{(4)}}{32} - \frac{3g_{190}^{(4)}}{4} + \frac{3g_{195}^{(4)}}{16} + \frac{15g_{198}^{(4)}}{8} - \frac{3g_{94}^{(4)}}{16} \\
& + \frac{3g_{95}^{(4)}}{16} - \frac{15\eta_{100}^{(3)}}{128} + \frac{15\eta_{102}^{(3)}}{128} + \frac{\eta_{112}^{(3)}}{48} + \frac{9\eta_{114}^{(3)}}{64} - \frac{\eta_{115}^{(3)}}{48} + \frac{11\eta_{117}^{(3)}}{48} - \frac{11\eta_{118}^{(3)}}{48} - \frac{3\eta_{120}^{(3)}}{8} \\
& + \frac{3\eta_{121}^{(3)}}{16} - \frac{\eta_{162}^{(3)}}{96} - \frac{5\eta_{163}^{(3)}}{96} + \frac{\eta_{165}^{(3)}}{64} - \frac{\eta_{19}^{(3)}}{64} - \frac{11\eta_{194}^{(3)}}{192} + \frac{5\eta_{198}^{(3)}}{96} + \frac{5\eta_{201}^{(3)}}{96} - \frac{5\eta_{206}^{(3)}}{96} - \frac{\eta_{208}^{(3)}}{48} \\
& + \frac{5\eta_{209}^{(3)}}{96} + \frac{5\eta_{214}^{(3)}}{64} - \frac{5\eta_{215}^{(3)}}{48} - \frac{5\eta_{216}^{(3)}}{64} - \frac{\eta_{219}^{(3)}}{64} - \frac{\eta_{221}^{(3)}}{64} - \frac{5\eta_{223}^{(3)}}{48} + \frac{\eta_{24}^{(3)}}{64} - \frac{11\eta_{279}^{(3)}}{32} - \frac{\eta_{291}^{(3)}}{8} \\
& + \frac{5\eta_{294}^{(3)}}{16} + \frac{\eta_{77}^{(3)}}{192} + \frac{\eta_{78}^{(3)}}{192} + \frac{\eta_{80}^{(3)}}{384} - \frac{\eta_{81}^{(3)}}{128} - \frac{\eta_{82}^{(3)}}{384} - \frac{\eta_{83}^{(3)}}{192} - \frac{\eta_{85}^{(3)}}{384} + \frac{\eta_{86}^{(3)}}{384} + \frac{9\eta_{94}^{(3)}}{128} + \frac{85}{192} \\
\eta_{299}^{(3)} = & -\frac{g_{139}^{(4)}}{8} + \frac{g_{141}^{(4)}}{8} + \frac{g_{155}^{(4)}}{4} - \frac{g_{156}^{(4)}}{4} + \frac{g_{179}^{(4)}}{8} - \frac{3g_{181}^{(4)}}{16} + \frac{3g_{182}^{(4)}}{16} - \frac{g_{183}^{(4)}}{16} + \frac{3g_{190}^{(4)}}{2} + \frac{g_{192}^{(4)}}{4} + \frac{g_{193}^{(4)}}{2} \\
& - \frac{9g_{195}^{(4)}}{8} - \frac{3g_{196}^{(4)}}{4} - \frac{g_{197}^{(4)}}{4} + \frac{3g_{198}^{(4)}}{4} - \frac{3g_{94}^{(4)}}{8} + \frac{3g_{95}^{(4)}}{8} - \frac{3\eta_{100}^{(3)}}{64} + \frac{3\eta_{102}^{(3)}}{64} + \frac{\eta_{105}^{(3)}}{64} - \frac{\eta_{106}^{(3)}}{64} + \frac{\eta_{112}^{(3)}}{24} \\
& - \frac{3\eta_{114}^{(3)}}{32} - \frac{\eta_{115}^{(3)}}{24} + \frac{19\eta_{117}^{(3)}}{48} - \frac{11\eta_{118}^{(3)}}{24} - \frac{3\eta_{120}^{(3)}}{4} + \frac{3\eta_{121}^{(3)}}{8} - \frac{\eta_{162}^{(3)}}{48} + \frac{\eta_{163}^{(3)}}{12} - \frac{\eta_{165}^{(3)}}{96} - \frac{\eta_{19}^{(3)}}{32} \\
& - \frac{7\eta_{194}^{(3)}}{96} + \frac{\eta_{196}^{(3)}}{12} + \frac{\eta_{198}^{(3)}}{48} + \frac{5\eta_{201}^{(3)}}{48} - \frac{\eta_{202}^{(3)}}{48} + \frac{\eta_{203}^{(3)}}{96} + \frac{\eta_{205}^{(3)}}{24} - \frac{\eta_{206}^{(3)}}{16} - \frac{\eta_{208}^{(3)}}{24} + \frac{\eta_{209}^{(3)}}{16} - \frac{\eta_{210}^{(3)}}{96} \\
& + \frac{\eta_{211}^{(3)}}{96} + \frac{\eta_{213}^{(3)}}{12} + \frac{\eta_{214}^{(3)}}{32} - \frac{\eta_{215}^{(3)}}{24} - \frac{\eta_{216}^{(3)}}{32} - \frac{\eta_{219}^{(3)}}{32} + \frac{\eta_{220}^{(3)}}{96} - \frac{5\eta_{221}^{(3)}}{32} + \frac{\eta_{222}^{(3)}}{24} - \frac{\eta_{223}^{(3)}}{24} + \frac{\eta_{24}^{(3)}}{32} \\
& - \frac{\eta_{274}^{(3)}}{16} - \frac{\eta_{275}^{(3)}}{16} + \frac{\eta_{276}^{(3)}}{16} + \frac{\eta_{277}^{(3)}}{8} - \frac{7\eta_{279}^{(3)}}{16} + \frac{\eta_{281}^{(3)}}{8} + \frac{\eta_{285}^{(3)}}{8} - \frac{\eta_{286}^{(3)}}{16} - \frac{3\eta_{290}^{(3)}}{16} - \frac{\eta_{291}^{(3)}}{4} - \frac{3\eta_{292}^{(3)}}{16} \\
& + \frac{13\eta_{294}^{(3)}}{8} - \frac{\eta_{295}^{(3)}}{8} + \frac{\eta_{77}^{(3)}}{96} + \frac{\eta_{78}^{(3)}}{96} + \frac{\eta_{80}^{(3)}}{192} - \frac{\eta_{81}^{(3)}}{64} - \frac{\eta_{82}^{(3)}}{192} - \frac{\eta_{83}^{(3)}}{96} - \frac{\eta_{85}^{(3)}}{192} + \frac{\eta_{86}^{(3)}}{192} - \frac{\eta_{94}^{(3)}}{64} + \frac{617}{384} \\
\eta_{300}^{(3)} = & \frac{\eta_{203}^{(3)}}{6} - \frac{\eta_{210}^{(3)}}{6} - \frac{\eta_{218}^{(3)}}{6} + \frac{\eta_{220}^{(3)}}{6} + 2\eta_{295}^{(3)}
\end{aligned}$$

$$\begin{aligned}
\eta_{301}^{(3)} = & -\frac{\mathfrak{g}_{139}^{(4)}}{6} + \frac{\mathfrak{g}_{141}^{(4)}}{6} + \frac{\mathfrak{g}_{155}^{(4)}}{3} - \frac{\mathfrak{g}_{156}^{(4)}}{3} - \frac{9\mathfrak{g}_{181}^{(4)}}{4} + \frac{9\mathfrak{g}_{182}^{(4)}}{4} - 6\mathfrak{g}_{190}^{(4)} + \frac{5\mathfrak{g}_{195}^{(4)}}{2} + 9\mathfrak{g}_{198}^{(4)} - \frac{\mathfrak{g}_{94}^{(4)}}{2} \\
& + \frac{\mathfrak{g}_{95}^{(4)}}{2} - \frac{9\eta_{100}^{(3)}}{16} + \frac{9\eta_{102}^{(3)}}{16} + \frac{\eta_{112}^{(3)}}{18} + \frac{7\eta_{114}^{(3)}}{8} - \frac{\eta_{115}^{(3)}}{18} + \frac{11\eta_{117}^{(3)}}{18} - \frac{11\eta_{118}^{(3)}}{18} - \eta_{120}^{(3)} + \frac{\eta_{121}^{(3)}}{2} \\
& - \frac{\eta_{162}^{(3)}}{12} - \frac{5\eta_{163}^{(3)}}{12} + \frac{5\eta_{165}^{(3)}}{24} - \frac{\eta_{19}^{(3)}}{24} - \frac{\eta_{194}^{(3)}}{24} - \frac{\eta_{196}^{(3)}}{6} + \frac{\eta_{198}^{(3)}}{4} + \frac{\eta_{201}^{(3)}}{12} + \frac{\eta_{206}^{(3)}}{12} - \frac{\eta_{208}^{(3)}}{6} + \frac{\eta_{209}^{(3)}}{12} \\
& - \frac{\eta_{213}^{(3)}}{6} + \frac{3\eta_{214}^{(3)}}{8} - \frac{\eta_{215}^{(3)}}{2} - \frac{3\eta_{216}^{(3)}}{8} - \frac{5\eta_{219}^{(3)}}{24} + \frac{\eta_{221}^{(3)}}{8} - \frac{\eta_{223}^{(3)}}{2} + \frac{\eta_{24}^{(3)}}{24} - \frac{\eta_{279}^{(3)}}{4} - \eta_{291}^{(3)} \\
& + \frac{\eta_{294}^{(3)}}{2} + \frac{\eta_{77}^{(3)}}{72} + \frac{\eta_{78}^{(3)}}{72} + \frac{\eta_{80}^{(3)}}{144} - \frac{\eta_{81}^{(3)}}{48} - \frac{\eta_{82}^{(3)}}{144} - \frac{\eta_{83}^{(3)}}{72} - \frac{\eta_{85}^{(3)}}{144} + \frac{\eta_{86}^{(3)}}{144} + \frac{7\eta_{94}^{(3)}}{16} - \frac{19}{18} \\
\eta_{302}^{(3)} = & \frac{11\mathfrak{g}_{139}^{(4)}}{18} - \frac{11\mathfrak{g}_{141}^{(4)}}{18} - \frac{11\mathfrak{g}_{155}^{(4)}}{9} + \frac{11\mathfrak{g}_{156}^{(4)}}{9} - \frac{3\mathfrak{g}_{179}^{(4)}}{4} + \frac{27\mathfrak{g}_{181}^{(4)}}{4} - \frac{27\mathfrak{g}_{182}^{(4)}}{4} + \frac{3\mathfrak{g}_{183}^{(4)}}{8} + 16\mathfrak{g}_{190}^{(4)} \\
& + \frac{5\mathfrak{g}_{192}^{(4)}}{2} + \mathfrak{g}_{193}^{(4)} - 2\mathfrak{g}_{194}^{(4)} - \frac{37\mathfrak{g}_{195}^{(4)}}{6} + \frac{\mathfrak{g}_{196}^{(4)}}{2} - \frac{\mathfrak{g}_{197}^{(4)}}{2} - 27\mathfrak{g}_{198}^{(4)} + \frac{11\mathfrak{g}_{94}^{(4)}}{6} - \frac{11\mathfrak{g}_{95}^{(4)}}{6} + \frac{27\eta_{100}^{(3)}}{16} \\
& - \frac{27\eta_{102}^{(3)}}{16} - \frac{3\eta_{105}^{(3)}}{32} + \frac{3\eta_{106}^{(3)}}{32} + \frac{\eta_{109}^{(3)}}{2} - \frac{11\eta_{112}^{(3)}}{54} - \frac{59\eta_{114}^{(3)}}{24} + \frac{11\eta_{115}^{(3)}}{54} - \frac{511\eta_{117}^{(3)}}{216} + \frac{121\eta_{118}^{(3)}}{54} \\
& + \frac{11\eta_{120}^{(3)}}{3} - \frac{11\eta_{121}^{(3)}}{6} + \frac{\eta_{162}^{(3)}}{18} + \frac{71\eta_{163}^{(3)}}{72} - \frac{37\eta_{165}^{(3)}}{72} + \frac{11\eta_{19}^{(3)}}{72} + \frac{11\eta_{194}^{(3)}}{72} + \frac{\eta_{196}^{(3)}}{3} - \frac{3\eta_{198}^{(3)}}{4} \\
& - \frac{5\eta_{201}^{(3)}}{12} + \frac{\eta_{202}^{(3)}}{8} + \frac{5\eta_{203}^{(3)}}{48} - \frac{17\eta_{205}^{(3)}}{36} - \frac{\eta_{206}^{(3)}}{6} + \frac{\eta_{208}^{(3)}}{9} + \frac{\eta_{209}^{(3)}}{18} - \frac{5\eta_{210}^{(3)}}{48} - \frac{\eta_{211}^{(3)}}{16} + \frac{\eta_{213}^{(3)}}{3} \\
& - \frac{9\eta_{214}^{(3)}}{8} + \frac{3\eta_{215}^{(3)}}{2} + \frac{9\eta_{216}^{(3)}}{8} - \frac{\eta_{218}^{(3)}}{6} + \frac{17\eta_{219}^{(3)}}{24} + \frac{5\eta_{220}^{(3)}}{48} - \frac{11\eta_{221}^{(3)}}{72} - \frac{\eta_{222}^{(3)}}{36} + \frac{3\eta_{223}^{(3)}}{2} \\
& - \frac{11\eta_{24}^{(3)}}{72} + \frac{\eta_{274}^{(3)}}{2} + \frac{\eta_{275}^{(3)}}{2} - \frac{\eta_{276}^{(3)}}{2} + \frac{\eta_{277}^{(3)}}{2} - \eta_{278}^{(3)} + \frac{11\eta_{279}^{(3)}}{12} + \frac{\eta_{281}^{(3)}}{2} - \frac{\eta_{282}^{(3)}}{2} - \frac{\eta_{284}^{(3)}}{2} \\
& - \eta_{285}^{(3)} + \frac{7\eta_{286}^{(3)}}{8} + \frac{3\eta_{290}^{(3)}}{8} + \frac{2\eta_{291}^{(3)}}{3} + \frac{3\eta_{292}^{(3)}}{8} + 2\eta_{293}^{(3)} - \frac{5\eta_{294}^{(3)}}{2} + \frac{5\eta_{295}^{(3)}}{4} - \frac{11\eta_{77}^{(3)}}{216} \\
& - \frac{11\eta_{78}^{(3)}}{216} - \frac{11\eta_{80}^{(3)}}{432} + \frac{11\eta_{81}^{(3)}}{144} + \frac{11\eta_{82}^{(3)}}{432} + \frac{11\eta_{83}^{(3)}}{216} + \frac{11\eta_{85}^{(3)}}{432} - \frac{11\eta_{86}^{(3)}}{432} - \frac{7\eta_{94}^{(3)}}{6} + \frac{1321}{1728} \\
\eta_{303}^{(3)} = & \frac{5\mathfrak{g}_{139}^{(4)}}{36} - \frac{5\mathfrak{g}_{141}^{(4)}}{36} - \frac{5\mathfrak{g}_{155}^{(4)}}{18} + \frac{5\mathfrak{g}_{156}^{(4)}}{18} - \frac{3\mathfrak{g}_{179}^{(4)}}{8} - \frac{3\mathfrak{g}_{181}^{(4)}}{8} + \frac{3\mathfrak{g}_{182}^{(4)}}{8} + \frac{3\mathfrak{g}_{183}^{(4)}}{16} - 4\mathfrak{g}_{190}^{(4)} + \frac{5\mathfrak{g}_{192}^{(4)}}{4} \\
& + \frac{\mathfrak{g}_{193}^{(4)}}{2} - \mathfrak{g}_{194}^{(4)} + \frac{29\mathfrak{g}_{195}^{(4)}}{12} + \frac{\mathfrak{g}_{196}^{(4)}}{4} - \frac{\mathfrak{g}_{197}^{(4)}}{4} + \frac{3\mathfrak{g}_{198}^{(4)}}{2} + \frac{5\mathfrak{g}_{94}^{(4)}}{12} - \frac{5\mathfrak{g}_{95}^{(4)}}{12} - \frac{3\eta_{100}^{(3)}}{32} + \frac{3\eta_{102}^{(3)}}{32} \\
& - \frac{3\eta_{105}^{(3)}}{64} + \frac{3\eta_{106}^{(3)}}{64} + \frac{\eta_{109}^{(3)}}{4} - \frac{5\eta_{112}^{(3)}}{108} + \frac{19\eta_{114}^{(3)}}{48} + \frac{5\eta_{115}^{(3)}}{108} - \frac{247\eta_{117}^{(3)}}{432} + \frac{55\eta_{118}^{(3)}}{108} + \frac{5\eta_{120}^{(3)}}{6} \\
& - \frac{5\eta_{121}^{(3)}}{12} - \frac{\eta_{162}^{(3)}}{18} - \frac{61\eta_{163}^{(3)}}{144} + \frac{29\eta_{165}^{(3)}}{144} + \frac{5\eta_{19}^{(3)}}{144} + \frac{17\eta_{194}^{(3)}}{144} - \frac{\eta_{196}^{(3)}}{4} + \frac{\eta_{198}^{(3)}}{24} - \frac{5\eta_{201}^{(3)}}{24} + \frac{\eta_{202}^{(3)}}{16} \\
& - \frac{\eta_{203}^{(3)}}{32} - \frac{17\eta_{205}^{(3)}}{72} + \frac{\eta_{206}^{(3)}}{6} - \frac{\eta_{208}^{(3)}}{9} + \frac{\eta_{209}^{(3)}}{36} + \frac{\eta_{210}^{(3)}}{32} - \frac{\eta_{211}^{(3)}}{32} - \frac{\eta_{213}^{(3)}}{4} + \frac{\eta_{214}^{(3)}}{16} - \frac{\eta_{215}^{(3)}}{12} - \frac{\eta_{216}^{(3)}}{16} \\
& + \frac{\eta_{219}^{(3)}}{16} - \frac{\eta_{220}^{(3)}}{32} + \frac{43\eta_{221}^{(3)}}{144} - \frac{\eta_{222}^{(3)}}{72} - \frac{\eta_{223}^{(3)}}{12} - \frac{5\eta_{24}^{(3)}}{144} + \frac{3\eta_{274}^{(3)}}{16} + \frac{3\eta_{275}^{(3)}}{16} - \frac{3\eta_{276}^{(3)}}{16} - \frac{3\eta_{277}^{(3)}}{8} \\
& + \frac{17\eta_{279}^{(3)}}{24} - \frac{3\eta_{281}^{(3)}}{8} - \frac{3\eta_{285}^{(3)}}{8} + \frac{3\eta_{286}^{(3)}}{16} + \frac{9\eta_{290}^{(3)}}{16} - \frac{2\eta_{291}^{(3)}}{3} + \frac{9\eta_{292}^{(3)}}{16} - \frac{\eta_{294}^{(3)}}{4} + \frac{3\eta_{295}^{(3)}}{8} \\
& - \frac{5\eta_{77}^{(3)}}{432} - \frac{5\eta_{78}^{(3)}}{432} - \frac{5\eta_{80}^{(3)}}{864} + \frac{5\eta_{81}^{(3)}}{288} + \frac{5\eta_{82}^{(3)}}{864} + \frac{5\eta_{83}^{(3)}}{432} + \frac{5\eta_{85}^{(3)}}{864} - \frac{5\eta_{86}^{(3)}}{864} + \frac{11\eta_{94}^{(3)}}{48} - \frac{12695}{3456}
\end{aligned}$$

$$\mathfrak{q}_{30}^{(2)} = -3$$

### 2.3 Consistency conditions for $S$

From Osborn's equation at order 4-3-2, we find that the  $S$  coefficients must satisfy

$$\begin{aligned} \mathfrak{f}_1^{(3)} &= -\mathfrak{g}_{138}^{(4)} + \frac{\mathfrak{g}_{141}^{(4)}}{2} - 6\mathfrak{g}_{195}^{(4)} + \frac{\mathfrak{g}_{69}^{(4)}}{48} - \frac{\mathfrak{g}_{75}^{(4)}}{6} + \frac{\mathfrak{g}_{80}^{(4)}}{12} - \frac{\mathfrak{g}_{159}^{(3)}}{4} + \frac{\mathfrak{g}_{160}^{(3)}}{4} + \frac{\mathfrak{g}_{59}^{(3)}}{24} + \frac{\mathfrak{g}_{82}^{(3)}}{12} - \frac{25}{48} \\ \mathfrak{f}_2^{(3)} &= -\frac{\mathfrak{g}_{115}^{(4)}}{2} - \mathfrak{g}_{140}^{(4)} + \mathfrak{g}_{141}^{(4)} + \frac{\mathfrak{g}_{159}^{(3)}}{2} + \frac{\mathfrak{g}_{160}^{(3)}}{2} - \frac{\mathfrak{g}_{172}^{(3)}}{4} + \frac{\mathfrak{g}_{173}^{(3)}}{4} + \frac{\mathfrak{g}_{46}^{(3)}}{12} - \frac{\mathfrak{g}_{59}^{(3)}}{12} + \frac{\mathfrak{g}_{80}^{(3)}}{6} - \frac{\mathfrak{g}_{82}^{(3)}}{6} - \frac{27}{8} \\ \mathfrak{f}_4^{(3)} &= \frac{\mathfrak{g}_{115}^{(4)}}{3} + \frac{2\mathfrak{g}_{145}^{(4)}}{3} - \frac{2\mathfrak{g}_{147}^{(4)}}{3} + \mathfrak{g}_{177}^{(4)} - \mathfrak{g}_{178}^{(4)} + \mathfrak{g}_{179}^{(4)} - \frac{\mathfrak{g}_{76}^{(4)}}{9} + \frac{2\mathfrak{g}_{78}^{(4)}}{9} - \frac{2\mathfrak{f}_3^{(3)}}{3} - \frac{\mathfrak{g}_{151}^{(3)}}{12} - \frac{\mathfrak{g}_{159}^{(3)}}{3} \\ &\quad - \frac{\mathfrak{g}_{160}^{(3)}}{3} + \frac{\mathfrak{g}_{184}^{(3)}}{3} - \frac{\mathfrak{g}_{185}^{(3)}}{6} - \frac{\mathfrak{g}_{192}^{(3)}}{6} + \frac{\mathfrak{g}_{264}^{(3)}}{4} - \frac{\mathfrak{g}_{265}^{(3)}}{4} - \frac{\mathfrak{g}_{46}^{(3)}}{18} - \frac{\mathfrak{g}_{60}^{(3)}}{18} + \frac{2\mathfrak{g}_{83}^{(3)}}{9} - \frac{\mathfrak{g}_{85}^{(3)}}{9} + \frac{31}{72} \\ \mathfrak{f}_5^{(3)} &= \frac{\mathfrak{g}_{115}^{(4)}}{6} + \frac{\mathfrak{g}_{138}^{(4)}}{3} - \frac{\mathfrak{g}_{141}^{(4)}}{6} - \frac{\mathfrak{g}_{145}^{(4)}}{6} + \frac{\mathfrak{g}_{146}^{(4)}}{2} - \frac{\mathfrak{g}_{147}^{(4)}}{3} - \mathfrak{g}_{187}^{(4)} + \mathfrak{g}_{188}^{(4)} + 2\mathfrak{g}_{195}^{(4)} + 2\mathfrak{g}_{197}^{(4)} - \frac{\mathfrak{g}_{69}^{(4)}}{144} \\ &\quad + \frac{\mathfrak{g}_{75}^{(4)}}{18} - \frac{\mathfrak{g}_{76}^{(4)}}{18} + \frac{\mathfrak{g}_{78}^{(4)}}{9} - \frac{\mathfrak{g}_{80}^{(4)}}{36} - \frac{\mathfrak{f}_3^{(3)}}{6} - \frac{\mathfrak{g}_{156}^{(3)}}{6} - \frac{\mathfrak{g}_{159}^{(3)}}{12} - \frac{\mathfrak{g}_{160}^{(3)}}{12} + \frac{\mathfrak{g}_{184}^{(3)}}{24} - \frac{\mathfrak{g}_{186}^{(3)}}{24} + \frac{\mathfrak{g}_{204}^{(3)}}{2} \\ &\quad - \frac{\mathfrak{g}_{208}^{(3)}}{6} - \frac{\mathfrak{g}_{213}^{(3)}}{3} - \frac{\mathfrak{g}_{277}^{(3)}}{4} + \frac{\mathfrak{g}_{281}^{(3)}}{4} + 2\mathfrak{g}_{297}^{(3)} - \frac{\mathfrak{g}_{46}^{(3)}}{36} - \frac{\mathfrak{g}_{59}^{(3)}}{72} - \frac{\mathfrak{g}_{60}^{(3)}}{36} - \frac{\mathfrak{g}_{82}^{(3)}}{36} + \frac{\mathfrak{g}_{83}^{(3)}}{9} - \frac{\mathfrak{g}_{85}^{(3)}}{18} + \frac{137}{144} \\ \mathfrak{f}_6^{(3)} &= -\frac{\mathfrak{g}_{115}^{(4)}}{12} - \frac{\mathfrak{g}_{145}^{(4)}}{6} + \frac{\mathfrak{g}_{147}^{(4)}}{6} - \frac{\mathfrak{g}_{177}^{(4)}}{2} + \frac{\mathfrak{g}_{178}^{(4)}}{2} - \frac{\mathfrak{g}_{179}^{(4)}}{2} - \mathfrak{g}_{191}^{(4)} + \mathfrak{g}_{192}^{(4)} + \frac{\mathfrak{g}_{76}^{(4)}}{36} \\ &\quad - \frac{\mathfrak{g}_{78}^{(4)}}{18} + \frac{\mathfrak{f}_3^{(3)}}{6} + \frac{\mathfrak{g}_{151}^{(3)}}{24} + \frac{\mathfrak{g}_{159}^{(3)}}{12} + \frac{\mathfrak{g}_{160}^{(3)}}{12} - \frac{\mathfrak{g}_{163}^{(3)}}{12} - \frac{\mathfrak{g}_{184}^{(3)}}{8} + \frac{\mathfrak{g}_{185}^{(3)}}{12} - \frac{\mathfrak{g}_{186}^{(3)}}{24} \\ &\quad + \frac{\mathfrak{g}_{192}^{(3)}}{12} + \frac{\mathfrak{g}_{219}^{(3)}}{6} - \frac{\mathfrak{g}_{221}^{(3)}}{6} - \frac{\mathfrak{g}_{290}^{(3)}}{4} + \frac{\mathfrak{g}_{292}^{(3)}}{4} + \frac{\mathfrak{g}_{46}^{(3)}}{72} + \frac{\mathfrak{g}_{60}^{(3)}}{72} - \frac{\mathfrak{g}_{83}^{(3)}}{18} + \frac{\mathfrak{g}_{85}^{(3)}}{36} + \frac{25}{144} \\ \mathfrak{s}_1^{(3)} &= \mathfrak{g}_{131}^{(4)} + 3\mathfrak{g}_{174}^{(4)} - \frac{\mathfrak{g}_{187}^{(3)}}{2} + \frac{\mathfrak{g}_{188}^{(3)}}{2} - \frac{7}{4} \\ \mathfrak{s}_2^{(3)} &= 12\mathfrak{g}_{112}^{(4)} + \frac{\mathfrak{q}_{20}^{(2)}}{72} - \frac{\mathfrak{q}_{21}^{(2)}}{12} - \frac{\mathfrak{g}_{231}^{(3)}}{2} + \frac{\mathfrak{g}_{232}^{(3)}}{2} - \frac{\mathfrak{g}_{40}^{(3)}}{6} - \frac{13}{6} \\ \mathfrak{s}_3^{(3)} &= \frac{\mathfrak{g}_{131}^{(4)}}{6} - \frac{\mathfrak{g}_{174}^{(4)}}{2} + \frac{\mathfrak{g}_{178}^{(4)}}{2} - \frac{\mathfrak{g}_{183}^{(4)}}{2} - 2\mathfrak{g}_{191}^{(4)} + 4\mathfrak{g}_{194}^{(4)} - \frac{\mathfrak{g}_{184}^{(3)}}{12} - \frac{\mathfrak{g}_{186}^{(3)}}{12} \\ &\quad + \frac{\mathfrak{g}_{187}^{(3)}}{12} + \frac{\mathfrak{g}_{188}^{(3)}}{12} + \frac{\mathfrak{g}_{194}^{(3)}}{3} + \frac{\mathfrak{g}_{219}^{(3)}}{3} + \mathfrak{g}_{284}^{(3)} - \frac{\mathfrak{g}_{290}^{(3)}}{2} - \frac{\mathfrak{g}_{292}^{(3)}}{2} + 4\mathfrak{g}_{303}^{(3)} - \frac{3}{4} \end{aligned}$$
